# Supplementary material for: Sketch Decompositions for Classical Planning via Deep Reinforcement Learning
Source: arXiv:2412.08574 source file (2025-08-15)
Supplement: Supplementary file 1 [file grid.tex]

\lstset{
    basicstyle=\footnotesize\ttfamily,
    keywordstyle=\bfseries, % This will apply bold to all keywords
    % Define colors for different groups of keywords
    morekeywords=[1]{Domain},
    keywordstyle=[1]\color{red}\bfseries,
    morekeywords=[2]{Objects, Primitive, Goal, Initial, Plan, plan},
    keywordstyle=[2]\bfseries,
    morekeywords=[3]{putdown, move, pickup, and, loose, unlock, pickup },
    keywordstyle=[3]\color{orange}\bfseries,
    morekeywords=[4]{f0-2f, f0-0f, key1-0, shape0, key1-3, key1-2, shape1, key1-4, shape2, f0-1f, key1-1 },
    keywordstyle=[4]\color{blue}\bfseries,
}

\begin{figure*}
\footnotesize
\begin{lstlisting}[basicstyle=\footnotesize\ttfamily]
Name: grid-x1-y3-t3-k50-l10-p100 (grid_x-1_y-3_t-3_k-5_l-1.pddl)
Objects: 
f0-0f, f0-1f, f0-2f, key1-0, key1-1, key1-2, key1-3, key1-4, shape0, shape1
shape2
Initial: 
conn(f0-1f, f0-0f), conn(f0-0f, f0-1f), conn(f0-2f, f0-1f), conn(f0-1f, f0-2f)
key-shape(key1-0, shape1), key-shape(key1-1, shape1), key-shape(key1-2, shape1)
key-shape(key1-3, shape1), key-shape(key1-4, shape1), lock-shape(f0-2f, shape1)
at(key1-0, f0-0f), at(key1-2, f0-0f), at(key1-1, f0-1f), at(key1-3, f0-1f)
at(key1-4, f0-2f), at-robot(f0-0f), place(f0-0f), place(f0-1f), place(f0-2f)
key(key1-0), key(key1-1), key(key1-2), key(key1-3), key(key1-4), shape(shape0)
shape(shape1), shape(shape2), locked(f0-2f), open(f0-0f), open(f0-1f)
arm-empty()
Goal: 
at(key1-0, f0-1f), at(key1-1, f0-0f), at(key1-2, f0-2f), at(key1-3, f0-0f)
at(key1-4, f0-1f)

Plan has path-cycle: unchecked
Plan has subgoal-cycle: false
Primitive plan: 16
Plan: 10
1  pickup(f0-0f, key1-0)
2  move(f0-0f, f0-1f) -> pickup-and-loose(f0-1f, key1-1, key1-0)
3  pickup-and-loose(f0-1f, key1-3, key1-1)
4  move(f0-1f, f0-0f)
5  putdown(f0-0f, key1-3)
6  move(f0-0f, f0-1f) -> pickup(f0-1f, key1-1)
7  move(f0-1f, f0-0f) -> pickup-and-loose(f0-0f, key1-2, key1-1)
8  move(f0-0f, f0-1f) -> unlock(f0-1f, f0-2f, key1-2, shape1) -> move(f0-1f, f0-2f)
    ->pickup-and-loose(f0-2f, key1-4, key1-2)
9  move(f0-2f, f0-1f)
10 putdown(f0-1f, key1-4)
\end{lstlisting}
\end{figure*}

\clearpage

\lstset{
    basicstyle=\footnotesize\ttfamily,
    keywordstyle=\bfseries, % This will apply bold to all keywords
    % Define colors for different groups of keywords
    morekeywords=[1]{Domain},
    keywordstyle=[1]\color{red}\bfseries,
    morekeywords=[2]{Objects, Primitive, Goal, Initial, Plan, plan},
    keywordstyle=[2]\bfseries,
    morekeywords=[3]{putdown, move, pickup, and, loose, unlock, pickup },
    keywordstyle=[3]\color{orange}\bfseries,
    morekeywords=[4]{f0-2f, f0-0f, key1-0, shape0, key1-3, key1-2, shape1, key1-4, shape2, f0-1f, key1-1 },
    keywordstyle=[4]\color{blue}\bfseries,
}

\begin{figure*}
\footnotesize
\begin{lstlisting}[basicstyle=\footnotesize\ttfamily]
Name: grid-x1-y3-t3-k50-l10-p100 (grid_x-1_y-3_t-3_k-5_l-1.pddl)
Objects: 
f0-0f, f0-1f, f0-2f, key1-0, key1-1, key1-2, key1-3, key1-4, shape0, shape1
shape2
Initial: 
conn(f0-1f, f0-0f), conn(f0-0f, f0-1f), conn(f0-2f, f0-1f), conn(f0-1f, f0-2f)
key-shape(key1-0, shape1), key-shape(key1-1, shape1), key-shape(key1-2, shape1)
key-shape(key1-3, shape1), key-shape(key1-4, shape1), lock-shape(f0-2f, shape1)
at(key1-0, f0-0f), at(key1-2, f0-0f), at(key1-1, f0-1f), at(key1-3, f0-1f)
at(key1-4, f0-2f), at-robot(f0-0f), place(f0-0f), place(f0-1f), place(f0-2f)
key(key1-0), key(key1-1), key(key1-2), key(key1-3), key(key1-4), shape(shape0)
shape(shape1), shape(shape2), locked(f0-2f), open(f0-0f), open(f0-1f)
arm-empty()
Goal: 
at(key1-0, f0-1f), at(key1-1, f0-0f), at(key1-2, f0-2f), at(key1-3, f0-0f)
at(key1-4, f0-1f)

Plan has path-cycle: unchecked
Plan has subgoal-cycle: false
Primitive plan: 16
Plan: 10
1  pickup(f0-0f, key1-0)
2  move(f0-0f, f0-1f) -> pickup-and-loose(f0-1f, key1-3, key1-0)
3  pickup-and-loose(f0-1f, key1-1, key1-3)
4  move(f0-1f, f0-0f)
5  putdown(f0-0f, key1-1)
6  move(f0-0f, f0-1f) -> pickup(f0-1f, key1-3)
7  move(f0-1f, f0-0f) -> pickup-and-loose(f0-0f, key1-2, key1-3)
8  move(f0-0f, f0-1f) -> unlock(f0-1f, f0-2f, key1-2, shape1) -> move(f0-1f, f0-2f)
    ->pickup-and-loose(f0-2f, key1-4, key1-2)
9  move(f0-2f, f0-1f)
10 putdown(f0-1f, key1-4
\end{lstlisting}
\end{figure*}

\clearpage

\lstset{
    basicstyle=\footnotesize\ttfamily,
    keywordstyle=\bfseries, % This will apply bold to all keywords
    % Define colors for different groups of keywords
    morekeywords=[1]{Domain},
    keywordstyle=[1]\color{red}\bfseries,
    morekeywords=[2]{Objects, Primitive, Goal, Initial, Plan, plan},
    keywordstyle=[2]\bfseries,
    morekeywords=[3]{putdown, move, pickup, and, loose, unlock, pickup },
    keywordstyle=[3]\color{orange}\bfseries,
    morekeywords=[4]{f0-2f, f0-0f, shape2, f0-6f, key1-0, shape0, f0-3f, key1-3, key1-2, f0-8f, shape1, key1-4, f0-7f, f0-4f, f0-1f, f0-5f, key1-1 },
    keywordstyle=[4]\color{blue}\bfseries,
}

\begin{figure*}
\footnotesize
% [inline block 0: 1 envs, 2117 chars -> code_tex | \begin{lstlisting}[basicstyle=\footnotesize\ttfamily] Name: grid-x1-y9-t3-k50-l30-p100 (grid_x-1_y-9_t-3_k-5_l-3.pddl)...]

\end{figure*}

\clearpage

\lstset{
    basicstyle=\footnotesize\ttfamily,
    keywordstyle=\bfseries, % This will apply bold to all keywords
    % Define colors for different groups of keywords
    morekeywords=[1]{Domain},
    keywordstyle=[1]\color{red}\bfseries,
    morekeywords=[2]{Objects, Primitive, Goal, Initial, Plan, plan},
    keywordstyle=[2]\bfseries,
    morekeywords=[3]{putdown, move, pickup, and, loose, unlock, pickup },
    keywordstyle=[3]\color{orange}\bfseries,
    morekeywords=[4]{f0-2f, f0-0f, shape2, f0-6f, key1-0, shape0, f0-3f, key1-3, key1-2, f0-8f, shape1, key1-4, f0-7f, f0-4f, f0-1f, f0-5f, key1-1 },
    keywordstyle=[4]\color{blue}\bfseries,
}

\begin{figure*}
\footnotesize
% [inline block 1: 1 envs, 2117 chars -> code_tex | \begin{lstlisting}[basicstyle=\footnotesize\ttfamily] Name: grid-x1-y9-t3-k50-l30-p100 (grid_x-1_y-9_t-3_k-5_l-3.pddl)...]

\end{figure*}

\clearpage

\lstset{
    basicstyle=\footnotesize\ttfamily,
    keywordstyle=\bfseries, % This will apply bold to all keywords
    % Define colors for different groups of keywords
    morekeywords=[1]{Domain},
    keywordstyle=[1]\color{red}\bfseries,
    morekeywords=[2]{Objects, Primitive, Goal, Initial, Plan, plan},
    keywordstyle=[2]\bfseries,
    morekeywords=[3]{putdown, move, pickup, and, loose, unlock, pickup },
    keywordstyle=[3]\color{orange}\bfseries,
    morekeywords=[4]{f0-2f, f0-0f, shape2, f0-6f, key1-0, shape0, f0-3f, key1-3, key1-2, f0-8f, shape1, key1-4, f0-7f, f0-4f, f0-1f, f0-5f, key1-1 },
    keywordstyle=[4]\color{blue}\bfseries,
}

\begin{figure*}
\footnotesize
% [inline block 2: 1 envs, 2117 chars -> code_tex | \begin{lstlisting}[basicstyle=\footnotesize\ttfamily] Name: grid-x1-y9-t3-k50-l30-p100 (grid_x-1_y-9_t-3_k-5_l-3.pddl)...]

\end{figure*}

\clearpage

\lstset{
    basicstyle=\footnotesize\ttfamily,
    keywordstyle=\bfseries, % This will apply bold to all keywords
    % Define colors for different groups of keywords
    morekeywords=[1]{Domain},
    keywordstyle=[1]\color{red}\bfseries,
    morekeywords=[2]{Objects, Primitive, Goal, Initial, Plan, plan},
    keywordstyle=[2]\bfseries,
    morekeywords=[3]{putdown, move, pickup, and, loose, unlock, pickup },
    keywordstyle=[3]\color{orange}\bfseries,
    morekeywords=[4]{f0-2f, f0-0f, shape2, f0-6f, key1-0, shape0, f0-3f, key1-3, key1-2, f0-8f, shape1, key1-4, f0-7f, f0-4f, f0-1f, f0-5f, key1-1 },
    keywordstyle=[4]\color{blue}\bfseries,
}

\begin{figure*}
\footnotesize
% [inline block 3: 1 envs, 2117 chars -> code_tex | \begin{lstlisting}[basicstyle=\footnotesize\ttfamily] Name: grid-x1-y9-t3-k50-l30-p100 (grid_x-1_y-9_t-3_k-5_l-3.pddl)...]

\end{figure*}

\clearpage

\lstset{
    basicstyle=\footnotesize\ttfamily,
    keywordstyle=\bfseries, % This will apply bold to all keywords
    % Define colors for different groups of keywords
    morekeywords=[1]{Domain},
    keywordstyle=[1]\color{red}\bfseries,
    morekeywords=[2]{Objects, Primitive, Goal, Initial, Plan, plan},
    keywordstyle=[2]\bfseries,
    morekeywords=[3]{putdown, move, pickup, and, loose, unlock, pickup },
    keywordstyle=[3]\color{orange}\bfseries,
    morekeywords=[4]{f0-2f, f0-0f, f1-9f, key2-2, shape0, f1-4f, key2-4, f0-8f, shape1, f1-1f, f1-5f, f1-0f, shape2, f0-1f, f1-2f, key2-3, key2-6, key2-0, f1-6f, f0-11f, f1-7f, f1-12f, f0-7f, f1-10f, f0-10f, key2-5, f0-12f, f0-4f, f1-3f, f1-11f, f0-9f, f0-6f, key2-1, f0-3f, f1-8f, f0-5f },
    keywordstyle=[4]\color{blue}\bfseries,
}

\begin{figure*}
\footnotesize
% [inline block 4: 1 envs, 6335 chars -> code_tex | \begin{lstlisting}[basicstyle=\footnotesize\ttfamily] Name: grid-x2-y13-t3-k7-l7-p100 (grid_x-2_y-13_t-3_k-7_l-7.pddl)...]

\end{figure*}

\clearpage

\lstset{
    basicstyle=\footnotesize\ttfamily,
    keywordstyle=\bfseries, % This will apply bold to all keywords
    % Define colors for different groups of keywords
    morekeywords=[1]{Domain},
    keywordstyle=[1]\color{red}\bfseries,
    morekeywords=[2]{Objects, Primitive, Goal, Initial, Plan, plan},
    keywordstyle=[2]\bfseries,
    morekeywords=[3]{putdown, move, pickup, and, loose, unlock, pickup },
    keywordstyle=[3]\color{orange}\bfseries,
    morekeywords=[4]{f0-2f, f0-0f, f1-9f, key2-2, shape0, f1-4f, key2-4, f0-8f, shape1, f1-1f, f1-5f, f1-0f, shape2, f0-1f, f1-2f, key2-3, key2-6, key2-0, f1-6f, f0-11f, f1-7f, f1-12f, f0-7f, f1-10f, f0-10f, key2-5, f0-12f, f0-4f, f1-3f, f1-11f, f0-9f, f0-6f, key2-1, f0-3f, f1-8f, f0-5f },
    keywordstyle=[4]\color{blue}\bfseries,
}

\begin{figure*}
\footnotesize
% [inline block 5: 1 envs, 6335 chars -> code_tex | \begin{lstlisting}[basicstyle=\footnotesize\ttfamily] Name: grid-x2-y13-t3-k7-l7-p100 (grid_x-2_y-13_t-3_k-7_l-7.pddl)...]

\end{figure*}

\clearpage

\lstset{
    basicstyle=\footnotesize\ttfamily,
    keywordstyle=\bfseries, % This will apply bold to all keywords
    % Define colors for different groups of keywords
    morekeywords=[1]{Domain},
    keywordstyle=[1]\color{red}\bfseries,
    morekeywords=[2]{Objects, Primitive, Goal, Initial, Plan, plan},
    keywordstyle=[2]\bfseries,
    morekeywords=[3]{putdown, move, pickup, and, loose, unlock, pickup },
    keywordstyle=[3]\color{orange}\bfseries,
    morekeywords=[4]{f0-2f, f0-0f, f1-9f, key2-2, shape0, f1-4f, key2-4, f0-8f, shape1, f1-1f, f1-5f, f1-0f, shape2, f0-1f, f1-2f, key2-3, key2-6, key2-0, f1-6f, f0-11f, f1-7f, f1-12f, f0-7f, f1-10f, f0-10f, key2-5, f0-12f, f0-4f, f1-3f, f1-11f, f0-9f, f0-6f, key2-1, f0-3f, f1-8f, f0-5f },
    keywordstyle=[4]\color{blue}\bfseries,
}

\begin{figure*}
\footnotesize
% [inline block 6: 1 envs, 6335 chars -> code_tex | \begin{lstlisting}[basicstyle=\footnotesize\ttfamily] Name: grid-x2-y13-t3-k7-l7-p100 (grid_x-2_y-13_t-3_k-7_l-7.pddl)...]

\end{figure*}

\clearpage

\lstset{
    basicstyle=\footnotesize\ttfamily,
    keywordstyle=\bfseries, % This will apply bold to all keywords
    % Define colors for different groups of keywords
    morekeywords=[1]{Domain},
    keywordstyle=[1]\color{red}\bfseries,
    morekeywords=[2]{Objects, Primitive, Goal, Initial, Plan, plan},
    keywordstyle=[2]\bfseries,
    morekeywords=[3]{putdown, move, pickup, and, loose, unlock, pickup },
    keywordstyle=[3]\color{orange}\bfseries,
    morekeywords=[4]{f0-2f, f0-0f, f1-9f, key2-2, shape0, f1-4f, key2-4, f0-8f, shape1, f1-1f, f1-5f, f1-0f, shape2, f0-1f, f1-2f, key2-3, key2-6, key2-0, f1-6f, f0-11f, f1-7f, f1-12f, f0-7f, f1-10f, f0-10f, key2-5, f0-12f, f0-4f, f1-3f, f1-11f, f0-9f, f0-6f, key2-1, f0-3f, f1-8f, f0-5f },
    keywordstyle=[4]\color{blue}\bfseries,
}

\begin{figure*}
\footnotesize
% [inline block 7: 1 envs, 6335 chars -> code_tex | \begin{lstlisting}[basicstyle=\footnotesize\ttfamily] Name: grid-x2-y13-t3-k7-l7-p100 (grid_x-2_y-13_t-3_k-7_l-7.pddl)...]

\end{figure*}

\clearpage

\lstset{
    basicstyle=\footnotesize\ttfamily,
    keywordstyle=\bfseries, % This will apply bold to all keywords
    % Define colors for different groups of keywords
    morekeywords=[1]{Domain},
    keywordstyle=[1]\color{red}\bfseries,
    morekeywords=[2]{Objects, Primitive, Goal, Initial, Plan, plan},
    keywordstyle=[2]\bfseries,
    morekeywords=[3]{putdown, move, pickup, and, loose, unlock, pickup },
    keywordstyle=[3]\color{orange}\bfseries,
    morekeywords=[4]{f0-2f, f0-0f, key1-0, f1-2f, shape0, f1-4f, f0-3f, key1-3, key1-2, shape1, f1-1f, f1-3f, f1-0f, f0-4f, f0-1f, key1-1 },
    keywordstyle=[4]\color{blue}\bfseries,
}

\begin{figure*}
\footnotesize
% [inline block 8: 1 envs, 2629 chars -> code_tex | \begin{lstlisting}[basicstyle=\footnotesize\ttfamily] Name: grid-x2-y5-t2-k4-l8-p100 (grid_x-2_y-5_t-2_k-4_l-8.pddl)...]

\end{figure*}

\clearpage

\lstset{
    basicstyle=\footnotesize\ttfamily,
    keywordstyle=\bfseries, % This will apply bold to all keywords
    % Define colors for different groups of keywords
    morekeywords=[1]{Domain},
    keywordstyle=[1]\color{red}\bfseries,
    morekeywords=[2]{Objects, Primitive, Goal, Initial, Plan, plan},
    keywordstyle=[2]\bfseries,
    morekeywords=[3]{putdown, move, pickup, and, loose, unlock, pickup },
    keywordstyle=[3]\color{orange}\bfseries,
    morekeywords=[4]{f0-2f, f0-0f, key1-0, f1-2f, shape0, f1-4f, f0-3f, key1-3, key1-2, shape1, f1-1f, f1-3f, f1-0f, f0-4f, f0-1f, key1-1 },
    keywordstyle=[4]\color{blue}\bfseries,
}

\begin{figure*}
\footnotesize
% [inline block 9: 1 envs, 2629 chars -> code_tex | \begin{lstlisting}[basicstyle=\footnotesize\ttfamily] Name: grid-x2-y5-t2-k4-l8-p100 (grid_x-2_y-5_t-2_k-4_l-8.pddl)...]

\end{figure*}

\clearpage

\lstset{
    basicstyle=\footnotesize\ttfamily,
    keywordstyle=\bfseries, % This will apply bold to all keywords
    % Define colors for different groups of keywords
    morekeywords=[1]{Domain},
    keywordstyle=[1]\color{red}\bfseries,
    morekeywords=[2]{Objects, Primitive, Goal, Initial, Plan, plan},
    keywordstyle=[2]\bfseries,
    morekeywords=[3]{putdown, move, pickup, and, loose, unlock, pickup },
    keywordstyle=[3]\color{orange}\bfseries,
    morekeywords=[4]{f0-2f, f0-0f, f2-3f, f1-2f, shape0, f1-4f, f2-0f, f0-3f, f2-1f, shape1, f1-1f, f2-2f, f1-3f, f1-0f, f0-4f, f0-1f, f2-4f, key0-0 },
    keywordstyle=[4]\color{blue}\bfseries,
}

\begin{figure*}
\footnotesize
% [inline block 10: 1 envs, 2063 chars -> code_tex | \begin{lstlisting}[basicstyle=\footnotesize\ttfamily] Name: grid-x3-y5-t2-k10-l20-p100 (grid_x-3_y-5_t-2_k-1_l-2.pddl)...]

\end{figure*}

\clearpage

\lstset{
    basicstyle=\footnotesize\ttfamily,
    keywordstyle=\bfseries, % This will apply bold to all keywords
    % Define colors for different groups of keywords
    morekeywords=[1]{Domain},
    keywordstyle=[1]\color{red}\bfseries,
    morekeywords=[2]{Objects, Primitive, Goal, Initial, Plan, plan},
    keywordstyle=[2]\bfseries,
    morekeywords=[3]{putdown, move, pickup, and, loose, unlock, pickup },
    keywordstyle=[3]\color{orange}\bfseries,
    morekeywords=[4]{f0-2f, f0-0f, f2-3f, f1-2f, shape0, f1-4f, f2-0f, f0-3f, f2-1f, shape1, f1-1f, f2-2f, f1-3f, f1-0f, f0-4f, f0-1f, f2-4f, key0-0 },
    keywordstyle=[4]\color{blue}\bfseries,
}

\begin{figure*}
\footnotesize
% [inline block 11: 1 envs, 2063 chars -> code_tex | \begin{lstlisting}[basicstyle=\footnotesize\ttfamily] Name: grid-x3-y5-t2-k10-l20-p100 (grid_x-3_y-5_t-2_k-1_l-2.pddl)...]

\end{figure*}

\clearpage

\lstset{
    basicstyle=\footnotesize\ttfamily,
    keywordstyle=\bfseries, % This will apply bold to all keywords
    % Define colors for different groups of keywords
    morekeywords=[1]{Domain},
    keywordstyle=[1]\color{red}\bfseries,
    morekeywords=[2]{Objects, Primitive, Goal, Initial, Plan, plan},
    keywordstyle=[2]\bfseries,
    morekeywords=[3]{putdown, move, pickup, and, loose, unlock, pickup },
    keywordstyle=[3]\color{orange}\bfseries,
    morekeywords=[4]{f0-2f, f0-0f, f2-3f, f1-2f, shape0, f1-4f, f2-0f, f0-3f, f2-1f, shape1, f1-1f, f2-2f, f1-3f, f1-0f, f0-4f, f0-1f, f2-4f, key0-0 },
    keywordstyle=[4]\color{blue}\bfseries,
}

\begin{figure*}
\footnotesize
% [inline block 12: 1 envs, 2063 chars -> code_tex | \begin{lstlisting}[basicstyle=\footnotesize\ttfamily] Name: grid-x3-y5-t2-k10-l20-p100 (grid_x-3_y-5_t-2_k-1_l-2.pddl)...]

\end{figure*}

\clearpage

\lstset{
    basicstyle=\footnotesize\ttfamily,
    keywordstyle=\bfseries, % This will apply bold to all keywords
    % Define colors for different groups of keywords
    morekeywords=[1]{Domain},
    keywordstyle=[1]\color{red}\bfseries,
    morekeywords=[2]{Objects, Primitive, Goal, Initial, Plan, plan},
    keywordstyle=[2]\bfseries,
    morekeywords=[3]{putdown, move, pickup, and, loose, unlock, pickup },
    keywordstyle=[3]\color{orange}\bfseries,
    morekeywords=[4]{f0-2f, f0-0f, f2-3f, f1-2f, shape0, f1-4f, f2-0f, f0-3f, f2-1f, shape1, f1-1f, f2-2f, f1-3f, f1-0f, f0-4f, f0-1f, f2-4f, key0-0 },
    keywordstyle=[4]\color{blue}\bfseries,
}

\begin{figure*}
\footnotesize
% [inline block 13: 1 envs, 2063 chars -> code_tex | \begin{lstlisting}[basicstyle=\footnotesize\ttfamily] Name: grid-x3-y5-t2-k10-l20-p100 (grid_x-3_y-5_t-2_k-1_l-2.pddl)...]

\end{figure*}

\clearpage

\lstset{
    basicstyle=\footnotesize\ttfamily,
    keywordstyle=\bfseries, % This will apply bold to all keywords
    % Define colors for different groups of keywords
    morekeywords=[1]{Domain},
    keywordstyle=[1]\color{red}\bfseries,
    morekeywords=[2]{Objects, Primitive, Goal, Initial, Plan, plan},
    keywordstyle=[2]\bfseries,
    morekeywords=[3]{putdown, move, pickup, and, loose, unlock, pickup },
    keywordstyle=[3]\color{orange}\bfseries,
    morekeywords=[4]{f0-2f, f0-0f, f2-3f, key1-0, shape0, f1-4f, shape1, f1-1f, key1-4, f1-0f, shape2, f0-1f, f2-4f, f1-2f, f2-0f, key1-3, key1-2, f1-3f, f0-3f, f2-1f, f2-2f, f0-4f, key1-1 },
    keywordstyle=[4]\color{blue}\bfseries,
}

\begin{figure*}
\footnotesize
% [inline block 14: 1 envs, 4640 chars -> code_tex | \begin{lstlisting}[basicstyle=\footnotesize\ttfamily] Name: grid-x3-y5-t3-k50-l30-p100 (grid_x-3_y-5_t-3_k-5_l-3.pddl)...]

\end{figure*}

\clearpage

\lstset{
    basicstyle=\footnotesize\ttfamily,
    keywordstyle=\bfseries, % This will apply bold to all keywords
    % Define colors for different groups of keywords
    morekeywords=[1]{Domain},
    keywordstyle=[1]\color{red}\bfseries,
    morekeywords=[2]{Objects, Primitive, Goal, Initial, Plan, plan},
    keywordstyle=[2]\bfseries,
    morekeywords=[3]{putdown, move, pickup, and, loose, unlock, pickup },
    keywordstyle=[3]\color{orange}\bfseries,
    morekeywords=[4]{f0-2f, f0-0f, f2-3f, key1-0, shape0, f1-4f, shape1, f1-1f, key1-4, f1-0f, shape2, f0-1f, f2-4f, f1-2f, f2-0f, key1-3, key1-2, f1-3f, f0-3f, f2-1f, f2-2f, f0-4f, key1-1 },
    keywordstyle=[4]\color{blue}\bfseries,
}

\begin{figure*}
\footnotesize
% [inline block 15: 1 envs, 4684 chars -> code_tex | \begin{lstlisting}[basicstyle=\footnotesize\ttfamily] Name: grid-x3-y5-t3-k50-l30-p100 (grid_x-3_y-5_t-3_k-5_l-3.pddl)...]

\end{figure*}

\clearpage

\lstset{
    basicstyle=\footnotesize\ttfamily,
    keywordstyle=\bfseries, % This will apply bold to all keywords
    % Define colors for different groups of keywords
    morekeywords=[1]{Domain},
    keywordstyle=[1]\color{red}\bfseries,
    morekeywords=[2]{Objects, Primitive, Goal, Initial, Plan, plan},
    keywordstyle=[2]\bfseries,
    morekeywords=[3]{putdown, move, pickup, and, loose, unlock, pickup },
    keywordstyle=[3]\color{orange}\bfseries,
    morekeywords=[4]{f0-2f, f0-0f, f2-3f, key1-0, shape0, f1-4f, shape1, f1-1f, f1-5f, key1-4, f1-0f, f0-1f, f2-4f, f1-2f, f2-0f, f0-4f, key1-3, key1-2, f1-3f, f0-3f, f2-1f, f2-2f, f2-5f, f0-5f, key1-1 },
    keywordstyle=[4]\color{blue}\bfseries,
}

\begin{figure*}
\footnotesize
% [inline block 16: 1 envs, 8491 chars -> code_tex | \begin{lstlisting}[basicstyle=\footnotesize\ttfamily] Name: grid-x3-y6-t2-k5-l4-p100 (grid_x-3_y-6_t-2_k-5_l-4.pddl)...]

\end{figure*}

\clearpage

\lstset{
    basicstyle=\footnotesize\ttfamily,
    keywordstyle=\bfseries, % This will apply bold to all keywords
    % Define colors for different groups of keywords
    morekeywords=[1]{Domain},
    keywordstyle=[1]\color{red}\bfseries,
    morekeywords=[2]{Objects, Primitive, Goal, Initial, Plan, plan},
    keywordstyle=[2]\bfseries,
    morekeywords=[3]{putdown, move, pickup, and, loose, unlock, pickup },
    keywordstyle=[3]\color{orange}\bfseries,
    morekeywords=[4]{f0-2f, f0-0f, f2-3f, key1-0, shape0, f1-4f, shape1, f1-1f, f1-5f, key1-4, f1-0f, f0-1f, f2-4f, f1-2f, f2-0f, f0-4f, key1-3, key1-2, f1-3f, f0-3f, f2-1f, f2-2f, f2-5f, f0-5f, key1-1 },
    keywordstyle=[4]\color{blue}\bfseries,
}

\begin{figure*}
\footnotesize
% [inline block 17: 1 envs, 8394 chars -> code_tex | \begin{lstlisting}[basicstyle=\footnotesize\ttfamily] Name: grid-x3-y6-t2-k5-l4-p100 (grid_x-3_y-6_t-2_k-5_l-4.pddl)...]

\end{figure*}

\clearpage

\lstset{
    basicstyle=\footnotesize\ttfamily,
    keywordstyle=\bfseries, % This will apply bold to all keywords
    % Define colors for different groups of keywords
    morekeywords=[1]{Domain},
    keywordstyle=[1]\color{red}\bfseries,
    morekeywords=[2]{Objects, Primitive, Goal, Initial, Plan, plan},
    keywordstyle=[2]\bfseries,
    morekeywords=[3]{putdown, move, pickup, and, loose, unlock, pickup },
    keywordstyle=[3]\color{orange}\bfseries,
    morekeywords=[4]{f0-2f, f0-0f, f2-3f, shape0, f1-4f, shape1, f1-1f, f1-5f, f1-0f, f0-1f, f2-4f, f1-2f, f1-6f, f2-0f, f0-4f, f1-3f, f2-6f, key0-0, f0-6f, f0-3f, f2-1f, f2-2f, f2-5f, f0-5f },
    keywordstyle=[4]\color{blue}\bfseries,
}

\begin{figure*}
\footnotesize
% [inline block 18: 1 envs, 2612 chars -> code_tex | \begin{lstlisting}[basicstyle=\footnotesize\ttfamily] Name: grid-x3-y7-t2-k10-l10-p100 (grid_x-3_y-7_t-2_k-1_l-1.pddl)...]

\end{figure*}

\clearpage

\lstset{
    basicstyle=\footnotesize\ttfamily,
    keywordstyle=\bfseries, % This will apply bold to all keywords
    % Define colors for different groups of keywords
    morekeywords=[1]{Domain},
    keywordstyle=[1]\color{red}\bfseries,
    morekeywords=[2]{Objects, Primitive, Goal, Initial, Plan, plan},
    keywordstyle=[2]\bfseries,
    morekeywords=[3]{putdown, move, pickup, and, loose, unlock, pickup },
    keywordstyle=[3]\color{orange}\bfseries,
    morekeywords=[4]{f0-2f, f0-0f, f2-3f, shape0, f1-4f, shape1, f1-1f, f1-5f, f1-0f, f0-1f, f2-4f, f1-2f, f1-6f, f2-0f, f0-4f, f1-3f, f2-6f, key0-0, f0-6f, f0-3f, f2-1f, f2-2f, f2-5f, f0-5f },
    keywordstyle=[4]\color{blue}\bfseries,
}

\begin{figure*}
\footnotesize
% [inline block 19: 1 envs, 2612 chars -> code_tex | \begin{lstlisting}[basicstyle=\footnotesize\ttfamily] Name: grid-x3-y7-t2-k10-l10-p100 (grid_x-3_y-7_t-2_k-1_l-1.pddl)...]

\end{figure*}

\clearpage

\lstset{
    basicstyle=\footnotesize\ttfamily,
    keywordstyle=\bfseries, % This will apply bold to all keywords
    % Define colors for different groups of keywords
    morekeywords=[1]{Domain},
    keywordstyle=[1]\color{red}\bfseries,
    morekeywords=[2]{Objects, Primitive, Goal, Initial, Plan, plan},
    keywordstyle=[2]\bfseries,
    morekeywords=[3]{putdown, move, pickup, and, loose, unlock, pickup },
    keywordstyle=[3]\color{orange}\bfseries,
    morekeywords=[4]{f0-2f, f0-0f, f2-3f, shape0, f1-4f, shape1, f1-1f, f1-5f, f1-0f, f0-1f, f2-4f, f1-2f, f1-6f, f2-0f, f0-4f, f1-3f, f2-6f, key0-0, f0-6f, f0-3f, f2-1f, f2-2f, f2-5f, f0-5f },
    keywordstyle=[4]\color{blue}\bfseries,
}

\begin{figure*}
\footnotesize
% [inline block 20: 1 envs, 2612 chars -> code_tex | \begin{lstlisting}[basicstyle=\footnotesize\ttfamily] Name: grid-x3-y7-t2-k10-l10-p100 (grid_x-3_y-7_t-2_k-1_l-1.pddl)...]

\end{figure*}

\clearpage

\lstset{
    basicstyle=\footnotesize\ttfamily,
    keywordstyle=\bfseries, % This will apply bold to all keywords
    % Define colors for different groups of keywords
    morekeywords=[1]{Domain},
    keywordstyle=[1]\color{red}\bfseries,
    morekeywords=[2]{Objects, Primitive, Goal, Initial, Plan, plan},
    keywordstyle=[2]\bfseries,
    morekeywords=[3]{putdown, move, pickup, and, loose, unlock, pickup },
    keywordstyle=[3]\color{orange}\bfseries,
    morekeywords=[4]{f0-2f, f0-0f, f2-3f, shape0, f1-4f, shape1, f1-1f, f1-5f, f1-0f, f0-1f, f2-4f, f1-2f, f1-6f, f2-0f, f0-4f, f1-3f, f2-6f, key0-0, f0-6f, f0-3f, f2-1f, f2-2f, f2-5f, f0-5f },
    keywordstyle=[4]\color{blue}\bfseries,
}

\begin{figure*}
\footnotesize
% [inline block 21: 1 envs, 2612 chars -> code_tex | \begin{lstlisting}[basicstyle=\footnotesize\ttfamily] Name: grid-x3-y7-t2-k10-l10-p100 (grid_x-3_y-7_t-2_k-1_l-1.pddl)...]

\end{figure*}

\clearpage

\lstset{
    basicstyle=\footnotesize\ttfamily,
    keywordstyle=\bfseries, % This will apply bold to all keywords
    % Define colors for different groups of keywords
    morekeywords=[1]{Domain},
    keywordstyle=[1]\color{red}\bfseries,
    morekeywords=[2]{Objects, Primitive, Goal, Initial, Plan, plan},
    keywordstyle=[2]\bfseries,
    morekeywords=[3]{putdown, move, pickup, and, loose, unlock, pickup },
    keywordstyle=[3]\color{orange}\bfseries,
    morekeywords=[4]{f0-2f, f0-0f, f2-3f, key1-0, shape0, f1-4f, shape1, f1-1f, f1-5f, key1-4, f1-0f, shape2, f0-1f, f2-4f, f1-2f, f1-6f, f2-0f, f0-4f, key1-3, key1-2, f1-3f, f2-6f, f0-6f, f0-3f, f2-1f, f2-2f, f2-5f, f0-5f, key1-1 },
    keywordstyle=[4]\color{blue}\bfseries,
}

\begin{figure*}
\footnotesize
% [inline block 22: 1 envs, 3521 chars -> code_tex | \begin{lstlisting}[basicstyle=\footnotesize\ttfamily] Name: grid-x3-y7-t3-k50-l30-p100 (grid_x-3_y-7_t-3_k-5_l-3.pddl)...]

\end{figure*}

\clearpage

\lstset{
    basicstyle=\footnotesize\ttfamily,
    keywordstyle=\bfseries, % This will apply bold to all keywords
    % Define colors for different groups of keywords
    morekeywords=[1]{Domain},
    keywordstyle=[1]\color{red}\bfseries,
    morekeywords=[2]{Objects, Primitive, Goal, Initial, Plan, plan},
    keywordstyle=[2]\bfseries,
    morekeywords=[3]{putdown, move, pickup, and, loose, unlock, pickup },
    keywordstyle=[3]\color{orange}\bfseries,
    morekeywords=[4]{f0-2f, f0-0f, f2-3f, key1-0, shape0, f1-4f, shape1, f1-1f, f1-5f, key1-4, f1-0f, shape2, f0-1f, f2-4f, f1-2f, f1-6f, f2-0f, f0-4f, key1-3, key1-2, f1-3f, f2-6f, f0-6f, f0-3f, f2-1f, f2-2f, f2-5f, f0-5f, key1-1 },
    keywordstyle=[4]\color{blue}\bfseries,
}

\begin{figure*}
\footnotesize
% [inline block 23: 1 envs, 3521 chars -> code_tex | \begin{lstlisting}[basicstyle=\footnotesize\ttfamily] Name: grid-x3-y7-t3-k50-l30-p100 (grid_x-3_y-7_t-3_k-5_l-3.pddl)...]

\end{figure*}

\clearpage

\lstset{
    basicstyle=\footnotesize\ttfamily,
    keywordstyle=\bfseries, % This will apply bold to all keywords
    % Define colors for different groups of keywords
    morekeywords=[1]{Domain},
    keywordstyle=[1]\color{red}\bfseries,
    morekeywords=[2]{Objects, Primitive, Goal, Initial, Plan, plan},
    keywordstyle=[2]\bfseries,
    morekeywords=[3]{putdown, move, pickup, and, loose, unlock, pickup },
    keywordstyle=[3]\color{orange}\bfseries,
    morekeywords=[4]{f0-2f, f0-0f, f2-3f, key1-0, shape0, f1-4f, shape1, f1-1f, f1-5f, key1-4, f1-0f, shape2, f0-1f, f2-4f, f1-2f, f1-6f, f2-0f, f0-4f, key1-3, key1-2, f1-3f, f2-6f, f0-6f, f0-3f, f2-1f, f2-2f, f2-5f, f0-5f, key1-1 },
    keywordstyle=[4]\color{blue}\bfseries,
}

\begin{figure*}
\footnotesize
% [inline block 24: 1 envs, 3521 chars -> code_tex | \begin{lstlisting}[basicstyle=\footnotesize\ttfamily] Name: grid-x3-y7-t3-k50-l30-p100 (grid_x-3_y-7_t-3_k-5_l-3.pddl)...]

\end{figure*}

\clearpage

\lstset{
    basicstyle=\footnotesize\ttfamily,
    keywordstyle=\bfseries, % This will apply bold to all keywords
    % Define colors for different groups of keywords
    morekeywords=[1]{Domain},
    keywordstyle=[1]\color{red}\bfseries,
    morekeywords=[2]{Objects, Primitive, Goal, Initial, Plan, plan},
    keywordstyle=[2]\bfseries,
    morekeywords=[3]{putdown, move, pickup, and, loose, unlock, pickup },
    keywordstyle=[3]\color{orange}\bfseries,
    morekeywords=[4]{f0-2f, f0-0f, f2-3f, key1-0, shape0, f1-4f, shape1, f1-1f, f1-5f, key1-4, f1-0f, shape2, f0-1f, f2-4f, f1-2f, f1-6f, f2-0f, f0-4f, key1-3, key1-2, f1-3f, f2-6f, f0-6f, f0-3f, f2-1f, f2-2f, f2-5f, f0-5f, key1-1 },
    keywordstyle=[4]\color{blue}\bfseries,
}

\begin{figure*}
\footnotesize
% [inline block 25: 1 envs, 3521 chars -> code_tex | \begin{lstlisting}[basicstyle=\footnotesize\ttfamily] Name: grid-x3-y7-t3-k50-l30-p100 (grid_x-3_y-7_t-3_k-5_l-3.pddl)...]

\end{figure*}

\clearpage

\lstset{
    basicstyle=\footnotesize\ttfamily,
    keywordstyle=\bfseries, % This will apply bold to all keywords
    % Define colors for different groups of keywords
    morekeywords=[1]{Domain},
    keywordstyle=[1]\color{red}\bfseries,
    morekeywords=[2]{Objects, Primitive, Goal, Initial, Plan, plan},
    keywordstyle=[2]\bfseries,
    morekeywords=[3]{putdown, move, pickup, and, loose, unlock, pickup },
    keywordstyle=[3]\color{orange}\bfseries,
    morekeywords=[4]{f0-2f, f0-0f, f2-3f, f2-7f, shape0, f1-4f, f2-8f, f0-8f, shape1, f1-1f, f1-5f, f1-0f, f0-1f, f2-4f, f1-2f, f1-6f, f1-7f, f0-7f, f2-0f, f0-4f, f1-3f, f2-6f, key0-0, f0-6f, f1-8f, f0-3f, f2-1f, f2-2f, f2-5f, f0-5f },
    keywordstyle=[4]\color{blue}\bfseries,
}

\begin{figure*}
\footnotesize
% [inline block 26: 1 envs, 3274 chars -> code_tex | \begin{lstlisting}[basicstyle=\footnotesize\ttfamily] Name: grid-x3-y9-t2-k10-l10-p100 (grid_x-3_y-9_t-2_k-1_l-1.pddl)...]

\end{figure*}

\clearpage

\lstset{
    basicstyle=\footnotesize\ttfamily,
    keywordstyle=\bfseries, % This will apply bold to all keywords
    % Define colors for different groups of keywords
    morekeywords=[1]{Domain},
    keywordstyle=[1]\color{red}\bfseries,
    morekeywords=[2]{Objects, Primitive, Goal, Initial, Plan, plan},
    keywordstyle=[2]\bfseries,
    morekeywords=[3]{putdown, move, pickup, and, loose, unlock, pickup },
    keywordstyle=[3]\color{orange}\bfseries,
    morekeywords=[4]{f0-2f, f0-0f, f2-3f, f2-7f, shape0, f1-4f, f2-8f, f0-8f, shape1, f1-1f, f1-5f, f1-0f, f0-1f, f2-4f, f1-2f, f1-6f, f1-7f, f0-7f, f2-0f, f0-4f, f1-3f, f2-6f, key0-0, f0-6f, f1-8f, f0-3f, f2-1f, f2-2f, f2-5f, f0-5f },
    keywordstyle=[4]\color{blue}\bfseries,
}

\begin{figure*}
\footnotesize
% [inline block 27: 1 envs, 3274 chars -> code_tex | \begin{lstlisting}[basicstyle=\footnotesize\ttfamily] Name: grid-x3-y9-t2-k10-l10-p100 (grid_x-3_y-9_t-2_k-1_l-1.pddl)...]

\end{figure*}

\clearpage

\lstset{
    basicstyle=\footnotesize\ttfamily,
    keywordstyle=\bfseries, % This will apply bold to all keywords
    % Define colors for different groups of keywords
    morekeywords=[1]{Domain},
    keywordstyle=[1]\color{red}\bfseries,
    morekeywords=[2]{Objects, Primitive, Goal, Initial, Plan, plan},
    keywordstyle=[2]\bfseries,
    morekeywords=[3]{putdown, move, pickup, and, loose, unlock, pickup },
    keywordstyle=[3]\color{orange}\bfseries,
    morekeywords=[4]{f0-2f, f0-0f, f2-3f, f2-7f, shape0, f1-4f, f2-8f, f0-8f, shape1, f1-1f, f1-5f, f1-0f, f0-1f, f2-4f, f1-2f, f1-6f, f1-7f, f0-7f, f2-0f, f0-4f, f1-3f, f2-6f, key0-0, f0-6f, f1-8f, f0-3f, f2-1f, f2-2f, f2-5f, f0-5f },
    keywordstyle=[4]\color{blue}\bfseries,
}

\begin{figure*}
\footnotesize
% [inline block 28: 1 envs, 3274 chars -> code_tex | \begin{lstlisting}[basicstyle=\footnotesize\ttfamily] Name: grid-x3-y9-t2-k10-l10-p100 (grid_x-3_y-9_t-2_k-1_l-1.pddl)...]

\end{figure*}

\clearpage

\lstset{
    basicstyle=\footnotesize\ttfamily,
    keywordstyle=\bfseries, % This will apply bold to all keywords
    % Define colors for different groups of keywords
    morekeywords=[1]{Domain},
    keywordstyle=[1]\color{red}\bfseries,
    morekeywords=[2]{Objects, Primitive, Goal, Initial, Plan, plan},
    keywordstyle=[2]\bfseries,
    morekeywords=[3]{putdown, move, pickup, and, loose, unlock, pickup },
    keywordstyle=[3]\color{orange}\bfseries,
    morekeywords=[4]{f0-2f, f0-0f, f2-3f, f2-7f, shape0, f1-4f, f2-8f, f0-8f, shape1, f1-1f, f1-5f, f1-0f, f0-1f, f2-4f, f1-2f, f1-6f, f1-7f, f0-7f, f2-0f, f0-4f, f1-3f, f2-6f, key0-0, f0-6f, f1-8f, f0-3f, f2-1f, f2-2f, f2-5f, f0-5f },
    keywordstyle=[4]\color{blue}\bfseries,
}

\begin{figure*}
\footnotesize
% [inline block 29: 1 envs, 3274 chars -> code_tex | \begin{lstlisting}[basicstyle=\footnotesize\ttfamily] Name: grid-x3-y9-t2-k10-l10-p100 (grid_x-3_y-9_t-2_k-1_l-1.pddl)...]

\end{figure*}

\clearpage

\lstset{
    basicstyle=\footnotesize\ttfamily,
    keywordstyle=\bfseries, % This will apply bold to all keywords
    % Define colors for different groups of keywords
    morekeywords=[1]{Domain},
    keywordstyle=[1]\color{red}\bfseries,
    morekeywords=[2]{Objects, Primitive, Goal, Initial, Plan, plan},
    keywordstyle=[2]\bfseries,
    morekeywords=[3]{putdown, move, pickup, and, loose, unlock, pickup },
    keywordstyle=[3]\color{orange}\bfseries,
    morekeywords=[4]{f0-2f, f0-0f, f2-3f, f2-7f, key1-0, shape0, f1-4f, f2-8f, f0-8f, shape1, f1-1f, f1-5f, key1-4, f1-0f, shape2, f0-1f, f2-4f, f1-2f, f1-6f, f1-7f, f0-7f, f2-0f, f0-4f, key1-3, key1-2, f1-3f, f2-6f, f0-6f, f1-8f, f0-3f, f2-1f, f2-2f, f2-5f, f0-5f, key1-1 },
    keywordstyle=[4]\color{blue}\bfseries,
}

\begin{figure*}
\footnotesize
% [inline block 30: 1 envs, 4240 chars -> code_tex | \begin{lstlisting}[basicstyle=\footnotesize\ttfamily] Name: grid-x3-y9-t3-k50-l30-p100 (grid_x-3_y-9_t-3_k-5_l-3.pddl)...]

\end{figure*}

\clearpage

\lstset{
    basicstyle=\footnotesize\ttfamily,
    keywordstyle=\bfseries, % This will apply bold to all keywords
    % Define colors for different groups of keywords
    morekeywords=[1]{Domain},
    keywordstyle=[1]\color{red}\bfseries,
    morekeywords=[2]{Objects, Primitive, Goal, Initial, Plan, plan},
    keywordstyle=[2]\bfseries,
    morekeywords=[3]{putdown, move, pickup, and, loose, unlock, pickup },
    keywordstyle=[3]\color{orange}\bfseries,
    morekeywords=[4]{f0-2f, f0-0f, f2-3f, f2-7f, key1-0, shape0, f1-4f, f2-8f, f0-8f, shape1, f1-1f, f1-5f, key1-4, f1-0f, shape2, f0-1f, f2-4f, f1-2f, f1-6f, f1-7f, f0-7f, f2-0f, f0-4f, key1-3, key1-2, f1-3f, f2-6f, f0-6f, f1-8f, f0-3f, f2-1f, f2-2f, f2-5f, f0-5f, key1-1 },
    keywordstyle=[4]\color{blue}\bfseries,
}

\begin{figure*}
\footnotesize
% [inline block 31: 1 envs, 4240 chars -> code_tex | \begin{lstlisting}[basicstyle=\footnotesize\ttfamily] Name: grid-x3-y9-t3-k50-l30-p100 (grid_x-3_y-9_t-3_k-5_l-3.pddl)...]

\end{figure*}

\clearpage

\lstset{
    basicstyle=\footnotesize\ttfamily,
    keywordstyle=\bfseries, % This will apply bold to all keywords
    % Define colors for different groups of keywords
    morekeywords=[1]{Domain},
    keywordstyle=[1]\color{red}\bfseries,
    morekeywords=[2]{Objects, Primitive, Goal, Initial, Plan, plan},
    keywordstyle=[2]\bfseries,
    morekeywords=[3]{putdown, move, pickup, and, loose, unlock, pickup },
    keywordstyle=[3]\color{orange}\bfseries,
    morekeywords=[4]{f0-2f, f0-0f, f2-3f, f2-7f, key1-0, shape0, f1-4f, f2-8f, f0-8f, shape1, f1-1f, f1-5f, key1-4, f1-0f, shape2, f0-1f, f2-4f, f1-2f, f1-6f, f1-7f, f0-7f, f2-0f, f0-4f, key1-3, key1-2, f1-3f, f2-6f, f0-6f, f1-8f, f0-3f, f2-1f, f2-2f, f2-5f, f0-5f, key1-1 },
    keywordstyle=[4]\color{blue}\bfseries,
}

\begin{figure*}
\footnotesize
% [inline block 32: 1 envs, 4240 chars -> code_tex | \begin{lstlisting}[basicstyle=\footnotesize\ttfamily] Name: grid-x3-y9-t3-k50-l30-p100 (grid_x-3_y-9_t-3_k-5_l-3.pddl)...]

\end{figure*}

\clearpage

\lstset{
    basicstyle=\footnotesize\ttfamily,
    keywordstyle=\bfseries, % This will apply bold to all keywords
    % Define colors for different groups of keywords
    morekeywords=[1]{Domain},
    keywordstyle=[1]\color{red}\bfseries,
    morekeywords=[2]{Objects, Primitive, Goal, Initial, Plan, plan},
    keywordstyle=[2]\bfseries,
    morekeywords=[3]{putdown, move, pickup, and, loose, unlock, pickup },
    keywordstyle=[3]\color{orange}\bfseries,
    morekeywords=[4]{f0-2f, f0-0f, f2-3f, f2-7f, key1-0, shape0, f1-4f, f2-8f, f0-8f, shape1, f1-1f, f1-5f, key1-4, f1-0f, shape2, f0-1f, f2-4f, f1-2f, f1-6f, f1-7f, f0-7f, f2-0f, f0-4f, key1-3, key1-2, f1-3f, f2-6f, f0-6f, f1-8f, f0-3f, f2-1f, f2-2f, f2-5f, f0-5f, key1-1 },
    keywordstyle=[4]\color{blue}\bfseries,
}

\begin{figure*}
\footnotesize
% [inline block 33: 1 envs, 4240 chars -> code_tex | \begin{lstlisting}[basicstyle=\footnotesize\ttfamily] Name: grid-x3-y9-t3-k50-l30-p100 (grid_x-3_y-9_t-3_k-5_l-3.pddl)...]

\end{figure*}

\clearpage

\lstset{
    basicstyle=\footnotesize\ttfamily,
    keywordstyle=\bfseries, % This will apply bold to all keywords
    % Define colors for different groups of keywords
    morekeywords=[1]{Domain},
    keywordstyle=[1]\color{red}\bfseries,
    morekeywords=[2]{Objects, Primitive, Goal, Initial, Plan, plan},
    keywordstyle=[2]\bfseries,
    morekeywords=[3]{putdown, move, pickup, and, loose, unlock, pickup },
    keywordstyle=[3]\color{orange}\bfseries,
    morekeywords=[4]{f0-2f, f0-0f, f2-3f, key2-2, f3-1f, shape0, f1-4f, key2-4, shape1, f1-1f, f1-5f, f1-0f, shape2, f0-1f, f2-4f, f1-2f, key2-3, key2-6, key2-0, f1-6f, f3-3f, key2-7, key2-5, f2-0f, f1-3f, f3-5f, f2-6f, f0-6f, key2-1, f2-5f, f0-3f, key2-8, f2-1f, f2-2f, f3-2f, f3-6f, f0-4f, f3-0f, f0-5f, f3-4f },
    keywordstyle=[4]\color{blue}\bfseries,
}

\begin{figure*}
\footnotesize
% [inline block 34: 1 envs, 10381 chars -> code_tex | \begin{lstlisting}[basicstyle=\footnotesize\ttfamily] Name: grid-x4-y7-t3-k9-l9-p100 (grid_x-4_y-7_t-3_k-9_l-9.pddl)...]

\end{figure*}

\clearpage

\lstset{
    basicstyle=\footnotesize\ttfamily,
    keywordstyle=\bfseries, % This will apply bold to all keywords
    % Define colors for different groups of keywords
    morekeywords=[1]{Domain},
    keywordstyle=[1]\color{red}\bfseries,
    morekeywords=[2]{Objects, Primitive, Goal, Initial, Plan, plan},
    keywordstyle=[2]\bfseries,
    morekeywords=[3]{putdown, move, pickup, and, loose, unlock, pickup },
    keywordstyle=[3]\color{orange}\bfseries,
    morekeywords=[4]{f0-2f, f0-0f, f2-3f, key2-2, f3-1f, shape0, f1-4f, key2-4, shape1, f1-1f, f1-5f, f1-0f, shape2, f0-1f, f2-4f, f1-2f, key2-3, key2-6, key2-0, f1-6f, f3-3f, key2-7, key2-5, f2-0f, f1-3f, f3-5f, f2-6f, f0-6f, key2-1, f2-5f, f0-3f, key2-8, f2-1f, f2-2f, f3-2f, f3-6f, f0-4f, f3-0f, f0-5f, f3-4f },
    keywordstyle=[4]\color{blue}\bfseries,
}

\begin{figure*}
\footnotesize
% [inline block 35: 1 envs, 10281 chars -> code_tex | \begin{lstlisting}[basicstyle=\footnotesize\ttfamily] Name: grid-x4-y7-t3-k9-l9-p100 (grid_x-4_y-7_t-3_k-9_l-9.pddl)...]

\end{figure*}

\clearpage

\lstset{
    basicstyle=\footnotesize\ttfamily,
    keywordstyle=\bfseries, % This will apply bold to all keywords
    % Define colors for different groups of keywords
    morekeywords=[1]{Domain},
    keywordstyle=[1]\color{red}\bfseries,
    morekeywords=[2]{Objects, Primitive, Goal, Initial, Plan, plan},
    keywordstyle=[2]\bfseries,
    morekeywords=[3]{putdown, move, pickup, and, loose, unlock, pickup },
    keywordstyle=[3]\color{orange}\bfseries,
    morekeywords=[4]{f0-2f, f0-0f, f2-3f, f2-7f, f3-1f, shape0, f1-4f, f1-1f, f1-5f, f1-0f, f0-1f, f2-4f, f1-2f, f1-6f, key0-3, f1-7f, key0-1, key0-2, f0-7f, f3-3f, f3-7f, f2-0f, f1-3f, f3-5f, f2-6f, key0-0, f0-6f, f2-5f, f0-3f, f2-1f, f2-2f, f3-2f, f3-6f, f0-4f, f3-0f, f0-5f, f3-4f },
    keywordstyle=[4]\color{blue}\bfseries,
}

\begin{figure*}
\footnotesize
% [inline block 36: 1 envs, 10512 chars -> code_tex | \begin{lstlisting}[basicstyle=\footnotesize\ttfamily] Name: grid-x4-y8-t1-k4-l4-p100 (grid_x-4_y-8_t-1_k-4_l-4.pddl)...]

\end{figure*}

\clearpage

\lstset{
    basicstyle=\footnotesize\ttfamily,
    keywordstyle=\bfseries, % This will apply bold to all keywords
    % Define colors for different groups of keywords
    morekeywords=[1]{Domain},
    keywordstyle=[1]\color{red}\bfseries,
    morekeywords=[2]{Objects, Primitive, Goal, Initial, Plan, plan},
    keywordstyle=[2]\bfseries,
    morekeywords=[3]{putdown, move, pickup, and, loose, unlock, pickup },
    keywordstyle=[3]\color{orange}\bfseries,
    morekeywords=[4]{f0-2f, f0-0f, f2-3f, f2-7f, f3-1f, shape0, f1-4f, f1-1f, f1-5f, f1-0f, f0-1f, f2-4f, f1-2f, f1-6f, key0-3, f1-7f, key0-1, key0-2, f0-7f, f3-3f, f3-7f, f2-0f, f1-3f, f3-5f, f2-6f, key0-0, f0-6f, f2-5f, f0-3f, f2-1f, f2-2f, f3-2f, f3-6f, f0-4f, f3-0f, f0-5f, f3-4f },
    keywordstyle=[4]\color{blue}\bfseries,
}

\begin{figure*}
\footnotesize
% [inline block 37: 1 envs, 10509 chars -> code_tex | \begin{lstlisting}[basicstyle=\footnotesize\ttfamily] Name: grid-x4-y8-t1-k4-l4-p100 (grid_x-4_y-8_t-1_k-4_l-4.pddl)...]

\end{figure*}

\clearpage

\lstset{
    basicstyle=\footnotesize\ttfamily,
    keywordstyle=\bfseries, % This will apply bold to all keywords
    % Define colors for different groups of keywords
    morekeywords=[1]{Domain},
    keywordstyle=[1]\color{red}\bfseries,
    morekeywords=[2]{Objects, Primitive, Goal, Initial, Plan, plan},
    keywordstyle=[2]\bfseries,
    morekeywords=[3]{putdown, move, pickup, and, loose, unlock, pickup },
    keywordstyle=[3]\color{orange}\bfseries,
    morekeywords=[4]{f0-2f, f0-0f, f2-3f, f2-7f, key1-0, f3-1f, shape0, f1-4f, shape1, f1-1f, f1-5f, f1-0f, f0-1f, f2-4f, f1-2f, f1-6f, f1-7f, f0-7f, f3-3f, f3-7f, f2-0f, key1-3, key1-2, f1-3f, f3-5f, f2-6f, f0-6f, f2-5f, f0-3f, f2-1f, f2-2f, f3-2f, f3-6f, f0-4f, f3-0f, f0-5f, f3-4f, key1-1 },
    keywordstyle=[4]\color{blue}\bfseries,
}

\begin{figure*}
\footnotesize
% [inline block 38: 1 envs, 10582 chars -> code_tex | \begin{lstlisting}[basicstyle=\footnotesize\ttfamily] Name: grid-x4-y8-t2-k4-l4-p100 (grid_x-4_y-8_t-2_k-4_l-4.pddl)...]

\end{figure*}

\clearpage

\lstset{
    basicstyle=\footnotesize\ttfamily,
    keywordstyle=\bfseries, % This will apply bold to all keywords
    % Define colors for different groups of keywords
    morekeywords=[1]{Domain},
    keywordstyle=[1]\color{red}\bfseries,
    morekeywords=[2]{Objects, Primitive, Goal, Initial, Plan, plan},
    keywordstyle=[2]\bfseries,
    morekeywords=[3]{putdown, move, pickup, and, loose, unlock, pickup },
    keywordstyle=[3]\color{orange}\bfseries,
    morekeywords=[4]{f0-2f, f0-0f, f2-3f, f2-7f, key1-0, f3-1f, shape0, f1-4f, shape1, f1-1f, f1-5f, f1-0f, f0-1f, f2-4f, f1-2f, f1-6f, f1-7f, f0-7f, f3-3f, f3-7f, f2-0f, key1-3, key1-2, f1-3f, f3-5f, f2-6f, f0-6f, f2-5f, f0-3f, f2-1f, f2-2f, f3-2f, f3-6f, f0-4f, f3-0f, f0-5f, f3-4f, key1-1 },
    keywordstyle=[4]\color{blue}\bfseries,
}

\begin{figure*}
\footnotesize
% [inline block 39: 1 envs, 10532 chars -> code_tex | \begin{lstlisting}[basicstyle=\footnotesize\ttfamily] Name: grid-x4-y8-t2-k4-l4-p100 (grid_x-4_y-8_t-2_k-4_l-4.pddl)...]

\end{figure*}

\clearpage

\lstset{
    basicstyle=\footnotesize\ttfamily,
    keywordstyle=\bfseries, % This will apply bold to all keywords
    % Define colors for different groups of keywords
    morekeywords=[1]{Domain},
    keywordstyle=[1]\color{red}\bfseries,
    morekeywords=[2]{Objects, Primitive, Goal, Initial, Plan, plan},
    keywordstyle=[2]\bfseries,
    morekeywords=[3]{putdown, move, pickup, and, loose, unlock, pickup },
    keywordstyle=[3]\color{orange}\bfseries,
    morekeywords=[4]{f0-2f, f0-0f, f2-3f, f2-7f, key2-2, f3-1f, shape0, f1-4f, shape1, f1-1f, f1-5f, f1-0f, shape2, f0-1f, f2-4f, f1-2f, key2-3, key2-0, f1-6f, f1-7f, f0-7f, f3-3f, f3-7f, f2-0f, f1-3f, f3-5f, f2-6f, f0-6f, key2-1, f2-5f, f0-3f, f2-1f, f2-2f, f3-2f, f3-6f, f0-4f, f3-0f, f0-5f, f3-4f },
    keywordstyle=[4]\color{blue}\bfseries,
}

\begin{figure*}
\footnotesize
% [inline block 40: 1 envs, 10959 chars -> code_tex | \begin{lstlisting}[basicstyle=\footnotesize\ttfamily] Name: grid-x4-y8-t3-k4-l4-p100 (grid_x-4_y-8_t-3_k-4_l-4.pddl)...]

\end{figure*}

\clearpage

\lstset{
    basicstyle=\footnotesize\ttfamily,
    keywordstyle=\bfseries, % This will apply bold to all keywords
    % Define colors for different groups of keywords
    morekeywords=[1]{Domain},
    keywordstyle=[1]\color{red}\bfseries,
    morekeywords=[2]{Objects, Primitive, Goal, Initial, Plan, plan},
    keywordstyle=[2]\bfseries,
    morekeywords=[3]{putdown, move, pickup, and, loose, unlock, pickup },
    keywordstyle=[3]\color{orange}\bfseries,
    morekeywords=[4]{f0-2f, f0-0f, f2-3f, f2-7f, key2-2, f3-1f, shape0, f1-4f, shape1, f1-1f, f1-5f, f1-0f, shape2, f0-1f, f2-4f, f1-2f, key2-3, key2-0, f1-6f, f1-7f, f0-7f, f3-3f, f3-7f, f2-0f, f1-3f, f3-5f, f2-6f, f0-6f, key2-1, f2-5f, f0-3f, f2-1f, f2-2f, f3-2f, f3-6f, f0-4f, f3-0f, f0-5f, f3-4f },
    keywordstyle=[4]\color{blue}\bfseries,
}

\begin{figure*}
\footnotesize
% [inline block 41: 1 envs, 10510 chars -> code_tex | \begin{lstlisting}[basicstyle=\footnotesize\ttfamily] Name: grid-x4-y8-t3-k4-l4-p100 (grid_x-4_y-8_t-3_k-4_l-4.pddl)...]

\end{figure*}

\clearpage

\lstset{
    basicstyle=\footnotesize\ttfamily,
    keywordstyle=\bfseries, % This will apply bold to all keywords
    % Define colors for different groups of keywords
    morekeywords=[1]{Domain},
    keywordstyle=[1]\color{red}\bfseries,
    morekeywords=[2]{Objects, Primitive, Goal, Initial, Plan, plan},
    keywordstyle=[2]\bfseries,
    morekeywords=[3]{putdown, move, pickup, and, loose, unlock, pickup },
    keywordstyle=[3]\color{orange}\bfseries,
    morekeywords=[4]{f0-2f, f0-0f, f2-3f, f2-7f, key2-2, f3-1f, shape0, f1-4f, key2-4, shape1, f1-1f, f1-5f, f1-0f, shape2, f0-1f, f2-4f, f1-2f, key2-3, key2-0, f1-6f, f1-7f, f0-7f, f3-3f, f3-7f, key2-5, f2-0f, f1-3f, f3-5f, f2-6f, f0-6f, key2-1, f2-5f, f0-3f, f2-1f, f2-2f, f3-2f, f3-6f, f0-4f, f3-0f, f0-5f, f3-4f },
    keywordstyle=[4]\color{blue}\bfseries,
}

\begin{figure*}
\footnotesize
% [inline block 42: 1 envs, 12622 chars -> code_tex | \begin{lstlisting}[basicstyle=\footnotesize\ttfamily] Name: grid-x4-y8-t3-k6-l6-p100 (grid_x-4_y-8_t-3_k-6_l-6.pddl)...]

\end{figure*}

\clearpage

\lstset{
    basicstyle=\footnotesize\ttfamily,
    keywordstyle=\bfseries, % This will apply bold to all keywords
    % Define colors for different groups of keywords
    morekeywords=[1]{Domain},
    keywordstyle=[1]\color{red}\bfseries,
    morekeywords=[2]{Objects, Primitive, Goal, Initial, Plan, plan},
    keywordstyle=[2]\bfseries,
    morekeywords=[3]{putdown, move, pickup, and, loose, unlock, pickup },
    keywordstyle=[3]\color{orange}\bfseries,
    morekeywords=[4]{f0-2f, f0-0f, f2-3f, f2-7f, key2-2, f3-1f, shape0, f1-4f, key2-4, shape1, f1-1f, f1-5f, f1-0f, shape2, f0-1f, f2-4f, f1-2f, key2-3, key2-0, f1-6f, f1-7f, f0-7f, f3-3f, f3-7f, key2-5, f2-0f, f1-3f, f3-5f, f2-6f, f0-6f, key2-1, f2-5f, f0-3f, f2-1f, f2-2f, f3-2f, f3-6f, f0-4f, f3-0f, f0-5f, f3-4f },
    keywordstyle=[4]\color{blue}\bfseries,
}

\begin{figure*}
\footnotesize
% [inline block 43: 1 envs, 12618 chars -> code_tex | \begin{lstlisting}[basicstyle=\footnotesize\ttfamily] Name: grid-x4-y8-t3-k6-l6-p100 (grid_x-4_y-8_t-3_k-6_l-6.pddl)...]

\end{figure*}

\clearpage

\lstset{
    basicstyle=\footnotesize\ttfamily,
    keywordstyle=\bfseries, % This will apply bold to all keywords
    % Define colors for different groups of keywords
    morekeywords=[1]{Domain},
    keywordstyle=[1]\color{red}\bfseries,
    morekeywords=[2]{Objects, Primitive, Goal, Initial, Plan, plan},
    keywordstyle=[2]\bfseries,
    morekeywords=[3]{putdown, move, pickup, and, loose, unlock, pickup },
    keywordstyle=[3]\color{orange}\bfseries,
    morekeywords=[4]{f0-2f, f0-0f, f2-3f, f2-7f, key2-2, f3-1f, shape0, f1-4f, key2-4, shape1, f1-1f, f1-5f, f1-0f, shape2, f0-1f, f2-4f, f1-2f, key2-3, key2-0, f1-6f, f1-7f, f0-7f, f3-3f, f3-7f, key2-5, f2-0f, f1-3f, f3-5f, f2-6f, f0-6f, key2-1, f2-5f, f0-3f, f2-1f, f2-2f, f3-2f, f3-6f, f0-4f, f3-0f, f0-5f, f3-4f },
    keywordstyle=[4]\color{blue}\bfseries,
}

\begin{figure*}
\footnotesize
% [inline block 44: 1 envs, 6198 chars -> code_tex | \begin{lstlisting}[basicstyle=\footnotesize\ttfamily] Name: grid-x4-y8-t3-k6-l8-p100 (grid_x-4_y-8_t-3_k-6_l-8.pddl)...]

\end{figure*}

\clearpage

\lstset{
    basicstyle=\footnotesize\ttfamily,
    keywordstyle=\bfseries, % This will apply bold to all keywords
    % Define colors for different groups of keywords
    morekeywords=[1]{Domain},
    keywordstyle=[1]\color{red}\bfseries,
    morekeywords=[2]{Objects, Primitive, Goal, Initial, Plan, plan},
    keywordstyle=[2]\bfseries,
    morekeywords=[3]{putdown, move, pickup, and, loose, unlock, pickup },
    keywordstyle=[3]\color{orange}\bfseries,
    morekeywords=[4]{f0-2f, f0-0f, f2-3f, f2-7f, key2-2, f3-1f, shape0, f1-4f, key2-4, shape1, f1-1f, f1-5f, f1-0f, shape2, f0-1f, f2-4f, f1-2f, key2-3, key2-0, f1-6f, f1-7f, f0-7f, f3-3f, f3-7f, key2-5, f2-0f, f1-3f, f3-5f, f2-6f, f0-6f, key2-1, f2-5f, f0-3f, f2-1f, f2-2f, f3-2f, f3-6f, f0-4f, f3-0f, f0-5f, f3-4f },
    keywordstyle=[4]\color{blue}\bfseries,
}

\begin{figure*}
\footnotesize
% [inline block 45: 1 envs, 6198 chars -> code_tex | \begin{lstlisting}[basicstyle=\footnotesize\ttfamily] Name: grid-x4-y8-t3-k6-l8-p100 (grid_x-4_y-8_t-3_k-6_l-8.pddl)...]

\end{figure*}

\clearpage

\lstset{
    basicstyle=\footnotesize\ttfamily,
    keywordstyle=\bfseries, % This will apply bold to all keywords
    % Define colors for different groups of keywords
    morekeywords=[1]{Domain},
    keywordstyle=[1]\color{red}\bfseries,
    morekeywords=[2]{Objects, Primitive, Goal, Initial, Plan, plan},
    keywordstyle=[2]\bfseries,
    morekeywords=[3]{putdown, move, pickup, and, loose, unlock, pickup },
    keywordstyle=[3]\color{orange}\bfseries,
    morekeywords=[4]{f0-2f, f0-0f, f2-3f, f2-7f, key2-2, f3-1f, shape0, f1-4f, key2-4, shape1, f1-1f, f1-5f, f1-0f, shape2, f0-1f, f2-4f, f1-2f, key2-3, key2-0, f1-6f, f1-7f, f0-7f, f3-3f, f3-7f, key2-5, f2-0f, f1-3f, f3-5f, f2-6f, f0-6f, key2-1, f2-5f, f0-3f, f2-1f, f2-2f, f3-2f, f3-6f, f0-4f, f3-0f, f0-5f, f3-4f },
    keywordstyle=[4]\color{blue}\bfseries,
}

\begin{figure*}
\footnotesize
% [inline block 46: 1 envs, 6198 chars -> code_tex | \begin{lstlisting}[basicstyle=\footnotesize\ttfamily] Name: grid-x4-y8-t3-k6-l8-p100 (grid_x-4_y-8_t-3_k-6_l-8.pddl)...]

\end{figure*}

\clearpage

\lstset{
    basicstyle=\footnotesize\ttfamily,
    keywordstyle=\bfseries, % This will apply bold to all keywords
    % Define colors for different groups of keywords
    morekeywords=[1]{Domain},
    keywordstyle=[1]\color{red}\bfseries,
    morekeywords=[2]{Objects, Primitive, Goal, Initial, Plan, plan},
    keywordstyle=[2]\bfseries,
    morekeywords=[3]{putdown, move, pickup, and, loose, unlock, pickup },
    keywordstyle=[3]\color{orange}\bfseries,
    morekeywords=[4]{f0-2f, f0-0f, f2-3f, f2-7f, key2-2, f3-1f, shape0, f1-4f, key2-4, shape1, f1-1f, f1-5f, f1-0f, shape2, f0-1f, f2-4f, f1-2f, key2-3, key2-0, f1-6f, f1-7f, f0-7f, f3-3f, f3-7f, key2-5, f2-0f, f1-3f, f3-5f, f2-6f, f0-6f, key2-1, f2-5f, f0-3f, f2-1f, f2-2f, f3-2f, f3-6f, f0-4f, f3-0f, f0-5f, f3-4f },
    keywordstyle=[4]\color{blue}\bfseries,
}

\begin{figure*}
\footnotesize
% [inline block 47: 1 envs, 6198 chars -> code_tex | \begin{lstlisting}[basicstyle=\footnotesize\ttfamily] Name: grid-x4-y8-t3-k6-l8-p100 (grid_x-4_y-8_t-3_k-6_l-8.pddl)...]

\end{figure*}

\clearpage

\lstset{
    basicstyle=\footnotesize\ttfamily,
    keywordstyle=\bfseries, % This will apply bold to all keywords
    % Define colors for different groups of keywords
    morekeywords=[1]{Domain},
    keywordstyle=[1]\color{red}\bfseries,
    morekeywords=[2]{Objects, Primitive, Goal, Initial, Plan, plan},
    keywordstyle=[2]\bfseries,
    morekeywords=[3]{putdown, move, pickup, and, loose, unlock, pickup },
    keywordstyle=[3]\color{orange}\bfseries,
    morekeywords=[4]{f0-2f, f0-0f, f2-3f, f3-1f, shape0, f1-4f, shape1, f1-1f, f1-5f, f4-5f, f1-0f, f0-1f, f2-4f, f1-2f, f4-1f, f1-6f, f3-3f, f4-4f, f2-0f, f1-3f, f3-5f, f4-0f, f4-3f, f2-6f, key0-0, f0-6f, f4-2f, f2-5f, f0-3f, f2-1f, f4-6f, f2-2f, f3-2f, f3-6f, f0-4f, f3-0f, f0-5f, f3-4f },
    keywordstyle=[4]\color{blue}\bfseries,
}

\begin{figure*}
\footnotesize
% [inline block 48: 1 envs, 4132 chars -> code_tex | \begin{lstlisting}[basicstyle=\footnotesize\ttfamily] Name: grid-x5-y7-t2-k10-l10-p100 (grid_x-5_y-7_t-2_k-1_l-1.pddl)...]

\end{figure*}

\clearpage

\lstset{
    basicstyle=\footnotesize\ttfamily,
    keywordstyle=\bfseries, % This will apply bold to all keywords
    % Define colors for different groups of keywords
    morekeywords=[1]{Domain},
    keywordstyle=[1]\color{red}\bfseries,
    morekeywords=[2]{Objects, Primitive, Goal, Initial, Plan, plan},
    keywordstyle=[2]\bfseries,
    morekeywords=[3]{putdown, move, pickup, and, loose, unlock, pickup },
    keywordstyle=[3]\color{orange}\bfseries,
    morekeywords=[4]{f0-2f, f0-0f, f2-3f, f3-1f, shape0, f1-4f, shape1, f1-1f, f1-5f, f4-5f, f1-0f, f0-1f, f2-4f, f1-2f, f4-1f, f1-6f, f3-3f, f4-4f, f2-0f, f1-3f, f3-5f, f4-0f, f4-3f, f2-6f, key0-0, f0-6f, f4-2f, f2-5f, f0-3f, f2-1f, f4-6f, f2-2f, f3-2f, f3-6f, f0-4f, f3-0f, f0-5f, f3-4f },
    keywordstyle=[4]\color{blue}\bfseries,
}

\begin{figure*}
\footnotesize
% [inline block 49: 1 envs, 4132 chars -> code_tex | \begin{lstlisting}[basicstyle=\footnotesize\ttfamily] Name: grid-x5-y7-t2-k10-l10-p100 (grid_x-5_y-7_t-2_k-1_l-1.pddl)...]

\end{figure*}

\clearpage

\lstset{
    basicstyle=\footnotesize\ttfamily,
    keywordstyle=\bfseries, % This will apply bold to all keywords
    % Define colors for different groups of keywords
    morekeywords=[1]{Domain},
    keywordstyle=[1]\color{red}\bfseries,
    morekeywords=[2]{Objects, Primitive, Goal, Initial, Plan, plan},
    keywordstyle=[2]\bfseries,
    morekeywords=[3]{putdown, move, pickup, and, loose, unlock, pickup },
    keywordstyle=[3]\color{orange}\bfseries,
    morekeywords=[4]{f0-2f, f0-0f, f2-3f, f3-1f, shape0, f1-4f, shape1, f1-1f, f1-5f, f4-5f, f1-0f, f0-1f, f2-4f, f1-2f, f4-1f, f1-6f, f3-3f, f4-4f, f2-0f, f1-3f, f3-5f, f4-0f, f4-3f, f2-6f, key0-0, f0-6f, f4-2f, f2-5f, f0-3f, f2-1f, f4-6f, f2-2f, f3-2f, f3-6f, f0-4f, f3-0f, f0-5f, f3-4f },
    keywordstyle=[4]\color{blue}\bfseries,
}

\begin{figure*}
\footnotesize
% [inline block 50: 1 envs, 4132 chars -> code_tex | \begin{lstlisting}[basicstyle=\footnotesize\ttfamily] Name: grid-x5-y7-t2-k10-l10-p100 (grid_x-5_y-7_t-2_k-1_l-1.pddl)...]

\end{figure*}

\clearpage

\lstset{
    basicstyle=\footnotesize\ttfamily,
    keywordstyle=\bfseries, % This will apply bold to all keywords
    % Define colors for different groups of keywords
    morekeywords=[1]{Domain},
    keywordstyle=[1]\color{red}\bfseries,
    morekeywords=[2]{Objects, Primitive, Goal, Initial, Plan, plan},
    keywordstyle=[2]\bfseries,
    morekeywords=[3]{putdown, move, pickup, and, loose, unlock, pickup },
    keywordstyle=[3]\color{orange}\bfseries,
    morekeywords=[4]{f0-2f, f0-0f, f2-3f, f3-1f, shape0, f1-4f, shape1, f1-1f, f1-5f, f4-5f, f1-0f, f0-1f, f2-4f, f1-2f, f4-1f, f1-6f, f3-3f, f4-4f, f2-0f, f1-3f, f3-5f, f4-0f, f4-3f, f2-6f, key0-0, f0-6f, f4-2f, f2-5f, f0-3f, f2-1f, f4-6f, f2-2f, f3-2f, f3-6f, f0-4f, f3-0f, f0-5f, f3-4f },
    keywordstyle=[4]\color{blue}\bfseries,
}

\begin{figure*}
\footnotesize
% [inline block 51: 1 envs, 4132 chars -> code_tex | \begin{lstlisting}[basicstyle=\footnotesize\ttfamily] Name: grid-x5-y7-t2-k10-l10-p100 (grid_x-5_y-7_t-2_k-1_l-1.pddl)...]

\end{figure*}

\clearpage

\lstset{
    basicstyle=\footnotesize\ttfamily,
    keywordstyle=\bfseries, % This will apply bold to all keywords
    % Define colors for different groups of keywords
    morekeywords=[1]{Domain},
    keywordstyle=[1]\color{red}\bfseries,
    morekeywords=[2]{Objects, Primitive, Goal, Initial, Plan, plan},
    keywordstyle=[2]\bfseries,
    morekeywords=[3]{putdown, move, pickup, and, loose, unlock, pickup },
    keywordstyle=[3]\color{orange}\bfseries,
    morekeywords=[4]{f0-2f, f0-0f, f2-3f, key1-0, f3-1f, shape0, f1-4f, shape1, f1-1f, f1-5f, f4-5f, key1-4, f1-0f, shape2, f0-1f, f2-4f, f1-2f, f4-1f, f1-6f, f3-3f, f4-4f, f2-0f, key1-3, key1-2, f1-3f, f3-5f, f4-0f, f4-3f, f2-6f, f0-6f, f4-2f, f2-5f, f0-3f, f2-1f, f4-6f, f2-2f, f3-2f, f3-6f, f0-4f, f3-0f, f0-5f, f3-4f, key1-1 },
    keywordstyle=[4]\color{blue}\bfseries,
}

\begin{figure*}
\footnotesize
% [inline block 52: 1 envs, 5405 chars -> code_tex | \begin{lstlisting}[basicstyle=\footnotesize\ttfamily] Name: grid-x5-y7-t3-k50-l30-p100 (grid_x-5_y-7_t-3_k-5_l-3.pddl)...]

\end{figure*}

\clearpage

\lstset{
    basicstyle=\footnotesize\ttfamily,
    keywordstyle=\bfseries, % This will apply bold to all keywords
    % Define colors for different groups of keywords
    morekeywords=[1]{Domain},
    keywordstyle=[1]\color{red}\bfseries,
    morekeywords=[2]{Objects, Primitive, Goal, Initial, Plan, plan},
    keywordstyle=[2]\bfseries,
    morekeywords=[3]{putdown, move, pickup, and, loose, unlock, pickup },
    keywordstyle=[3]\color{orange}\bfseries,
    morekeywords=[4]{f0-2f, f0-0f, f2-3f, key1-0, f3-1f, shape0, f1-4f, shape1, f1-1f, f1-5f, f4-5f, key1-4, f1-0f, shape2, f0-1f, f2-4f, f1-2f, f4-1f, f1-6f, f3-3f, f4-4f, f2-0f, key1-3, key1-2, f1-3f, f3-5f, f4-0f, f4-3f, f2-6f, f0-6f, f4-2f, f2-5f, f0-3f, f2-1f, f4-6f, f2-2f, f3-2f, f3-6f, f0-4f, f3-0f, f0-5f, f3-4f, key1-1 },
    keywordstyle=[4]\color{blue}\bfseries,
}

\begin{figure*}
\footnotesize
% [inline block 53: 1 envs, 5404 chars -> code_tex | \begin{lstlisting}[basicstyle=\footnotesize\ttfamily] Name: grid-x5-y7-t3-k50-l30-p100 (grid_x-5_y-7_t-3_k-5_l-3.pddl)...]

\end{figure*}

\clearpage

\lstset{
    basicstyle=\footnotesize\ttfamily,
    keywordstyle=\bfseries, % This will apply bold to all keywords
    % Define colors for different groups of keywords
    morekeywords=[1]{Domain},
    keywordstyle=[1]\color{red}\bfseries,
    morekeywords=[2]{Objects, Primitive, Goal, Initial, Plan, plan},
    keywordstyle=[2]\bfseries,
    morekeywords=[3]{putdown, move, pickup, and, loose, unlock, pickup },
    keywordstyle=[3]\color{orange}\bfseries,
    morekeywords=[4]{f0-2f, f0-0f, f2-3f, key1-0, f3-1f, shape0, f1-4f, shape1, f1-1f, f1-5f, f4-5f, key1-4, f1-0f, shape2, f0-1f, f2-4f, f1-2f, f4-1f, f1-6f, f3-3f, f4-4f, f2-0f, key1-3, key1-2, f1-3f, f3-5f, f4-0f, f4-3f, f2-6f, f0-6f, f4-2f, f2-5f, f0-3f, f2-1f, f4-6f, f2-2f, f3-2f, f3-6f, f0-4f, f3-0f, f0-5f, f3-4f, key1-1 },
    keywordstyle=[4]\color{blue}\bfseries,
}

\begin{figure*}
\footnotesize
% [inline block 54: 1 envs, 5404 chars -> code_tex | \begin{lstlisting}[basicstyle=\footnotesize\ttfamily] Name: grid-x5-y7-t3-k50-l30-p100 (grid_x-5_y-7_t-3_k-5_l-3.pddl)...]

\end{figure*}

\clearpage

\lstset{
    basicstyle=\footnotesize\ttfamily,
    keywordstyle=\bfseries, % This will apply bold to all keywords
    % Define colors for different groups of keywords
    morekeywords=[1]{Domain},
    keywordstyle=[1]\color{red}\bfseries,
    morekeywords=[2]{Objects, Primitive, Goal, Initial, Plan, plan},
    keywordstyle=[2]\bfseries,
    morekeywords=[3]{putdown, move, pickup, and, loose, unlock, pickup },
    keywordstyle=[3]\color{orange}\bfseries,
    morekeywords=[4]{f0-2f, f0-0f, f2-3f, key1-0, f3-1f, shape0, f1-4f, shape1, f1-1f, f1-5f, f4-5f, key1-4, f1-0f, shape2, f0-1f, f2-4f, f1-2f, f4-1f, f1-6f, f3-3f, f4-4f, f2-0f, key1-3, key1-2, f1-3f, f3-5f, f4-0f, f4-3f, f2-6f, f0-6f, f4-2f, f2-5f, f0-3f, f2-1f, f4-6f, f2-2f, f3-2f, f3-6f, f0-4f, f3-0f, f0-5f, f3-4f, key1-1 },
    keywordstyle=[4]\color{blue}\bfseries,
}

\begin{figure*}
\footnotesize
% [inline block 55: 1 envs, 5404 chars -> code_tex | \begin{lstlisting}[basicstyle=\footnotesize\ttfamily] Name: grid-x5-y7-t3-k50-l30-p100 (grid_x-5_y-7_t-3_k-5_l-3.pddl)...]

\end{figure*}

\clearpage

\lstset{
    basicstyle=\footnotesize\ttfamily,
    keywordstyle=\bfseries, % This will apply bold to all keywords
    % Define colors for different groups of keywords
    morekeywords=[1]{Domain},
    keywordstyle=[1]\color{red}\bfseries,
    morekeywords=[2]{Objects, Primitive, Goal, Initial, Plan, plan},
    keywordstyle=[2]\bfseries,
    morekeywords=[3]{putdown, move, pickup, and, loose, unlock, pickup },
    keywordstyle=[3]\color{orange}\bfseries,
    morekeywords=[4]{f0-2f, f0-0f, f2-3f, f2-7f, f3-1f, shape0, f1-4f, f2-8f, f0-8f, shape1, f1-1f, f1-5f, f4-5f, f1-0f, f0-1f, f2-4f, f1-2f, f4-1f, f1-6f, f1-7f, f0-7f, f3-3f, f4-8f, f3-7f, f4-7f, f4-4f, f3-8f, f2-0f, f1-3f, f3-5f, f4-0f, f4-3f, f2-6f, key0-0, f0-6f, f4-2f, f2-5f, f1-8f, f0-3f, f2-1f, f4-6f, f2-2f, f3-2f, f3-6f, f0-4f, f3-0f, f0-5f, f3-4f },
    keywordstyle=[4]\color{blue}\bfseries,
}

\begin{figure*}
\footnotesize
% [inline block 56: 1 envs, 5138 chars -> code_tex | \begin{lstlisting}[basicstyle=\footnotesize\ttfamily] Name: grid-x5-y9-t2-k10-l20-p100 (grid_x-5_y-9_t-2_k-1_l-2.pddl)...]

\end{figure*}

\clearpage

\lstset{
    basicstyle=\footnotesize\ttfamily,
    keywordstyle=\bfseries, % This will apply bold to all keywords
    % Define colors for different groups of keywords
    morekeywords=[1]{Domain},
    keywordstyle=[1]\color{red}\bfseries,
    morekeywords=[2]{Objects, Primitive, Goal, Initial, Plan, plan},
    keywordstyle=[2]\bfseries,
    morekeywords=[3]{putdown, move, pickup, and, loose, unlock, pickup },
    keywordstyle=[3]\color{orange}\bfseries,
    morekeywords=[4]{f0-2f, f0-0f, f2-3f, f2-7f, f3-1f, shape0, f1-4f, f2-8f, f0-8f, shape1, f1-1f, f1-5f, f4-5f, f1-0f, f0-1f, f2-4f, f1-2f, f4-1f, f1-6f, f1-7f, f0-7f, f3-3f, f4-8f, f3-7f, f4-7f, f4-4f, f3-8f, f2-0f, f1-3f, f3-5f, f4-0f, f4-3f, f2-6f, key0-0, f0-6f, f4-2f, f2-5f, f1-8f, f0-3f, f2-1f, f4-6f, f2-2f, f3-2f, f3-6f, f0-4f, f3-0f, f0-5f, f3-4f },
    keywordstyle=[4]\color{blue}\bfseries,
}

\begin{figure*}
\footnotesize
% [inline block 57: 1 envs, 5138 chars -> code_tex | \begin{lstlisting}[basicstyle=\footnotesize\ttfamily] Name: grid-x5-y9-t2-k10-l20-p100 (grid_x-5_y-9_t-2_k-1_l-2.pddl)...]

\end{figure*}

\clearpage

\lstset{
    basicstyle=\footnotesize\ttfamily,
    keywordstyle=\bfseries, % This will apply bold to all keywords
    % Define colors for different groups of keywords
    morekeywords=[1]{Domain},
    keywordstyle=[1]\color{red}\bfseries,
    morekeywords=[2]{Objects, Primitive, Goal, Initial, Plan, plan},
    keywordstyle=[2]\bfseries,
    morekeywords=[3]{putdown, move, pickup, and, loose, unlock, pickup },
    keywordstyle=[3]\color{orange}\bfseries,
    morekeywords=[4]{f0-2f, f0-0f, f2-3f, f2-7f, f3-1f, shape0, f1-4f, f2-8f, f0-8f, shape1, f1-1f, f1-5f, f4-5f, f1-0f, f0-1f, f2-4f, f1-2f, f4-1f, f1-6f, f1-7f, f0-7f, f3-3f, f4-8f, f3-7f, f4-7f, f4-4f, f3-8f, f2-0f, f1-3f, f3-5f, f4-0f, f4-3f, f2-6f, key0-0, f0-6f, f4-2f, f2-5f, f1-8f, f0-3f, f2-1f, f4-6f, f2-2f, f3-2f, f3-6f, f0-4f, f3-0f, f0-5f, f3-4f },
    keywordstyle=[4]\color{blue}\bfseries,
}

\begin{figure*}
\footnotesize
% [inline block 58: 1 envs, 5138 chars -> code_tex | \begin{lstlisting}[basicstyle=\footnotesize\ttfamily] Name: grid-x5-y9-t2-k10-l20-p100 (grid_x-5_y-9_t-2_k-1_l-2.pddl)...]

\end{figure*}

\clearpage

\lstset{
    basicstyle=\footnotesize\ttfamily,
    keywordstyle=\bfseries, % This will apply bold to all keywords
    % Define colors for different groups of keywords
    morekeywords=[1]{Domain},
    keywordstyle=[1]\color{red}\bfseries,
    morekeywords=[2]{Objects, Primitive, Goal, Initial, Plan, plan},
    keywordstyle=[2]\bfseries,
    morekeywords=[3]{putdown, move, pickup, and, loose, unlock, pickup },
    keywordstyle=[3]\color{orange}\bfseries,
    morekeywords=[4]{f0-2f, f0-0f, f2-3f, f2-7f, f3-1f, shape0, f1-4f, f2-8f, f0-8f, shape1, f1-1f, f1-5f, f4-5f, f1-0f, f0-1f, f2-4f, f1-2f, f4-1f, f1-6f, f1-7f, f0-7f, f3-3f, f4-8f, f3-7f, f4-7f, f4-4f, f3-8f, f2-0f, f1-3f, f3-5f, f4-0f, f4-3f, f2-6f, key0-0, f0-6f, f4-2f, f2-5f, f1-8f, f0-3f, f2-1f, f4-6f, f2-2f, f3-2f, f3-6f, f0-4f, f3-0f, f0-5f, f3-4f },
    keywordstyle=[4]\color{blue}\bfseries,
}

\begin{figure*}
\footnotesize
% [inline block 59: 1 envs, 5138 chars -> code_tex | \begin{lstlisting}[basicstyle=\footnotesize\ttfamily] Name: grid-x5-y9-t2-k10-l20-p100 (grid_x-5_y-9_t-2_k-1_l-2.pddl)...]

\end{figure*}

\clearpage

\lstset{
    basicstyle=\footnotesize\ttfamily,
    keywordstyle=\bfseries, % This will apply bold to all keywords
    % Define colors for different groups of keywords
    morekeywords=[1]{Domain},
    keywordstyle=[1]\color{red}\bfseries,
    morekeywords=[2]{Objects, Primitive, Goal, Initial, Plan, plan},
    keywordstyle=[2]\bfseries,
    morekeywords=[3]{putdown, move, pickup, and, loose, unlock, pickup },
    keywordstyle=[3]\color{orange}\bfseries,
    morekeywords=[4]{f0-2f, f0-0f, f2-3f, f2-7f, key1-0, f3-1f, shape0, f1-4f, f2-8f, f0-8f, shape1, f1-1f, f1-5f, f4-5f, key1-4, f1-0f, shape2, f0-1f, f2-4f, f1-2f, f4-1f, f1-6f, f1-7f, f0-7f, f3-3f, f4-8f, f3-7f, f4-7f, f4-4f, f3-8f, f2-0f, key1-3, key1-2, f1-3f, f3-5f, f4-0f, f4-3f, f2-6f, f0-6f, f4-2f, f2-5f, f1-8f, f0-3f, f2-1f, f4-6f, f2-2f, f3-2f, f3-6f, f0-4f, f3-0f, f0-5f, f3-4f, key1-1 },
    keywordstyle=[4]\color{blue}\bfseries,
}

\begin{figure*}
\footnotesize
% [inline block 60: 1 envs, 6499 chars -> code_tex | \begin{lstlisting}[basicstyle=\footnotesize\ttfamily] Name: grid-x5-y9-t3-k50-l30-p100 (grid_x-5_y-9_t-3_k-5_l-3.pddl)...]

\end{figure*}

\clearpage

\lstset{
    basicstyle=\footnotesize\ttfamily,
    keywordstyle=\bfseries, % This will apply bold to all keywords
    % Define colors for different groups of keywords
    morekeywords=[1]{Domain},
    keywordstyle=[1]\color{red}\bfseries,
    morekeywords=[2]{Objects, Primitive, Goal, Initial, Plan, plan},
    keywordstyle=[2]\bfseries,
    morekeywords=[3]{putdown, move, pickup, and, loose, unlock, pickup },
    keywordstyle=[3]\color{orange}\bfseries,
    morekeywords=[4]{f0-2f, f0-0f, f2-3f, f2-7f, key1-0, f3-1f, shape0, f1-4f, f2-8f, f0-8f, shape1, f1-1f, f1-5f, f4-5f, key1-4, f1-0f, shape2, f0-1f, f2-4f, f1-2f, f4-1f, f1-6f, f1-7f, f0-7f, f3-3f, f4-8f, f3-7f, f4-7f, f4-4f, f3-8f, f2-0f, key1-3, key1-2, f1-3f, f3-5f, f4-0f, f4-3f, f2-6f, f0-6f, f4-2f, f2-5f, f1-8f, f0-3f, f2-1f, f4-6f, f2-2f, f3-2f, f3-6f, f0-4f, f3-0f, f0-5f, f3-4f, key1-1 },
    keywordstyle=[4]\color{blue}\bfseries,
}

\begin{figure*}
\footnotesize
% [inline block 61: 1 envs, 6499 chars -> code_tex | \begin{lstlisting}[basicstyle=\footnotesize\ttfamily] Name: grid-x5-y9-t3-k50-l30-p100 (grid_x-5_y-9_t-3_k-5_l-3.pddl)...]

\end{figure*}

\clearpage

\lstset{
    basicstyle=\footnotesize\ttfamily,
    keywordstyle=\bfseries, % This will apply bold to all keywords
    % Define colors for different groups of keywords
    morekeywords=[1]{Domain},
    keywordstyle=[1]\color{red}\bfseries,
    morekeywords=[2]{Objects, Primitive, Goal, Initial, Plan, plan},
    keywordstyle=[2]\bfseries,
    morekeywords=[3]{putdown, move, pickup, and, loose, unlock, pickup },
    keywordstyle=[3]\color{orange}\bfseries,
    morekeywords=[4]{f0-2f, f0-0f, f2-3f, f2-7f, key1-0, f3-1f, shape0, f1-4f, f2-8f, f0-8f, shape1, f1-1f, f1-5f, f4-5f, key1-4, f1-0f, shape2, f0-1f, f2-4f, f1-2f, f4-1f, f1-6f, f1-7f, f0-7f, f3-3f, f4-8f, f3-7f, f4-7f, f4-4f, f3-8f, f2-0f, key1-3, key1-2, f1-3f, f3-5f, f4-0f, f4-3f, f2-6f, f0-6f, f4-2f, f2-5f, f1-8f, f0-3f, f2-1f, f4-6f, f2-2f, f3-2f, f3-6f, f0-4f, f3-0f, f0-5f, f3-4f, key1-1 },
    keywordstyle=[4]\color{blue}\bfseries,
}

\begin{figure*}
\footnotesize
% [inline block 62: 1 envs, 6499 chars -> code_tex | \begin{lstlisting}[basicstyle=\footnotesize\ttfamily] Name: grid-x5-y9-t3-k50-l30-p100 (grid_x-5_y-9_t-3_k-5_l-3.pddl)...]

\end{figure*}

\clearpage

\lstset{
    basicstyle=\footnotesize\ttfamily,
    keywordstyle=\bfseries, % This will apply bold to all keywords
    % Define colors for different groups of keywords
    morekeywords=[1]{Domain},
    keywordstyle=[1]\color{red}\bfseries,
    morekeywords=[2]{Objects, Primitive, Goal, Initial, Plan, plan},
    keywordstyle=[2]\bfseries,
    morekeywords=[3]{putdown, move, pickup, and, loose, unlock, pickup },
    keywordstyle=[3]\color{orange}\bfseries,
    morekeywords=[4]{f0-2f, f0-0f, f2-3f, f2-7f, key1-0, f3-1f, shape0, f1-4f, f2-8f, f0-8f, shape1, f1-1f, f1-5f, f4-5f, key1-4, f1-0f, shape2, f0-1f, f2-4f, f1-2f, f4-1f, f1-6f, f1-7f, f0-7f, f3-3f, f4-8f, f3-7f, f4-7f, f4-4f, f3-8f, f2-0f, key1-3, key1-2, f1-3f, f3-5f, f4-0f, f4-3f, f2-6f, f0-6f, f4-2f, f2-5f, f1-8f, f0-3f, f2-1f, f4-6f, f2-2f, f3-2f, f3-6f, f0-4f, f3-0f, f0-5f, f3-4f, key1-1 },
    keywordstyle=[4]\color{blue}\bfseries,
}

\begin{figure*}
\footnotesize
% [inline block 63: 1 envs, 6499 chars -> code_tex | \begin{lstlisting}[basicstyle=\footnotesize\ttfamily] Name: grid-x5-y9-t3-k50-l30-p100 (grid_x-5_y-9_t-3_k-5_l-3.pddl)...]

\end{figure*}

\clearpage

\lstset{
    basicstyle=\footnotesize\ttfamily,
    keywordstyle=\bfseries, % This will apply bold to all keywords
    % Define colors for different groups of keywords
    morekeywords=[1]{Domain},
    keywordstyle=[1]\color{red}\bfseries,
    morekeywords=[2]{Objects, Primitive, Goal, Initial, Plan, plan},
    keywordstyle=[2]\bfseries,
    morekeywords=[3]{putdown, move, pickup, and, loose, unlock, pickup },
    keywordstyle=[3]\color{orange}\bfseries,
    morekeywords=[4]{f0-2f, f0-0f, f2-3f, key2-2, f3-1f, shape0, f5-2f, f1-4f, key2-4, shape1, f1-1f, f1-0f, shape2, f0-1f, f2-4f, f1-2f, key2-3, key2-0, f4-1f, f5-0f, f3-3f, f4-4f, key2-5, f2-0f, f1-3f, f5-3f, f4-0f, f4-3f, f5-1f, key2-1, f4-2f, f0-3f, f2-1f, f5-4f, f2-2f, f3-2f, f0-4f, f3-0f, f3-4f },
    keywordstyle=[4]\color{blue}\bfseries,
}

\begin{figure*}
\footnotesize
% [inline block 64: 1 envs, 5284 chars -> code_tex | \begin{lstlisting}[basicstyle=\footnotesize\ttfamily] Name: grid-x6-y5-t3-k6-l9-p100 (grid_x-6_y-5_t-3_k-6_l-9.pddl)...]

\end{figure*}

\clearpage

\lstset{
    basicstyle=\footnotesize\ttfamily,
    keywordstyle=\bfseries, % This will apply bold to all keywords
    % Define colors for different groups of keywords
    morekeywords=[1]{Domain},
    keywordstyle=[1]\color{red}\bfseries,
    morekeywords=[2]{Objects, Primitive, Goal, Initial, Plan, plan},
    keywordstyle=[2]\bfseries,
    morekeywords=[3]{putdown, move, pickup, and, loose, unlock, pickup },
    keywordstyle=[3]\color{orange}\bfseries,
    morekeywords=[4]{f0-2f, f0-0f, f2-3f, key2-2, f3-1f, shape0, f5-2f, f1-4f, key2-4, shape1, f1-1f, f1-0f, shape2, f0-1f, f2-4f, f1-2f, key2-3, key2-0, f4-1f, f5-0f, f3-3f, f4-4f, key2-5, f2-0f, f1-3f, f5-3f, f4-0f, f4-3f, f5-1f, key2-1, f4-2f, f0-3f, f2-1f, f5-4f, f2-2f, f3-2f, f0-4f, f3-0f, f3-4f },
    keywordstyle=[4]\color{blue}\bfseries,
}

\begin{figure*}
\footnotesize
% [inline block 65: 1 envs, 5284 chars -> code_tex | \begin{lstlisting}[basicstyle=\footnotesize\ttfamily] Name: grid-x6-y5-t3-k6-l9-p100 (grid_x-6_y-5_t-3_k-6_l-9.pddl)...]

\end{figure*}

\clearpage

\lstset{
    basicstyle=\footnotesize\ttfamily,
    keywordstyle=\bfseries, % This will apply bold to all keywords
    % Define colors for different groups of keywords
    morekeywords=[1]{Domain},
    keywordstyle=[1]\color{red}\bfseries,
    morekeywords=[2]{Objects, Primitive, Goal, Initial, Plan, plan},
    keywordstyle=[2]\bfseries,
    morekeywords=[3]{putdown, move, pickup, and, loose, unlock, pickup },
    keywordstyle=[3]\color{orange}\bfseries,
    morekeywords=[4]{f0-2f, f0-0f, f2-3f, key2-2, f3-1f, shape0, f5-2f, f1-4f, key2-4, shape1, f1-1f, f1-0f, shape2, f0-1f, f2-4f, f1-2f, key2-3, key2-0, f4-1f, f5-0f, f3-3f, f4-4f, key2-5, f2-0f, f1-3f, f5-3f, f4-0f, f4-3f, f5-1f, key2-1, f4-2f, f0-3f, f2-1f, f5-4f, f2-2f, f3-2f, f0-4f, f3-0f, f3-4f },
    keywordstyle=[4]\color{blue}\bfseries,
}

\begin{figure*}
\footnotesize
% [inline block 66: 1 envs, 5284 chars -> code_tex | \begin{lstlisting}[basicstyle=\footnotesize\ttfamily] Name: grid-x6-y5-t3-k6-l9-p100 (grid_x-6_y-5_t-3_k-6_l-9.pddl)...]

\end{figure*}

\clearpage

\lstset{
    basicstyle=\footnotesize\ttfamily,
    keywordstyle=\bfseries, % This will apply bold to all keywords
    % Define colors for different groups of keywords
    morekeywords=[1]{Domain},
    keywordstyle=[1]\color{red}\bfseries,
    morekeywords=[2]{Objects, Primitive, Goal, Initial, Plan, plan},
    keywordstyle=[2]\bfseries,
    morekeywords=[3]{putdown, move, pickup, and, loose, unlock, pickup },
    keywordstyle=[3]\color{orange}\bfseries,
    morekeywords=[4]{f0-2f, f0-0f, f2-3f, key2-2, f3-1f, shape0, f5-2f, f1-4f, key2-4, shape1, f1-1f, f1-0f, shape2, f0-1f, f2-4f, f1-2f, key2-3, key2-0, f4-1f, f5-0f, f3-3f, f4-4f, key2-5, f2-0f, f1-3f, f5-3f, f4-0f, f4-3f, f5-1f, key2-1, f4-2f, f0-3f, f2-1f, f5-4f, f2-2f, f3-2f, f0-4f, f3-0f, f3-4f },
    keywordstyle=[4]\color{blue}\bfseries,
}

\begin{figure*}
\footnotesize
% [inline block 67: 1 envs, 5284 chars -> code_tex | \begin{lstlisting}[basicstyle=\footnotesize\ttfamily] Name: grid-x6-y5-t3-k6-l9-p100 (grid_x-6_y-5_t-3_k-6_l-9.pddl)...]

\end{figure*}

\clearpage

\lstset{
    basicstyle=\footnotesize\ttfamily,
    keywordstyle=\bfseries, % This will apply bold to all keywords
    % Define colors for different groups of keywords
    morekeywords=[1]{Domain},
    keywordstyle=[1]\color{red}\bfseries,
    morekeywords=[2]{Objects, Primitive, Goal, Initial, Plan, plan},
    keywordstyle=[2]\bfseries,
    morekeywords=[3]{putdown, move, pickup, and, loose, unlock, pickup },
    keywordstyle=[3]\color{orange}\bfseries,
    morekeywords=[4]{f0-2f, f0-0f, f2-3f, key4-0, f3-1f, shape0, f5-2f, f1-4f, f5-5f, key4-2, shape1, f1-1f, f1-5f, f4-5f, f1-0f, shape2, f0-1f, f2-4f, f1-2f, f4-1f, f5-0f, key4-3, f3-3f, f4-4f, shape4, f2-0f, f1-3f, key4-6, key4-4, f3-5f, f5-3f, key4-5, f4-0f, f4-3f, key4-1, f5-1f, f4-2f, f2-5f, shape3, f0-3f, f2-1f, f5-4f, f2-2f, f3-2f, f0-4f, f3-0f, f0-5f, f3-4f },
    keywordstyle=[4]\color{blue}\bfseries,
}

\begin{figure*}
\footnotesize
% [inline block 68: 1 envs, 5983 chars -> code_tex | \begin{lstlisting}[basicstyle=\footnotesize\ttfamily] Name: grid-x6-y6-t5-k7-l10-p100 (grid_x-6_y-6_t-5_k-7_l-10.pddl)...]

\end{figure*}

\clearpage

\lstset{
    basicstyle=\footnotesize\ttfamily,
    keywordstyle=\bfseries, % This will apply bold to all keywords
    % Define colors for different groups of keywords
    morekeywords=[1]{Domain},
    keywordstyle=[1]\color{red}\bfseries,
    morekeywords=[2]{Objects, Primitive, Goal, Initial, Plan, plan},
    keywordstyle=[2]\bfseries,
    morekeywords=[3]{putdown, move, pickup, and, loose, unlock, pickup },
    keywordstyle=[3]\color{orange}\bfseries,
    morekeywords=[4]{f0-2f, f0-0f, f2-3f, key4-0, f3-1f, shape0, f5-2f, f1-4f, f5-5f, key4-2, shape1, f1-1f, f1-5f, f4-5f, f1-0f, shape2, f0-1f, f2-4f, f1-2f, f4-1f, f5-0f, key4-3, f3-3f, f4-4f, shape4, f2-0f, f1-3f, key4-6, key4-4, f3-5f, f5-3f, key4-5, f4-0f, f4-3f, key4-1, f5-1f, f4-2f, f2-5f, shape3, f0-3f, f2-1f, f5-4f, f2-2f, f3-2f, f0-4f, f3-0f, f0-5f, f3-4f },
    keywordstyle=[4]\color{blue}\bfseries,
}

\begin{figure*}
\footnotesize
% [inline block 69: 1 envs, 5983 chars -> code_tex | \begin{lstlisting}[basicstyle=\footnotesize\ttfamily] Name: grid-x6-y6-t5-k7-l10-p100 (grid_x-6_y-6_t-5_k-7_l-10.pddl)...]

\end{figure*}

\clearpage

\lstset{
    basicstyle=\footnotesize\ttfamily,
    keywordstyle=\bfseries, % This will apply bold to all keywords
    % Define colors for different groups of keywords
    morekeywords=[1]{Domain},
    keywordstyle=[1]\color{red}\bfseries,
    morekeywords=[2]{Objects, Primitive, Goal, Initial, Plan, plan},
    keywordstyle=[2]\bfseries,
    morekeywords=[3]{putdown, move, pickup, and, loose, unlock, pickup },
    keywordstyle=[3]\color{orange}\bfseries,
    morekeywords=[4]{f0-2f, f0-0f, f2-3f, key4-0, f3-1f, shape0, f5-2f, f1-4f, f5-5f, key4-2, shape1, f1-1f, f1-5f, f4-5f, f1-0f, shape2, f0-1f, f2-4f, f1-2f, f4-1f, f5-0f, key4-3, f3-3f, f4-4f, shape4, f2-0f, f1-3f, key4-6, key4-4, f3-5f, f5-3f, key4-5, f4-0f, f4-3f, key4-1, f5-1f, f4-2f, f2-5f, shape3, f0-3f, f2-1f, f5-4f, f2-2f, f3-2f, f0-4f, f3-0f, f0-5f, f3-4f },
    keywordstyle=[4]\color{blue}\bfseries,
}

\begin{figure*}
\footnotesize
% [inline block 70: 1 envs, 5983 chars -> code_tex | \begin{lstlisting}[basicstyle=\footnotesize\ttfamily] Name: grid-x6-y6-t5-k7-l10-p100 (grid_x-6_y-6_t-5_k-7_l-10.pddl)...]

\end{figure*}

\clearpage

\lstset{
    basicstyle=\footnotesize\ttfamily,
    keywordstyle=\bfseries, % This will apply bold to all keywords
    % Define colors for different groups of keywords
    morekeywords=[1]{Domain},
    keywordstyle=[1]\color{red}\bfseries,
    morekeywords=[2]{Objects, Primitive, Goal, Initial, Plan, plan},
    keywordstyle=[2]\bfseries,
    morekeywords=[3]{putdown, move, pickup, and, loose, unlock, pickup },
    keywordstyle=[3]\color{orange}\bfseries,
    morekeywords=[4]{f0-2f, f0-0f, f2-3f, key4-0, f3-1f, shape0, f5-2f, f1-4f, f5-5f, key4-2, shape1, f1-1f, f1-5f, f4-5f, f1-0f, shape2, f0-1f, f2-4f, f1-2f, f4-1f, f5-0f, key4-3, f3-3f, f4-4f, shape4, f2-0f, f1-3f, key4-6, key4-4, f3-5f, f5-3f, key4-5, f4-0f, f4-3f, key4-1, f5-1f, f4-2f, f2-5f, shape3, f0-3f, f2-1f, f5-4f, f2-2f, f3-2f, f0-4f, f3-0f, f0-5f, f3-4f },
    keywordstyle=[4]\color{blue}\bfseries,
}

\begin{figure*}
\footnotesize
% [inline block 71: 1 envs, 5983 chars -> code_tex | \begin{lstlisting}[basicstyle=\footnotesize\ttfamily] Name: grid-x6-y6-t5-k7-l10-p100 (grid_x-6_y-6_t-5_k-7_l-10.pddl)...]

\end{figure*}

\clearpage

\lstset{
    basicstyle=\footnotesize\ttfamily,
    keywordstyle=\bfseries, % This will apply bold to all keywords
    % Define colors for different groups of keywords
    morekeywords=[1]{Domain},
    keywordstyle=[1]\color{red}\bfseries,
    morekeywords=[2]{Objects, Primitive, Goal, Initial, Plan, plan},
    keywordstyle=[2]\bfseries,
    morekeywords=[3]{putdown, move, pickup, and, loose, unlock, pickup },
    keywordstyle=[3]\color{orange}\bfseries,
    morekeywords=[4]{f0-2f, f0-0f, f2-3f, key1-0, f3-1f, shape0, f5-2f, f1-4f, f5-5f, shape1, f1-1f, f1-5f, f4-5f, key1-4, f1-0f, f0-1f, f2-4f, f1-2f, f4-1f, f5-0f, f1-6f, f3-3f, f4-4f, f2-0f, key1-3, key1-2, f1-3f, f5-6f, f3-5f, f5-3f, f4-0f, f4-3f, f2-6f, f5-1f, f0-6f, f4-2f, f2-5f, f0-3f, f2-1f, f4-6f, f5-4f, f2-2f, key1-5, f3-2f, f3-6f, f0-4f, f3-0f, f0-5f, f3-4f, key1-1 },
    keywordstyle=[4]\color{blue}\bfseries,
}

\begin{figure*}
\footnotesize
% [inline block 72: 1 envs, 10723 chars -> code_tex | \begin{lstlisting}[basicstyle=\footnotesize\ttfamily] Name: grid-x6-y7-t2-k6-l7-p100 (grid_x-6_y-7_t-2_k-6_l-7.pddl)...]

\end{figure*}

\clearpage

\lstset{
    basicstyle=\footnotesize\ttfamily,
    keywordstyle=\bfseries, % This will apply bold to all keywords
    % Define colors for different groups of keywords
    morekeywords=[1]{Domain},
    keywordstyle=[1]\color{red}\bfseries,
    morekeywords=[2]{Objects, Primitive, Goal, Initial, Plan, plan},
    keywordstyle=[2]\bfseries,
    morekeywords=[3]{putdown, move, pickup, and, loose, unlock, pickup },
    keywordstyle=[3]\color{orange}\bfseries,
    morekeywords=[4]{f0-2f, f0-0f, f2-3f, key1-0, f3-1f, shape0, f5-2f, f1-4f, f5-5f, shape1, f1-1f, f1-5f, f4-5f, key1-4, f1-0f, f0-1f, f2-4f, f1-2f, f4-1f, f5-0f, f1-6f, f3-3f, f4-4f, f2-0f, key1-3, key1-2, f1-3f, f5-6f, f3-5f, f5-3f, f4-0f, f4-3f, f2-6f, f5-1f, f0-6f, f4-2f, f2-5f, f0-3f, f2-1f, f4-6f, f5-4f, f2-2f, key1-5, f3-2f, f3-6f, f0-4f, f3-0f, f0-5f, f3-4f, key1-1 },
    keywordstyle=[4]\color{blue}\bfseries,
}

\begin{figure*}
\footnotesize
% [inline block 73: 1 envs, 11187 chars -> code_tex | \begin{lstlisting}[basicstyle=\footnotesize\ttfamily] Name: grid-x6-y7-t2-k6-l7-p100 (grid_x-6_y-7_t-2_k-6_l-7.pddl)...]

\end{figure*}

\clearpage

\lstset{
    basicstyle=\footnotesize\ttfamily,
    keywordstyle=\bfseries, % This will apply bold to all keywords
    % Define colors for different groups of keywords
    morekeywords=[1]{Domain},
    keywordstyle=[1]\color{red}\bfseries,
    morekeywords=[2]{Objects, Primitive, Goal, Initial, Plan, plan},
    keywordstyle=[2]\bfseries,
    morekeywords=[3]{putdown, move, pickup, and, loose, unlock, pickup },
    keywordstyle=[3]\color{orange}\bfseries,
    morekeywords=[4]{f0-2f, f0-0f, f2-3f, key1-0, f3-1f, f6-4f, shape0, f5-2f, f1-4f, shape1, f1-1f, f6-1f, f1-0f, f0-1f, f2-4f, f1-2f, f6-2f, f4-1f, f5-0f, f3-3f, f6-0f, f4-4f, f2-0f, key1-2, f1-3f, f5-3f, f4-0f, f4-3f, f5-1f, f4-2f, f0-3f, f2-1f, f5-4f, f2-2f, f6-3f, f3-2f, f0-4f, f3-0f, f3-4f, key1-1 },
    keywordstyle=[4]\color{blue}\bfseries,
}

\begin{figure*}
\footnotesize
% [inline block 74: 1 envs, 7488 chars -> code_tex | \begin{lstlisting}[basicstyle=\footnotesize\ttfamily] Name: grid-x7-y5-t2-k3-l4-p100 (grid_x-7_y-5_t-2_k-3_l-4.pddl)...]

\end{figure*}

\clearpage

\lstset{
    basicstyle=\footnotesize\ttfamily,
    keywordstyle=\bfseries, % This will apply bold to all keywords
    % Define colors for different groups of keywords
    morekeywords=[1]{Domain},
    keywordstyle=[1]\color{red}\bfseries,
    morekeywords=[2]{Objects, Primitive, Goal, Initial, Plan, plan},
    keywordstyle=[2]\bfseries,
    morekeywords=[3]{putdown, move, pickup, and, loose, unlock, pickup },
    keywordstyle=[3]\color{orange}\bfseries,
    morekeywords=[4]{f0-2f, f0-0f, f2-3f, key1-0, f3-1f, f6-4f, shape0, f5-2f, f1-4f, shape1, f1-1f, f6-1f, f1-0f, f0-1f, f2-4f, f1-2f, f6-2f, f4-1f, f5-0f, f3-3f, f6-0f, f4-4f, f2-0f, key1-2, f1-3f, f5-3f, f4-0f, f4-3f, f5-1f, f4-2f, f0-3f, f2-1f, f5-4f, f2-2f, f6-3f, f3-2f, f0-4f, f3-0f, f3-4f, key1-1 },
    keywordstyle=[4]\color{blue}\bfseries,
}

\begin{figure*}
\footnotesize
% [inline block 75: 1 envs, 7858 chars -> code_tex | \begin{lstlisting}[basicstyle=\footnotesize\ttfamily] Name: grid-x7-y5-t2-k3-l4-p100 (grid_x-7_y-5_t-2_k-3_l-4.pddl)...]

\end{figure*}

\clearpage

\lstset{
    basicstyle=\footnotesize\ttfamily,
    keywordstyle=\bfseries, % This will apply bold to all keywords
    % Define colors for different groups of keywords
    morekeywords=[1]{Domain},
    keywordstyle=[1]\color{red}\bfseries,
    morekeywords=[2]{Objects, Primitive, Goal, Initial, Plan, plan},
    keywordstyle=[2]\bfseries,
    morekeywords=[3]{putdown, move, pickup, and, loose, unlock, pickup },
    keywordstyle=[3]\color{orange}\bfseries,
    morekeywords=[4]{f0-2f, f0-0f, f2-3f, f2-7f, f3-1f, f6-4f, shape0, f5-2f, f1-4f, f5-5f, f2-8f, f0-8f, shape1, f1-1f, f6-1f, f1-5f, f4-5f, f1-0f, f6-6f, f0-1f, f2-4f, f6-5f, f1-2f, f6-2f, f4-1f, f5-0f, f1-6f, f1-7f, f5-8f, f0-7f, f3-3f, f4-8f, f3-7f, f4-7f, f6-0f, f4-4f, f6-7f, f3-8f, f2-0f, f1-3f, f6-8f, f5-6f, f5-7f, f3-5f, f5-3f, f4-0f, f4-3f, f2-6f, key0-0, f5-1f, f0-6f, f4-2f, f2-5f, f1-8f, f0-3f, f2-1f, f4-6f, f5-4f, f2-2f, f6-3f, f3-2f, f3-6f, f0-4f, f3-0f, f0-5f, f3-4f },
    keywordstyle=[4]\color{blue}\bfseries,
}

\begin{figure*}
\footnotesize
% [inline block 76: 1 envs, 7211 chars -> code_tex | \begin{lstlisting}[basicstyle=\footnotesize\ttfamily] Name: grid-x7-y9-t2-k10-l10-p100 (grid_x-7_y-9_t-2_k-1_l-1.pddl)...]

\end{figure*}

\clearpage

\lstset{
    basicstyle=\footnotesize\ttfamily,
    keywordstyle=\bfseries, % This will apply bold to all keywords
    % Define colors for different groups of keywords
    morekeywords=[1]{Domain},
    keywordstyle=[1]\color{red}\bfseries,
    morekeywords=[2]{Objects, Primitive, Goal, Initial, Plan, plan},
    keywordstyle=[2]\bfseries,
    morekeywords=[3]{putdown, move, pickup, and, loose, unlock, pickup },
    keywordstyle=[3]\color{orange}\bfseries,
    morekeywords=[4]{f0-2f, f0-0f, f2-3f, f2-7f, f3-1f, f6-4f, shape0, f5-2f, f1-4f, f5-5f, f2-8f, f0-8f, shape1, f1-1f, f6-1f, f1-5f, f4-5f, f1-0f, f6-6f, f0-1f, f2-4f, f6-5f, f1-2f, f6-2f, f4-1f, f5-0f, f1-6f, f1-7f, f5-8f, f0-7f, f3-3f, f4-8f, f3-7f, f4-7f, f6-0f, f4-4f, f6-7f, f3-8f, f2-0f, f1-3f, f6-8f, f5-6f, f5-7f, f3-5f, f5-3f, f4-0f, f4-3f, f2-6f, key0-0, f5-1f, f0-6f, f4-2f, f2-5f, f1-8f, f0-3f, f2-1f, f4-6f, f5-4f, f2-2f, f6-3f, f3-2f, f3-6f, f0-4f, f3-0f, f0-5f, f3-4f },
    keywordstyle=[4]\color{blue}\bfseries,
}

\begin{figure*}
\footnotesize
% [inline block 77: 1 envs, 7211 chars -> code_tex | \begin{lstlisting}[basicstyle=\footnotesize\ttfamily] Name: grid-x7-y9-t2-k10-l10-p100 (grid_x-7_y-9_t-2_k-1_l-1.pddl)...]

\end{figure*}

\clearpage

\lstset{
    basicstyle=\footnotesize\ttfamily,
    keywordstyle=\bfseries, % This will apply bold to all keywords
    % Define colors for different groups of keywords
    morekeywords=[1]{Domain},
    keywordstyle=[1]\color{red}\bfseries,
    morekeywords=[2]{Objects, Primitive, Goal, Initial, Plan, plan},
    keywordstyle=[2]\bfseries,
    morekeywords=[3]{putdown, move, pickup, and, loose, unlock, pickup },
    keywordstyle=[3]\color{orange}\bfseries,
    morekeywords=[4]{f0-2f, f0-0f, f2-3f, f2-7f, f3-1f, f6-4f, shape0, f5-2f, f1-4f, f5-5f, f2-8f, f0-8f, shape1, f1-1f, f6-1f, f1-5f, f4-5f, f1-0f, f6-6f, f0-1f, f2-4f, f6-5f, f1-2f, f6-2f, f4-1f, f5-0f, f1-6f, f1-7f, f5-8f, f0-7f, f3-3f, f4-8f, f3-7f, f4-7f, f6-0f, f4-4f, f6-7f, f3-8f, f2-0f, f1-3f, f6-8f, f5-6f, f5-7f, f3-5f, f5-3f, f4-0f, f4-3f, f2-6f, key0-0, f5-1f, f0-6f, f4-2f, f2-5f, f1-8f, f0-3f, f2-1f, f4-6f, f5-4f, f2-2f, f6-3f, f3-2f, f3-6f, f0-4f, f3-0f, f0-5f, f3-4f },
    keywordstyle=[4]\color{blue}\bfseries,
}

\begin{figure*}
\footnotesize
% [inline block 78: 1 envs, 7211 chars -> code_tex | \begin{lstlisting}[basicstyle=\footnotesize\ttfamily] Name: grid-x7-y9-t2-k10-l10-p100 (grid_x-7_y-9_t-2_k-1_l-1.pddl)...]

\end{figure*}

\clearpage

\lstset{
    basicstyle=\footnotesize\ttfamily,
    keywordstyle=\bfseries, % This will apply bold to all keywords
    % Define colors for different groups of keywords
    morekeywords=[1]{Domain},
    keywordstyle=[1]\color{red}\bfseries,
    morekeywords=[2]{Objects, Primitive, Goal, Initial, Plan, plan},
    keywordstyle=[2]\bfseries,
    morekeywords=[3]{putdown, move, pickup, and, loose, unlock, pickup },
    keywordstyle=[3]\color{orange}\bfseries,
    morekeywords=[4]{f0-2f, f0-0f, f2-3f, f2-7f, f3-1f, f6-4f, shape0, f5-2f, f1-4f, f5-5f, f2-8f, f0-8f, shape1, f1-1f, f6-1f, f1-5f, f4-5f, f1-0f, f6-6f, f0-1f, f2-4f, f6-5f, f1-2f, f6-2f, f4-1f, f5-0f, f1-6f, f1-7f, f5-8f, f0-7f, f3-3f, f4-8f, f3-7f, f4-7f, f6-0f, f4-4f, f6-7f, f3-8f, f2-0f, f1-3f, f6-8f, f5-6f, f5-7f, f3-5f, f5-3f, f4-0f, f4-3f, f2-6f, key0-0, f5-1f, f0-6f, f4-2f, f2-5f, f1-8f, f0-3f, f2-1f, f4-6f, f5-4f, f2-2f, f6-3f, f3-2f, f3-6f, f0-4f, f3-0f, f0-5f, f3-4f },
    keywordstyle=[4]\color{blue}\bfseries,
}

\begin{figure*}
\footnotesize
% [inline block 79: 1 envs, 7211 chars -> code_tex | \begin{lstlisting}[basicstyle=\footnotesize\ttfamily] Name: grid-x7-y9-t2-k10-l10-p100 (grid_x-7_y-9_t-2_k-1_l-1.pddl)...]

\end{figure*}

\clearpage

\lstset{
    basicstyle=\footnotesize\ttfamily,
    keywordstyle=\bfseries, % This will apply bold to all keywords
    % Define colors for different groups of keywords
    morekeywords=[1]{Domain},
    keywordstyle=[1]\color{red}\bfseries,
    morekeywords=[2]{Objects, Primitive, Goal, Initial, Plan, plan},
    keywordstyle=[2]\bfseries,
    morekeywords=[3]{putdown, move, pickup, and, loose, unlock, pickup },
    keywordstyle=[3]\color{orange}\bfseries,
    morekeywords=[4]{f0-2f, f0-0f, f2-3f, f2-7f, key1-0, f3-1f, f6-4f, shape0, f5-2f, f1-4f, f5-5f, f2-8f, f0-8f, shape1, f1-1f, f6-1f, f1-5f, f4-5f, key1-4, f1-0f, f6-6f, shape2, f0-1f, f2-4f, f6-5f, f1-2f, f6-2f, f4-1f, f5-0f, f1-6f, f1-7f, f5-8f, f0-7f, f3-3f, f4-8f, f3-7f, f4-7f, f6-0f, f4-4f, f6-7f, f3-8f, f2-0f, key1-3, key1-2, f1-3f, f6-8f, f5-6f, f5-7f, f3-5f, f5-3f, f4-0f, f4-3f, f2-6f, f5-1f, f0-6f, f4-2f, f2-5f, f1-8f, f0-3f, f2-1f, f4-6f, f5-4f, f2-2f, f6-3f, f3-2f, f3-6f, f0-4f, f3-0f, f0-5f, f3-4f, key1-1 },
    keywordstyle=[4]\color{blue}\bfseries,
}

\begin{figure*}
\footnotesize
% [inline block 80: 1 envs, 8754 chars -> code_tex | \begin{lstlisting}[basicstyle=\footnotesize\ttfamily] Name: grid-x7-y9-t3-k50-l30-p100 (grid_x-7_y-9_t-3_k-5_l-3.pddl)...]

\end{figure*}

\clearpage

\lstset{
    basicstyle=\footnotesize\ttfamily,
    keywordstyle=\bfseries, % This will apply bold to all keywords
    % Define colors for different groups of keywords
    morekeywords=[1]{Domain},
    keywordstyle=[1]\color{red}\bfseries,
    morekeywords=[2]{Objects, Primitive, Goal, Initial, Plan, plan},
    keywordstyle=[2]\bfseries,
    morekeywords=[3]{putdown, move, pickup, and, loose, unlock, pickup },
    keywordstyle=[3]\color{orange}\bfseries,
    morekeywords=[4]{f0-2f, f0-0f, f2-3f, f2-7f, key1-0, f3-1f, f6-4f, shape0, f5-2f, f1-4f, f5-5f, f2-8f, f0-8f, shape1, f1-1f, f6-1f, f1-5f, f4-5f, key1-4, f1-0f, f6-6f, shape2, f0-1f, f2-4f, f6-5f, f1-2f, f6-2f, f4-1f, f5-0f, f1-6f, f1-7f, f5-8f, f0-7f, f3-3f, f4-8f, f3-7f, f4-7f, f6-0f, f4-4f, f6-7f, f3-8f, f2-0f, key1-3, key1-2, f1-3f, f6-8f, f5-6f, f5-7f, f3-5f, f5-3f, f4-0f, f4-3f, f2-6f, f5-1f, f0-6f, f4-2f, f2-5f, f1-8f, f0-3f, f2-1f, f4-6f, f5-4f, f2-2f, f6-3f, f3-2f, f3-6f, f0-4f, f3-0f, f0-5f, f3-4f, key1-1 },
    keywordstyle=[4]\color{blue}\bfseries,
}

\begin{figure*}
\footnotesize
% [inline block 81: 1 envs, 8754 chars -> code_tex | \begin{lstlisting}[basicstyle=\footnotesize\ttfamily] Name: grid-x7-y9-t3-k50-l30-p100 (grid_x-7_y-9_t-3_k-5_l-3.pddl)...]

\end{figure*}

\clearpage

\lstset{
    basicstyle=\footnotesize\ttfamily,
    keywordstyle=\bfseries, % This will apply bold to all keywords
    % Define colors for different groups of keywords
    morekeywords=[1]{Domain},
    keywordstyle=[1]\color{red}\bfseries,
    morekeywords=[2]{Objects, Primitive, Goal, Initial, Plan, plan},
    keywordstyle=[2]\bfseries,
    morekeywords=[3]{putdown, move, pickup, and, loose, unlock, pickup },
    keywordstyle=[3]\color{orange}\bfseries,
    morekeywords=[4]{f0-2f, f0-0f, f2-3f, f2-7f, key1-0, f3-1f, f6-4f, shape0, f5-2f, f1-4f, f5-5f, f2-8f, f0-8f, shape1, f1-1f, f6-1f, f1-5f, f4-5f, key1-4, f1-0f, f6-6f, shape2, f0-1f, f2-4f, f6-5f, f1-2f, f6-2f, f4-1f, f5-0f, f1-6f, f1-7f, f5-8f, f0-7f, f3-3f, f4-8f, f3-7f, f4-7f, f6-0f, f4-4f, f6-7f, f3-8f, f2-0f, key1-3, key1-2, f1-3f, f6-8f, f5-6f, f5-7f, f3-5f, f5-3f, f4-0f, f4-3f, f2-6f, f5-1f, f0-6f, f4-2f, f2-5f, f1-8f, f0-3f, f2-1f, f4-6f, f5-4f, f2-2f, f6-3f, f3-2f, f3-6f, f0-4f, f3-0f, f0-5f, f3-4f, key1-1 },
    keywordstyle=[4]\color{blue}\bfseries,
}

\begin{figure*}
\footnotesize
% [inline block 82: 1 envs, 8754 chars -> code_tex | \begin{lstlisting}[basicstyle=\footnotesize\ttfamily] Name: grid-x7-y9-t3-k50-l30-p100 (grid_x-7_y-9_t-3_k-5_l-3.pddl)...]

\end{figure*}

\clearpage

\lstset{
    basicstyle=\footnotesize\ttfamily,
    keywordstyle=\bfseries, % This will apply bold to all keywords
    % Define colors for different groups of keywords
    morekeywords=[1]{Domain},
    keywordstyle=[1]\color{red}\bfseries,
    morekeywords=[2]{Objects, Primitive, Goal, Initial, Plan, plan},
    keywordstyle=[2]\bfseries,
    morekeywords=[3]{putdown, move, pickup, and, loose, unlock, pickup },
    keywordstyle=[3]\color{orange}\bfseries,
    morekeywords=[4]{f0-2f, f0-0f, f2-3f, f2-7f, key1-0, f3-1f, f6-4f, shape0, f5-2f, f1-4f, f5-5f, f2-8f, f0-8f, shape1, f1-1f, f6-1f, f1-5f, f4-5f, key1-4, f1-0f, f6-6f, shape2, f0-1f, f2-4f, f6-5f, f1-2f, f6-2f, f4-1f, f5-0f, f1-6f, f1-7f, f5-8f, f0-7f, f3-3f, f4-8f, f3-7f, f4-7f, f6-0f, f4-4f, f6-7f, f3-8f, f2-0f, key1-3, key1-2, f1-3f, f6-8f, f5-6f, f5-7f, f3-5f, f5-3f, f4-0f, f4-3f, f2-6f, f5-1f, f0-6f, f4-2f, f2-5f, f1-8f, f0-3f, f2-1f, f4-6f, f5-4f, f2-2f, f6-3f, f3-2f, f3-6f, f0-4f, f3-0f, f0-5f, f3-4f, key1-1 },
    keywordstyle=[4]\color{blue}\bfseries,
}

\begin{figure*}
\footnotesize
% [inline block 83: 1 envs, 8754 chars -> code_tex | \begin{lstlisting}[basicstyle=\footnotesize\ttfamily] Name: grid-x7-y9-t3-k50-l30-p100 (grid_x-7_y-9_t-3_k-5_l-3.pddl)...]

\end{figure*}

\clearpage

\lstset{
    basicstyle=\footnotesize\ttfamily,
    keywordstyle=\bfseries, % This will apply bold to all keywords
    % Define colors for different groups of keywords
    morekeywords=[1]{Domain},
    keywordstyle=[1]\color{red}\bfseries,
    morekeywords=[2]{Objects, Primitive, Goal, Initial, Plan, plan},
    keywordstyle=[2]\bfseries,
    morekeywords=[3]{putdown, move, pickup, and, loose, unlock, pickup },
    keywordstyle=[3]\color{orange}\bfseries,
    morekeywords=[4]{f0-2f, f0-0f, f2-3f, f3-6f, f7-4f, f3-1f, f6-4f, shape0, f5-2f, f1-4f, f5-5f, key3-0, shape1, f1-1f, f6-1f, f7-0f, f1-5f, f4-5f, f1-0f, f6-6f, shape2, f0-1f, f2-4f, f6-5f, f7-6f, f1-2f, f6-2f, f4-1f, f5-0f, f1-6f, key3-1, f7-5f, f3-3f, key3-3, f6-0f, f4-4f, f2-0f, f1-3f, f5-6f, f3-5f, f5-3f, f4-0f, f4-3f, f2-6f, f7-3f, f5-1f, f0-6f, f4-2f, f2-5f, key3-2, shape3, f0-3f, f2-1f, f4-6f, f5-4f, f2-2f, f7-2f, f6-3f, f3-2f, f7-1f, f0-4f, f3-0f, f0-5f, f3-4f },
    keywordstyle=[4]\color{blue}\bfseries,
}

\begin{figure*}
\footnotesize
% [inline block 84: 1 envs, 7800 chars -> code_tex | \begin{lstlisting}[basicstyle=\footnotesize\ttfamily] Name: grid-x8-y7-t4-k4-l6-p100 (grid_x-8_y-7_t-4_k-4_l-6.pddl)...]

\end{figure*}

\clearpage

\lstset{
    basicstyle=\footnotesize\ttfamily,
    keywordstyle=\bfseries, % This will apply bold to all keywords
    % Define colors for different groups of keywords
    morekeywords=[1]{Domain},
    keywordstyle=[1]\color{red}\bfseries,
    morekeywords=[2]{Objects, Primitive, Goal, Initial, Plan, plan},
    keywordstyle=[2]\bfseries,
    morekeywords=[3]{putdown, move, pickup, and, loose, unlock, pickup },
    keywordstyle=[3]\color{orange}\bfseries,
    morekeywords=[4]{f0-2f, f0-0f, f2-3f, f3-6f, f7-4f, f3-1f, f6-4f, shape0, f5-2f, f1-4f, f5-5f, key3-0, shape1, f1-1f, f6-1f, f7-0f, f1-5f, f4-5f, f1-0f, f6-6f, shape2, f0-1f, f2-4f, f6-5f, f7-6f, f1-2f, f6-2f, f4-1f, f5-0f, f1-6f, key3-1, f7-5f, f3-3f, key3-3, f6-0f, f4-4f, f2-0f, f1-3f, f5-6f, f3-5f, f5-3f, f4-0f, f4-3f, f2-6f, f7-3f, f5-1f, f0-6f, f4-2f, f2-5f, key3-2, shape3, f0-3f, f2-1f, f4-6f, f5-4f, f2-2f, f7-2f, f6-3f, f3-2f, f7-1f, f0-4f, f3-0f, f0-5f, f3-4f },
    keywordstyle=[4]\color{blue}\bfseries,
}

\begin{figure*}
\footnotesize
% [inline block 85: 1 envs, 7800 chars -> code_tex | \begin{lstlisting}[basicstyle=\footnotesize\ttfamily] Name: grid-x8-y7-t4-k4-l6-p100 (grid_x-8_y-7_t-4_k-4_l-6.pddl)...]

\end{figure*}

\clearpage

\lstset{
    basicstyle=\footnotesize\ttfamily,
    keywordstyle=\bfseries, % This will apply bold to all keywords
    % Define colors for different groups of keywords
    morekeywords=[1]{Domain},
    keywordstyle=[1]\color{red}\bfseries,
    morekeywords=[2]{Objects, Primitive, Goal, Initial, Plan, plan},
    keywordstyle=[2]\bfseries,
    morekeywords=[3]{putdown, move, pickup, and, loose, unlock, pickup },
    keywordstyle=[3]\color{orange}\bfseries,
    morekeywords=[4]{f0-2f, f0-0f, f2-3f, f3-6f, f7-4f, f3-1f, f6-4f, shape0, f5-2f, f1-4f, f5-5f, key3-0, shape1, f1-1f, f6-1f, f7-0f, f1-5f, f4-5f, f1-0f, f6-6f, shape2, f0-1f, f2-4f, f6-5f, f7-6f, f1-2f, f6-2f, f4-1f, f5-0f, f1-6f, key3-1, f7-5f, f3-3f, key3-3, f6-0f, f4-4f, f2-0f, f1-3f, f5-6f, f3-5f, f5-3f, f4-0f, f4-3f, f2-6f, f7-3f, f5-1f, f0-6f, f4-2f, f2-5f, key3-2, shape3, f0-3f, f2-1f, f4-6f, f5-4f, f2-2f, f7-2f, f6-3f, f3-2f, f7-1f, f0-4f, f3-0f, f0-5f, f3-4f },
    keywordstyle=[4]\color{blue}\bfseries,
}

\begin{figure*}
\footnotesize
% [inline block 86: 1 envs, 7800 chars -> code_tex | \begin{lstlisting}[basicstyle=\footnotesize\ttfamily] Name: grid-x8-y7-t4-k4-l6-p100 (grid_x-8_y-7_t-4_k-4_l-6.pddl)...]

\end{figure*}

\clearpage

\lstset{
    basicstyle=\footnotesize\ttfamily,
    keywordstyle=\bfseries, % This will apply bold to all keywords
    % Define colors for different groups of keywords
    morekeywords=[1]{Domain},
    keywordstyle=[1]\color{red}\bfseries,
    morekeywords=[2]{Objects, Primitive, Goal, Initial, Plan, plan},
    keywordstyle=[2]\bfseries,
    morekeywords=[3]{putdown, move, pickup, and, loose, unlock, pickup },
    keywordstyle=[3]\color{orange}\bfseries,
    morekeywords=[4]{f0-2f, f0-0f, f2-3f, f3-6f, f7-4f, f3-1f, f6-4f, shape0, f5-2f, f1-4f, f5-5f, key3-0, shape1, f1-1f, f6-1f, f7-0f, f1-5f, f4-5f, f1-0f, f6-6f, shape2, f0-1f, f2-4f, f6-5f, f7-6f, f1-2f, f6-2f, f4-1f, f5-0f, f1-6f, key3-1, f7-5f, f3-3f, key3-3, f6-0f, f4-4f, f2-0f, f1-3f, f5-6f, f3-5f, f5-3f, f4-0f, f4-3f, f2-6f, f7-3f, f5-1f, f0-6f, f4-2f, f2-5f, key3-2, shape3, f0-3f, f2-1f, f4-6f, f5-4f, f2-2f, f7-2f, f6-3f, f3-2f, f7-1f, f0-4f, f3-0f, f0-5f, f3-4f },
    keywordstyle=[4]\color{blue}\bfseries,
}

\begin{figure*}
\footnotesize
% [inline block 87: 1 envs, 7800 chars -> code_tex | \begin{lstlisting}[basicstyle=\footnotesize\ttfamily] Name: grid-x8-y7-t4-k4-l6-p100 (grid_x-8_y-7_t-4_k-4_l-6.pddl)...]

\end{figure*}

\clearpage

\lstset{
    basicstyle=\footnotesize\ttfamily,
    keywordstyle=\bfseries, % This will apply bold to all keywords
    % Define colors for different groups of keywords
    morekeywords=[1]{Domain},
    keywordstyle=[1]\color{red}\bfseries,
    morekeywords=[2]{Objects, Primitive, Goal, Initial, Plan, plan},
    keywordstyle=[2]\bfseries,
    morekeywords=[3]{putdown, move, pickup, and, loose, unlock, pickup },
    keywordstyle=[3]\color{orange}\bfseries,
    morekeywords=[4]{f0-2f, f0-0f, f2-3f, f3-6f, f7-4f, f3-1f, f6-4f, f2-7f, f5-2f, f1-4f, f5-5f, shape0, f1-1f, f6-1f, f7-0f, f1-5f, f4-5f, f1-0f, f6-6f, f0-1f, f2-4f, f6-5f, f7-6f, f1-2f, f6-2f, f4-1f, f5-0f, f1-6f, key0-3, f1-7f, key0-1, key0-2, f0-7f, f7-5f, f3-3f, f3-7f, f4-7f, f6-0f, f4-4f, f6-7f, f2-0f, f7-7f, f1-3f, f5-6f, f5-7f, f3-5f, f5-3f, f4-0f, f4-3f, f2-6f, key0-0, f7-3f, f5-1f, f0-6f, f4-2f, f2-5f, f0-3f, f2-1f, f4-6f, f5-4f, f2-2f, f7-2f, f6-3f, f3-2f, f7-1f, f0-4f, f3-0f, f0-5f, f3-4f },
    keywordstyle=[4]\color{blue}\bfseries,
}

\begin{figure*}
\footnotesize
% [inline block 88: 1 envs, 8457 chars -> code_tex | \begin{lstlisting}[basicstyle=\footnotesize\ttfamily] Name: grid-x8-y8-t1-k4-l4-p100 (grid_x-8_y-8_t-1_k-4_l-4.pddl)...]

\end{figure*}

\clearpage

\lstset{
    basicstyle=\footnotesize\ttfamily,
    keywordstyle=\bfseries, % This will apply bold to all keywords
    % Define colors for different groups of keywords
    morekeywords=[1]{Domain},
    keywordstyle=[1]\color{red}\bfseries,
    morekeywords=[2]{Objects, Primitive, Goal, Initial, Plan, plan},
    keywordstyle=[2]\bfseries,
    morekeywords=[3]{putdown, move, pickup, and, loose, unlock, pickup },
    keywordstyle=[3]\color{orange}\bfseries,
    morekeywords=[4]{f0-2f, f0-0f, f2-3f, f3-6f, f7-4f, f3-1f, f6-4f, f2-7f, f5-2f, f1-4f, f5-5f, shape0, f1-1f, f6-1f, f7-0f, f1-5f, f4-5f, f1-0f, f6-6f, f0-1f, f2-4f, f6-5f, f7-6f, f1-2f, f6-2f, f4-1f, f5-0f, f1-6f, key0-3, f1-7f, key0-1, key0-2, f0-7f, f7-5f, f3-3f, f3-7f, f4-7f, f6-0f, f4-4f, f6-7f, f2-0f, f7-7f, f1-3f, f5-6f, f5-7f, f3-5f, f5-3f, f4-0f, f4-3f, f2-6f, key0-0, f7-3f, f5-1f, f0-6f, f4-2f, f2-5f, f0-3f, f2-1f, f4-6f, f5-4f, f2-2f, f7-2f, f6-3f, f3-2f, f7-1f, f0-4f, f3-0f, f0-5f, f3-4f },
    keywordstyle=[4]\color{blue}\bfseries,
}

\begin{figure*}
\footnotesize
% [inline block 89: 1 envs, 8457 chars -> code_tex | \begin{lstlisting}[basicstyle=\footnotesize\ttfamily] Name: grid-x8-y8-t1-k4-l4-p100 (grid_x-8_y-8_t-1_k-4_l-4.pddl)...]

\end{figure*}

\clearpage

\lstset{
    basicstyle=\footnotesize\ttfamily,
    keywordstyle=\bfseries, % This will apply bold to all keywords
    % Define colors for different groups of keywords
    morekeywords=[1]{Domain},
    keywordstyle=[1]\color{red}\bfseries,
    morekeywords=[2]{Objects, Primitive, Goal, Initial, Plan, plan},
    keywordstyle=[2]\bfseries,
    morekeywords=[3]{putdown, move, pickup, and, loose, unlock, pickup },
    keywordstyle=[3]\color{orange}\bfseries,
    morekeywords=[4]{f0-2f, f0-0f, f2-3f, f3-6f, f7-4f, f3-1f, f6-4f, f2-7f, f5-2f, f1-4f, f5-5f, shape0, f1-1f, f6-1f, f7-0f, f1-5f, f4-5f, f1-0f, f6-6f, f0-1f, f2-4f, f6-5f, f7-6f, f1-2f, f6-2f, f4-1f, f5-0f, f1-6f, key0-3, f1-7f, key0-1, key0-2, f0-7f, f7-5f, f3-3f, f3-7f, f4-7f, f6-0f, f4-4f, f6-7f, f2-0f, f7-7f, f1-3f, f5-6f, f5-7f, f3-5f, f5-3f, f4-0f, f4-3f, f2-6f, key0-0, f7-3f, f5-1f, f0-6f, f4-2f, f2-5f, f0-3f, f2-1f, f4-6f, f5-4f, f2-2f, f7-2f, f6-3f, f3-2f, f7-1f, f0-4f, f3-0f, f0-5f, f3-4f },
    keywordstyle=[4]\color{blue}\bfseries,
}

\begin{figure*}
\footnotesize
% [inline block 90: 1 envs, 8457 chars -> code_tex | \begin{lstlisting}[basicstyle=\footnotesize\ttfamily] Name: grid-x8-y8-t1-k4-l4-p100 (grid_x-8_y-8_t-1_k-4_l-4.pddl)...]

\end{figure*}

\clearpage

\lstset{
    basicstyle=\footnotesize\ttfamily,
    keywordstyle=\bfseries, % This will apply bold to all keywords
    % Define colors for different groups of keywords
    morekeywords=[1]{Domain},
    keywordstyle=[1]\color{red}\bfseries,
    morekeywords=[2]{Objects, Primitive, Goal, Initial, Plan, plan},
    keywordstyle=[2]\bfseries,
    morekeywords=[3]{putdown, move, pickup, and, loose, unlock, pickup },
    keywordstyle=[3]\color{orange}\bfseries,
    morekeywords=[4]{f0-2f, f0-0f, f2-3f, f3-6f, f7-4f, f3-1f, f6-4f, f2-7f, f5-2f, f1-4f, f5-5f, shape0, f1-1f, f6-1f, f7-0f, f1-5f, f4-5f, f1-0f, f6-6f, f0-1f, f2-4f, f6-5f, f7-6f, f1-2f, f6-2f, f4-1f, f5-0f, f1-6f, key0-3, f1-7f, key0-1, key0-2, f0-7f, f7-5f, f3-3f, f3-7f, f4-7f, f6-0f, f4-4f, f6-7f, f2-0f, f7-7f, f1-3f, f5-6f, f5-7f, f3-5f, f5-3f, f4-0f, f4-3f, f2-6f, key0-0, f7-3f, f5-1f, f0-6f, f4-2f, f2-5f, f0-3f, f2-1f, f4-6f, f5-4f, f2-2f, f7-2f, f6-3f, f3-2f, f7-1f, f0-4f, f3-0f, f0-5f, f3-4f },
    keywordstyle=[4]\color{blue}\bfseries,
}

\begin{figure*}
\footnotesize
% [inline block 91: 1 envs, 8457 chars -> code_tex | \begin{lstlisting}[basicstyle=\footnotesize\ttfamily] Name: grid-x8-y8-t1-k4-l4-p100 (grid_x-8_y-8_t-1_k-4_l-4.pddl)...]

\end{figure*}

\clearpage

\lstset{
    basicstyle=\footnotesize\ttfamily,
    keywordstyle=\bfseries, % This will apply bold to all keywords
    % Define colors for different groups of keywords
    morekeywords=[1]{Domain},
    keywordstyle=[1]\color{red}\bfseries,
    morekeywords=[2]{Objects, Primitive, Goal, Initial, Plan, plan},
    keywordstyle=[2]\bfseries,
    morekeywords=[3]{putdown, move, pickup, and, loose, unlock, pickup },
    keywordstyle=[3]\color{orange}\bfseries,
    morekeywords=[4]{f0-2f, f0-0f, f2-3f, f3-6f, f7-4f, f3-1f, f6-4f, f2-7f, f5-2f, f1-4f, f5-5f, shape0, key1-0, shape1, f1-1f, f6-1f, f7-0f, f1-5f, f4-5f, f1-0f, f6-6f, f0-1f, f2-4f, f6-5f, f7-6f, f1-2f, f6-2f, f4-1f, f5-0f, f1-6f, f1-7f, f0-7f, f7-5f, f3-3f, f3-7f, f4-7f, f6-0f, f4-4f, f6-7f, f2-0f, f7-7f, key1-3, key1-2, f1-3f, f5-6f, f5-7f, f3-5f, f5-3f, f4-0f, f4-3f, f2-6f, f7-3f, f5-1f, f0-6f, f4-2f, f2-5f, f0-3f, f2-1f, f4-6f, f5-4f, f2-2f, f7-2f, f6-3f, f3-2f, f7-1f, f0-4f, f3-0f, f0-5f, f3-4f, key1-1 },
    keywordstyle=[4]\color{blue}\bfseries,
}

\begin{figure*}
\footnotesize
% [inline block 92: 1 envs, 8344 chars -> code_tex | \begin{lstlisting}[basicstyle=\footnotesize\ttfamily] Name: grid-x8-y8-t2-k4-l4-p100 (grid_x-8_y-8_t-2_k-4_l-4.pddl)...]

\end{figure*}

\clearpage

\lstset{
    basicstyle=\footnotesize\ttfamily,
    keywordstyle=\bfseries, % This will apply bold to all keywords
    % Define colors for different groups of keywords
    morekeywords=[1]{Domain},
    keywordstyle=[1]\color{red}\bfseries,
    morekeywords=[2]{Objects, Primitive, Goal, Initial, Plan, plan},
    keywordstyle=[2]\bfseries,
    morekeywords=[3]{putdown, move, pickup, and, loose, unlock, pickup },
    keywordstyle=[3]\color{orange}\bfseries,
    morekeywords=[4]{f0-2f, f0-0f, f2-3f, f3-6f, f7-4f, f3-1f, f6-4f, f2-7f, f5-2f, f1-4f, f5-5f, shape0, key1-0, shape1, f1-1f, f6-1f, f7-0f, f1-5f, f4-5f, f1-0f, f6-6f, f0-1f, f2-4f, f6-5f, f7-6f, f1-2f, f6-2f, f4-1f, f5-0f, f1-6f, f1-7f, f0-7f, f7-5f, f3-3f, f3-7f, f4-7f, f6-0f, f4-4f, f6-7f, f2-0f, f7-7f, key1-3, key1-2, f1-3f, f5-6f, f5-7f, f3-5f, f5-3f, f4-0f, f4-3f, f2-6f, f7-3f, f5-1f, f0-6f, f4-2f, f2-5f, f0-3f, f2-1f, f4-6f, f5-4f, f2-2f, f7-2f, f6-3f, f3-2f, f7-1f, f0-4f, f3-0f, f0-5f, f3-4f, key1-1 },
    keywordstyle=[4]\color{blue}\bfseries,
}

\begin{figure*}
\footnotesize
% [inline block 93: 1 envs, 8344 chars -> code_tex | \begin{lstlisting}[basicstyle=\footnotesize\ttfamily] Name: grid-x8-y8-t2-k4-l4-p100 (grid_x-8_y-8_t-2_k-4_l-4.pddl)...]

\end{figure*}

\clearpage

\lstset{
    basicstyle=\footnotesize\ttfamily,
    keywordstyle=\bfseries, % This will apply bold to all keywords
    % Define colors for different groups of keywords
    morekeywords=[1]{Domain},
    keywordstyle=[1]\color{red}\bfseries,
    morekeywords=[2]{Objects, Primitive, Goal, Initial, Plan, plan},
    keywordstyle=[2]\bfseries,
    morekeywords=[3]{putdown, move, pickup, and, loose, unlock, pickup },
    keywordstyle=[3]\color{orange}\bfseries,
    morekeywords=[4]{f0-2f, f0-0f, f2-3f, f3-6f, f7-4f, f3-1f, f6-4f, f2-7f, f5-2f, f1-4f, f5-5f, shape0, key1-0, shape1, f1-1f, f6-1f, f7-0f, f1-5f, f4-5f, f1-0f, f6-6f, f0-1f, f2-4f, f6-5f, f7-6f, f1-2f, f6-2f, f4-1f, f5-0f, f1-6f, f1-7f, f0-7f, f7-5f, f3-3f, f3-7f, f4-7f, f6-0f, f4-4f, f6-7f, f2-0f, f7-7f, key1-3, key1-2, f1-3f, f5-6f, f5-7f, f3-5f, f5-3f, f4-0f, f4-3f, f2-6f, f7-3f, f5-1f, f0-6f, f4-2f, f2-5f, f0-3f, f2-1f, f4-6f, f5-4f, f2-2f, f7-2f, f6-3f, f3-2f, f7-1f, f0-4f, f3-0f, f0-5f, f3-4f, key1-1 },
    keywordstyle=[4]\color{blue}\bfseries,
}

\begin{figure*}
\footnotesize
% [inline block 94: 1 envs, 8344 chars -> code_tex | \begin{lstlisting}[basicstyle=\footnotesize\ttfamily] Name: grid-x8-y8-t2-k4-l4-p100 (grid_x-8_y-8_t-2_k-4_l-4.pddl)...]

\end{figure*}

\clearpage

\lstset{
    basicstyle=\footnotesize\ttfamily,
    keywordstyle=\bfseries, % This will apply bold to all keywords
    % Define colors for different groups of keywords
    morekeywords=[1]{Domain},
    keywordstyle=[1]\color{red}\bfseries,
    morekeywords=[2]{Objects, Primitive, Goal, Initial, Plan, plan},
    keywordstyle=[2]\bfseries,
    morekeywords=[3]{putdown, move, pickup, and, loose, unlock, pickup },
    keywordstyle=[3]\color{orange}\bfseries,
    morekeywords=[4]{f0-2f, f0-0f, f2-3f, f3-6f, f7-4f, f3-1f, f6-4f, f2-7f, f5-2f, f1-4f, f5-5f, shape0, key1-0, shape1, f1-1f, f6-1f, f7-0f, f1-5f, f4-5f, f1-0f, f6-6f, f0-1f, f2-4f, f6-5f, f7-6f, f1-2f, f6-2f, f4-1f, f5-0f, f1-6f, f1-7f, f0-7f, f7-5f, f3-3f, f3-7f, f4-7f, f6-0f, f4-4f, f6-7f, f2-0f, f7-7f, key1-3, key1-2, f1-3f, f5-6f, f5-7f, f3-5f, f5-3f, f4-0f, f4-3f, f2-6f, f7-3f, f5-1f, f0-6f, f4-2f, f2-5f, f0-3f, f2-1f, f4-6f, f5-4f, f2-2f, f7-2f, f6-3f, f3-2f, f7-1f, f0-4f, f3-0f, f0-5f, f3-4f, key1-1 },
    keywordstyle=[4]\color{blue}\bfseries,
}

\begin{figure*}
\footnotesize
% [inline block 95: 1 envs, 8344 chars -> code_tex | \begin{lstlisting}[basicstyle=\footnotesize\ttfamily] Name: grid-x8-y8-t2-k4-l4-p100 (grid_x-8_y-8_t-2_k-4_l-4.pddl)...]

\end{figure*}

\clearpage

\lstset{
    basicstyle=\footnotesize\ttfamily,
    keywordstyle=\bfseries, % This will apply bold to all keywords
    % Define colors for different groups of keywords
    morekeywords=[1]{Domain},
    keywordstyle=[1]\color{red}\bfseries,
    morekeywords=[2]{Objects, Primitive, Goal, Initial, Plan, plan},
    keywordstyle=[2]\bfseries,
    morekeywords=[3]{putdown, move, pickup, and, loose, unlock, pickup },
    keywordstyle=[3]\color{orange}\bfseries,
    morekeywords=[4]{f0-2f, f0-0f, f2-3f, f3-6f, f7-4f, f3-1f, f6-4f, f2-7f, f5-2f, f1-4f, f5-5f, shape0, shape1, f1-1f, f6-1f, f7-0f, f1-5f, f4-5f, f1-0f, f6-6f, shape2, f0-1f, f2-4f, f6-5f, f7-6f, f1-2f, f6-2f, key2-3, key2-0, f4-1f, f5-0f, f1-6f, key2-2, f1-7f, f0-7f, f7-5f, f3-3f, f3-7f, f4-7f, f6-0f, f4-4f, f6-7f, f2-0f, f7-7f, f1-3f, f5-6f, f5-7f, f3-5f, f5-3f, f4-0f, f4-3f, f2-6f, f7-3f, f5-1f, f0-6f, key2-1, f4-2f, f2-5f, f0-3f, f2-1f, f4-6f, f5-4f, f2-2f, f7-2f, f6-3f, f3-2f, f7-1f, f0-4f, f3-0f, f0-5f, f3-4f },
    keywordstyle=[4]\color{blue}\bfseries,
}

\begin{figure*}
\footnotesize
% [inline block 96: 1 envs, 8503 chars -> code_tex | \begin{lstlisting}[basicstyle=\footnotesize\ttfamily] Name: grid-x8-y8-t3-k4-l4-p100 (grid_x-8_y-8_t-3_k-4_l-4.pddl)...]

\end{figure*}

\clearpage

\lstset{
    basicstyle=\footnotesize\ttfamily,
    keywordstyle=\bfseries, % This will apply bold to all keywords
    % Define colors for different groups of keywords
    morekeywords=[1]{Domain},
    keywordstyle=[1]\color{red}\bfseries,
    morekeywords=[2]{Objects, Primitive, Goal, Initial, Plan, plan},
    keywordstyle=[2]\bfseries,
    morekeywords=[3]{putdown, move, pickup, and, loose, unlock, pickup },
    keywordstyle=[3]\color{orange}\bfseries,
    morekeywords=[4]{f0-2f, f0-0f, f2-3f, f3-6f, f7-4f, f3-1f, f6-4f, f2-7f, f5-2f, f1-4f, f5-5f, shape0, shape1, f1-1f, f6-1f, f7-0f, f1-5f, f4-5f, f1-0f, f6-6f, shape2, f0-1f, f2-4f, f6-5f, f7-6f, f1-2f, f6-2f, key2-3, key2-0, f4-1f, f5-0f, f1-6f, key2-2, f1-7f, f0-7f, f7-5f, f3-3f, f3-7f, f4-7f, f6-0f, f4-4f, f6-7f, f2-0f, f7-7f, f1-3f, f5-6f, f5-7f, f3-5f, f5-3f, f4-0f, f4-3f, f2-6f, f7-3f, f5-1f, f0-6f, key2-1, f4-2f, f2-5f, f0-3f, f2-1f, f4-6f, f5-4f, f2-2f, f7-2f, f6-3f, f3-2f, f7-1f, f0-4f, f3-0f, f0-5f, f3-4f },
    keywordstyle=[4]\color{blue}\bfseries,
}

\begin{figure*}
\footnotesize
% [inline block 97: 1 envs, 8503 chars -> code_tex | \begin{lstlisting}[basicstyle=\footnotesize\ttfamily] Name: grid-x8-y8-t3-k4-l4-p100 (grid_x-8_y-8_t-3_k-4_l-4.pddl)...]

\end{figure*}

\clearpage

\lstset{
    basicstyle=\footnotesize\ttfamily,
    keywordstyle=\bfseries, % This will apply bold to all keywords
    % Define colors for different groups of keywords
    morekeywords=[1]{Domain},
    keywordstyle=[1]\color{red}\bfseries,
    morekeywords=[2]{Objects, Primitive, Goal, Initial, Plan, plan},
    keywordstyle=[2]\bfseries,
    morekeywords=[3]{putdown, move, pickup, and, loose, unlock, pickup },
    keywordstyle=[3]\color{orange}\bfseries,
    morekeywords=[4]{f0-2f, f0-0f, f2-3f, f3-6f, f7-4f, f3-1f, f6-4f, f2-7f, f5-2f, f1-4f, f5-5f, shape0, shape1, f1-1f, f6-1f, f7-0f, f1-5f, f4-5f, f1-0f, f6-6f, shape2, f0-1f, f2-4f, f6-5f, f7-6f, f1-2f, f6-2f, key2-3, key2-0, f4-1f, f5-0f, f1-6f, key2-2, f1-7f, f0-7f, f7-5f, f3-3f, f3-7f, f4-7f, f6-0f, f4-4f, f6-7f, f2-0f, f7-7f, f1-3f, f5-6f, f5-7f, f3-5f, f5-3f, f4-0f, f4-3f, f2-6f, f7-3f, f5-1f, f0-6f, key2-1, f4-2f, f2-5f, f0-3f, f2-1f, f4-6f, f5-4f, f2-2f, f7-2f, f6-3f, f3-2f, f7-1f, f0-4f, f3-0f, f0-5f, f3-4f },
    keywordstyle=[4]\color{blue}\bfseries,
}

\begin{figure*}
\footnotesize
% [inline block 98: 1 envs, 8503 chars -> code_tex | \begin{lstlisting}[basicstyle=\footnotesize\ttfamily] Name: grid-x8-y8-t3-k4-l4-p100 (grid_x-8_y-8_t-3_k-4_l-4.pddl)...]

\end{figure*}

\clearpage

\lstset{
    basicstyle=\footnotesize\ttfamily,
    keywordstyle=\bfseries, % This will apply bold to all keywords
    % Define colors for different groups of keywords
    morekeywords=[1]{Domain},
    keywordstyle=[1]\color{red}\bfseries,
    morekeywords=[2]{Objects, Primitive, Goal, Initial, Plan, plan},
    keywordstyle=[2]\bfseries,
    morekeywords=[3]{putdown, move, pickup, and, loose, unlock, pickup },
    keywordstyle=[3]\color{orange}\bfseries,
    morekeywords=[4]{f0-2f, f0-0f, f2-3f, f3-6f, f7-4f, f3-1f, f6-4f, f2-7f, f5-2f, f1-4f, f5-5f, shape0, shape1, f1-1f, f6-1f, f7-0f, f1-5f, f4-5f, f1-0f, f6-6f, shape2, f0-1f, f2-4f, f6-5f, f7-6f, f1-2f, f6-2f, key2-3, key2-0, f4-1f, f5-0f, f1-6f, key2-2, f1-7f, f0-7f, f7-5f, f3-3f, f3-7f, f4-7f, f6-0f, f4-4f, f6-7f, f2-0f, f7-7f, f1-3f, f5-6f, f5-7f, f3-5f, f5-3f, f4-0f, f4-3f, f2-6f, f7-3f, f5-1f, f0-6f, key2-1, f4-2f, f2-5f, f0-3f, f2-1f, f4-6f, f5-4f, f2-2f, f7-2f, f6-3f, f3-2f, f7-1f, f0-4f, f3-0f, f0-5f, f3-4f },
    keywordstyle=[4]\color{blue}\bfseries,
}

\begin{figure*}
\footnotesize
% [inline block 99: 1 envs, 8503 chars -> code_tex | \begin{lstlisting}[basicstyle=\footnotesize\ttfamily] Name: grid-x8-y8-t3-k4-l4-p100 (grid_x-8_y-8_t-3_k-4_l-4.pddl)...]

\end{figure*}

\clearpage

\lstset{
    basicstyle=\footnotesize\ttfamily,
    keywordstyle=\bfseries, % This will apply bold to all keywords
    % Define colors for different groups of keywords
    morekeywords=[1]{Domain},
    keywordstyle=[1]\color{red}\bfseries,
    morekeywords=[2]{Objects, Primitive, Goal, Initial, Plan, plan},
    keywordstyle=[2]\bfseries,
    morekeywords=[3]{putdown, move, pickup, and, loose, unlock, pickup },
    keywordstyle=[3]\color{orange}\bfseries,
    morekeywords=[4]{f0-2f, f0-0f, f2-3f, f3-6f, f7-4f, f3-1f, f6-4f, f2-7f, f5-2f, f1-4f, f5-5f, shape0, key3-0, shape1, f1-1f, f6-1f, f7-0f, f1-5f, f4-5f, f1-0f, f6-6f, shape2, f0-1f, f2-4f, f6-5f, f7-6f, f1-2f, f6-2f, f4-1f, f5-0f, f1-6f, f1-7f, key3-1, f0-7f, f7-5f, f3-3f, f3-7f, f4-7f, key3-3, f6-0f, f4-4f, f6-7f, f2-0f, f7-7f, f1-3f, f5-6f, f5-7f, f3-5f, f5-3f, f4-0f, f4-3f, f2-6f, f7-3f, f5-1f, f0-6f, f4-2f, f2-5f, key3-2, shape3, f0-3f, f2-1f, f4-6f, f5-4f, f2-2f, f7-2f, f6-3f, f3-2f, f7-1f, f0-4f, f3-0f, f0-5f, f3-4f },
    keywordstyle=[4]\color{blue}\bfseries,
}

\begin{figure*}
\footnotesize
% [inline block 100: 1 envs, 8525 chars -> code_tex | \begin{lstlisting}[basicstyle=\footnotesize\ttfamily] Name: grid-x8-y8-t4-k4-l4-p100 (grid_x-8_y-8_t-4_k-4_l-4.pddl)...]

\end{figure*}

\clearpage

\lstset{
    basicstyle=\footnotesize\ttfamily,
    keywordstyle=\bfseries, % This will apply bold to all keywords
    % Define colors for different groups of keywords
    morekeywords=[1]{Domain},
    keywordstyle=[1]\color{red}\bfseries,
    morekeywords=[2]{Objects, Primitive, Goal, Initial, Plan, plan},
    keywordstyle=[2]\bfseries,
    morekeywords=[3]{putdown, move, pickup, and, loose, unlock, pickup },
    keywordstyle=[3]\color{orange}\bfseries,
    morekeywords=[4]{f0-2f, f0-0f, f2-3f, f3-6f, f7-4f, f3-1f, f6-4f, f2-7f, f5-2f, f1-4f, f5-5f, shape0, key3-0, shape1, f1-1f, f6-1f, f7-0f, f1-5f, f4-5f, f1-0f, f6-6f, shape2, f0-1f, f2-4f, f6-5f, f7-6f, f1-2f, f6-2f, f4-1f, f5-0f, f1-6f, f1-7f, key3-1, f0-7f, f7-5f, f3-3f, f3-7f, f4-7f, key3-3, f6-0f, f4-4f, f6-7f, f2-0f, f7-7f, f1-3f, f5-6f, f5-7f, f3-5f, f5-3f, f4-0f, f4-3f, f2-6f, f7-3f, f5-1f, f0-6f, f4-2f, f2-5f, key3-2, shape3, f0-3f, f2-1f, f4-6f, f5-4f, f2-2f, f7-2f, f6-3f, f3-2f, f7-1f, f0-4f, f3-0f, f0-5f, f3-4f },
    keywordstyle=[4]\color{blue}\bfseries,
}

\begin{figure*}
\footnotesize
% [inline block 101: 1 envs, 8525 chars -> code_tex | \begin{lstlisting}[basicstyle=\footnotesize\ttfamily] Name: grid-x8-y8-t4-k4-l4-p100 (grid_x-8_y-8_t-4_k-4_l-4.pddl)...]

\end{figure*}

\clearpage

\lstset{
    basicstyle=\footnotesize\ttfamily,
    keywordstyle=\bfseries, % This will apply bold to all keywords
    % Define colors for different groups of keywords
    morekeywords=[1]{Domain},
    keywordstyle=[1]\color{red}\bfseries,
    morekeywords=[2]{Objects, Primitive, Goal, Initial, Plan, plan},
    keywordstyle=[2]\bfseries,
    morekeywords=[3]{putdown, move, pickup, and, loose, unlock, pickup },
    keywordstyle=[3]\color{orange}\bfseries,
    morekeywords=[4]{f0-2f, f0-0f, f2-3f, f3-6f, f7-4f, f3-1f, f6-4f, f2-7f, f5-2f, f1-4f, f5-5f, shape0, key3-0, shape1, f1-1f, f6-1f, f7-0f, f1-5f, f4-5f, f1-0f, f6-6f, shape2, f0-1f, f2-4f, f6-5f, f7-6f, f1-2f, f6-2f, f4-1f, f5-0f, f1-6f, f1-7f, key3-1, f0-7f, f7-5f, f3-3f, f3-7f, f4-7f, key3-3, f6-0f, f4-4f, f6-7f, f2-0f, f7-7f, f1-3f, f5-6f, f5-7f, f3-5f, f5-3f, f4-0f, f4-3f, f2-6f, f7-3f, f5-1f, f0-6f, f4-2f, f2-5f, key3-2, shape3, f0-3f, f2-1f, f4-6f, f5-4f, f2-2f, f7-2f, f6-3f, f3-2f, f7-1f, f0-4f, f3-0f, f0-5f, f3-4f },
    keywordstyle=[4]\color{blue}\bfseries,
}

\begin{figure*}
\footnotesize
% [inline block 102: 1 envs, 8525 chars -> code_tex | \begin{lstlisting}[basicstyle=\footnotesize\ttfamily] Name: grid-x8-y8-t4-k4-l4-p100 (grid_x-8_y-8_t-4_k-4_l-4.pddl)...]

\end{figure*}

\clearpage

\lstset{
    basicstyle=\footnotesize\ttfamily,
    keywordstyle=\bfseries, % This will apply bold to all keywords
    % Define colors for different groups of keywords
    morekeywords=[1]{Domain},
    keywordstyle=[1]\color{red}\bfseries,
    morekeywords=[2]{Objects, Primitive, Goal, Initial, Plan, plan},
    keywordstyle=[2]\bfseries,
    morekeywords=[3]{putdown, move, pickup, and, loose, unlock, pickup },
    keywordstyle=[3]\color{orange}\bfseries,
    morekeywords=[4]{f0-2f, f0-0f, f2-3f, f3-6f, f7-4f, f3-1f, f6-4f, f2-7f, f5-2f, f1-4f, f5-5f, shape0, key3-0, shape1, f1-1f, f6-1f, f7-0f, f1-5f, f4-5f, f1-0f, f6-6f, shape2, f0-1f, f2-4f, f6-5f, f7-6f, f1-2f, f6-2f, f4-1f, f5-0f, f1-6f, f1-7f, key3-1, f0-7f, f7-5f, f3-3f, f3-7f, f4-7f, key3-3, f6-0f, f4-4f, f6-7f, f2-0f, f7-7f, f1-3f, f5-6f, f5-7f, f3-5f, f5-3f, f4-0f, f4-3f, f2-6f, f7-3f, f5-1f, f0-6f, f4-2f, f2-5f, key3-2, shape3, f0-3f, f2-1f, f4-6f, f5-4f, f2-2f, f7-2f, f6-3f, f3-2f, f7-1f, f0-4f, f3-0f, f0-5f, f3-4f },
    keywordstyle=[4]\color{blue}\bfseries,
}

\begin{figure*}
\footnotesize
% [inline block 103: 1 envs, 8525 chars -> code_tex | \begin{lstlisting}[basicstyle=\footnotesize\ttfamily] Name: grid-x8-y8-t4-k4-l4-p100 (grid_x-8_y-8_t-4_k-4_l-4.pddl)...]

\end{figure*}

\clearpage

\lstset{
    basicstyle=\footnotesize\ttfamily,
    keywordstyle=\bfseries, % This will apply bold to all keywords
    % Define colors for different groups of keywords
    morekeywords=[1]{Domain},
    keywordstyle=[1]\color{red}\bfseries,
    morekeywords=[2]{Objects, Primitive, Goal, Initial, Plan, plan},
    keywordstyle=[2]\bfseries,
    morekeywords=[3]{putdown, move, pickup, and, loose, unlock, pickup },
    keywordstyle=[3]\color{orange}\bfseries,
    morekeywords=[4]{f0-2f, f0-0f, f2-3f, f3-6f, f7-4f, f3-1f, f6-4f, f2-7f, f5-2f, f8-1f, f1-4f, f5-5f, shape0, f8-4f, f1-1f, f6-1f, f7-0f, f1-5f, f4-5f, f8-6f, f1-0f, f8-2f, f6-6f, f0-1f, f2-4f, f6-5f, f7-6f, f1-2f, f6-2f, f4-1f, f5-0f, f1-6f, f8-7f, f1-7f, key0-1, f8-5f, key0-2, f0-7f, f7-5f, f3-3f, f3-7f, f4-7f, f6-0f, f8-0f, f4-4f, f6-7f, f2-0f, f7-7f, f1-3f, f5-6f, f5-7f, f3-5f, f5-3f, f4-0f, f4-3f, f2-6f, key0-0, f7-3f, f5-1f, f0-6f, f4-2f, f2-5f, f0-3f, f2-1f, f8-3f, f5-4f, f4-6f, f2-2f, f7-2f, f6-3f, f3-2f, f7-1f, f0-4f, f3-0f, f0-5f, f3-4f },
    keywordstyle=[4]\color{blue}\bfseries,
}

\begin{figure*}
\footnotesize
% [inline block 104: 1 envs, 8764 chars -> code_tex | \begin{lstlisting}[basicstyle=\footnotesize\ttfamily] Name: grid-x9-y8-t1-k3-l4-p100 (grid_x-9_y-8_t-1_k-3_l-4.pddl)...]

\end{figure*}

\clearpage

\lstset{
    basicstyle=\footnotesize\ttfamily,
    keywordstyle=\bfseries, % This will apply bold to all keywords
    % Define colors for different groups of keywords
    morekeywords=[1]{Domain},
    keywordstyle=[1]\color{red}\bfseries,
    morekeywords=[2]{Objects, Primitive, Goal, Initial, Plan, plan},
    keywordstyle=[2]\bfseries,
    morekeywords=[3]{putdown, move, pickup, and, loose, unlock, pickup },
    keywordstyle=[3]\color{orange}\bfseries,
    morekeywords=[4]{f0-2f, f0-0f, f2-3f, f3-6f, f7-4f, f3-1f, f6-4f, f2-7f, f5-2f, f8-1f, f1-4f, f5-5f, shape0, f8-4f, f1-1f, f6-1f, f7-0f, f1-5f, f4-5f, f8-6f, f1-0f, f8-2f, f6-6f, f0-1f, f2-4f, f6-5f, f7-6f, f1-2f, f6-2f, f4-1f, f5-0f, f1-6f, f8-7f, f1-7f, key0-1, f8-5f, key0-2, f0-7f, f7-5f, f3-3f, f3-7f, f4-7f, f6-0f, f8-0f, f4-4f, f6-7f, f2-0f, f7-7f, f1-3f, f5-6f, f5-7f, f3-5f, f5-3f, f4-0f, f4-3f, f2-6f, key0-0, f7-3f, f5-1f, f0-6f, f4-2f, f2-5f, f0-3f, f2-1f, f8-3f, f5-4f, f4-6f, f2-2f, f7-2f, f6-3f, f3-2f, f7-1f, f0-4f, f3-0f, f0-5f, f3-4f },
    keywordstyle=[4]\color{blue}\bfseries,
}

\begin{figure*}
\footnotesize
% [inline block 105: 1 envs, 8764 chars -> code_tex | \begin{lstlisting}[basicstyle=\footnotesize\ttfamily] Name: grid-x9-y8-t1-k3-l4-p100 (grid_x-9_y-8_t-1_k-3_l-4.pddl)...]

\end{figure*}

\clearpage

\lstset{
    basicstyle=\footnotesize\ttfamily,
    keywordstyle=\bfseries, % This will apply bold to all keywords
    % Define colors for different groups of keywords
    morekeywords=[1]{Domain},
    keywordstyle=[1]\color{red}\bfseries,
    morekeywords=[2]{Objects, Primitive, Goal, Initial, Plan, plan},
    keywordstyle=[2]\bfseries,
    morekeywords=[3]{putdown, move, pickup, and, loose, unlock, pickup },
    keywordstyle=[3]\color{orange}\bfseries,
    morekeywords=[4]{f0-2f, f0-0f, f2-3f, f3-6f, f7-4f, f3-1f, f6-4f, f2-7f, f5-2f, f8-1f, f1-4f, f5-5f, shape0, f8-4f, f1-1f, f6-1f, f7-0f, f1-5f, f4-5f, f8-6f, f1-0f, f8-2f, f6-6f, f0-1f, f2-4f, f6-5f, f7-6f, f1-2f, f6-2f, f4-1f, f5-0f, f1-6f, f8-7f, f1-7f, key0-1, f8-5f, key0-2, f0-7f, f7-5f, f3-3f, f3-7f, f4-7f, f6-0f, f8-0f, f4-4f, f6-7f, f2-0f, f7-7f, f1-3f, f5-6f, f5-7f, f3-5f, f5-3f, f4-0f, f4-3f, f2-6f, key0-0, f7-3f, f5-1f, f0-6f, f4-2f, f2-5f, f0-3f, f2-1f, f8-3f, f5-4f, f4-6f, f2-2f, f7-2f, f6-3f, f3-2f, f7-1f, f0-4f, f3-0f, f0-5f, f3-4f },
    keywordstyle=[4]\color{blue}\bfseries,
}

\begin{figure*}
\footnotesize
% [inline block 106: 1 envs, 8764 chars -> code_tex | \begin{lstlisting}[basicstyle=\footnotesize\ttfamily] Name: grid-x9-y8-t1-k3-l4-p100 (grid_x-9_y-8_t-1_k-3_l-4.pddl)...]

\end{figure*}

\clearpage

\lstset{
    basicstyle=\footnotesize\ttfamily,
    keywordstyle=\bfseries, % This will apply bold to all keywords
    % Define colors for different groups of keywords
    morekeywords=[1]{Domain},
    keywordstyle=[1]\color{red}\bfseries,
    morekeywords=[2]{Objects, Primitive, Goal, Initial, Plan, plan},
    keywordstyle=[2]\bfseries,
    morekeywords=[3]{putdown, move, pickup, and, loose, unlock, pickup },
    keywordstyle=[3]\color{orange}\bfseries,
    morekeywords=[4]{f0-2f, f0-0f, f2-3f, f3-6f, f7-4f, f3-1f, f6-4f, f2-7f, f5-2f, f8-1f, f1-4f, f5-5f, shape0, f8-4f, f1-1f, f6-1f, f7-0f, f1-5f, f4-5f, f8-6f, f1-0f, f8-2f, f6-6f, f0-1f, f2-4f, f6-5f, f7-6f, f1-2f, f6-2f, f4-1f, f5-0f, f1-6f, f8-7f, f1-7f, key0-1, f8-5f, key0-2, f0-7f, f7-5f, f3-3f, f3-7f, f4-7f, f6-0f, f8-0f, f4-4f, f6-7f, f2-0f, f7-7f, f1-3f, f5-6f, f5-7f, f3-5f, f5-3f, f4-0f, f4-3f, f2-6f, key0-0, f7-3f, f5-1f, f0-6f, f4-2f, f2-5f, f0-3f, f2-1f, f8-3f, f5-4f, f4-6f, f2-2f, f7-2f, f6-3f, f3-2f, f7-1f, f0-4f, f3-0f, f0-5f, f3-4f },
    keywordstyle=[4]\color{blue}\bfseries,
}

\begin{figure*}
\footnotesize
% [inline block 107: 1 envs, 8764 chars -> code_tex | \begin{lstlisting}[basicstyle=\footnotesize\ttfamily] Name: grid-x9-y8-t1-k3-l4-p100 (grid_x-9_y-8_t-1_k-3_l-4.pddl)...]

\end{figure*}

\clearpage

\lstset{
    basicstyle=\footnotesize\ttfamily,
    keywordstyle=\bfseries, % This will apply bold to all keywords
    % Define colors for different groups of keywords
    morekeywords=[1]{Domain},
    keywordstyle=[1]\color{red}\bfseries,
    morekeywords=[2]{Objects, Primitive, Goal, Initial, Plan, plan},
    keywordstyle=[2]\bfseries,
    morekeywords=[3]{putdown, move, pickup, and, loose, unlock, pickup },
    keywordstyle=[3]\color{orange}\bfseries,
    morekeywords=[4]{f0-2f, f0-0f, f2-3f, f3-6f, f7-4f, f3-1f, f6-4f, f2-7f, f5-2f, f8-1f, f1-4f, f5-5f, shape0, f8-4f, f1-1f, f6-1f, f7-0f, f1-5f, f4-5f, f8-6f, f1-0f, f8-2f, f6-6f, f0-1f, f2-4f, f6-5f, f7-6f, f1-2f, f6-2f, f4-1f, f5-0f, f1-6f, f8-7f, f1-7f, key0-1, f8-5f, key0-2, f0-7f, f7-5f, f3-3f, f3-7f, f4-7f, f6-0f, f8-0f, f4-4f, f6-7f, f2-0f, f7-7f, f1-3f, f5-6f, f5-7f, f3-5f, f5-3f, f4-0f, f4-3f, f2-6f, key0-0, f7-3f, f5-1f, f0-6f, f4-2f, f2-5f, f0-3f, f2-1f, f8-3f, f5-4f, f4-6f, f2-2f, f7-2f, f6-3f, f3-2f, f7-1f, f0-4f, f3-0f, f0-5f, f3-4f },
    keywordstyle=[4]\color{blue}\bfseries,
}

\lstset{
    basicstyle=\footnotesize\ttfamily,
    keywordstyle=\bfseries, % This will apply bold to all keywords
    % Define colors for different groups of keywords
    morekeywords=[1]{Domain},
    keywordstyle=[1]\color{red}\bfseries,
    morekeywords=[2]{Objects, Primitive, Goal, Initial, Plan, plan},
    keywordstyle=[2]\bfseries,
    morekeywords=[3]{putdown, move, pickup, and, loose, unlock, pickup },
    keywordstyle=[3]\color{orange}\bfseries,
    morekeywords=[4]{f0-2f, f0-0f, f2-3f, f3-6f, f7-4f, f3-1f, f6-4f, f2-7f, f5-2f, f8-1f, f1-4f, f5-5f, shape0, f8-4f, f1-1f, f6-1f, f7-0f, f1-5f, f4-5f, f8-6f, f1-0f, f8-2f, f6-6f, f0-1f, f2-4f, f6-5f, f7-6f, f1-2f, f6-2f, f4-1f, f5-0f, f1-6f, f8-7f, f1-7f, key0-1, f8-5f, key0-2, f0-7f, f7-5f, f3-3f, f3-7f, f4-7f, f6-0f, f8-0f, f4-4f, f6-7f, f2-0f, f7-7f, f1-3f, f5-6f, f5-7f, f3-5f, f5-3f, f4-0f, f4-3f, f2-6f, key0-0, f7-3f, f5-1f, f0-6f, f4-2f, f2-5f, f0-3f, f2-1f, f8-3f, f5-4f, f4-6f, f2-2f, f7-2f, f6-3f, f3-2f, f7-1f, f0-4f, f3-0f, f0-5f, f3-4f },
    keywordstyle=[4]\color{blue}\bfseries,
}

\lstset{
    basicstyle=\footnotesize\ttfamily,
    keywordstyle=\bfseries, % This will apply bold to all keywords
    % Define colors for different groups of keywords
    morekeywords=[1]{Domain},
    keywordstyle=[1]\color{red}\bfseries,
    morekeywords=[2]{Objects, Primitive, Goal, Initial, Plan, plan},
    keywordstyle=[2]\bfseries,
    morekeywords=[3]{putdown, move, pickup, and, loose, unlock, pickup },
    keywordstyle=[3]\color{orange}\bfseries,
    morekeywords=[4]{f0-2f, f0-0f, f2-3f, f3-6f, f7-4f, f3-1f, f6-4f, f2-7f, f5-2f, f8-1f, f1-4f, f5-5f, shape0, f8-4f, f1-1f, f6-1f, f7-0f, f1-5f, f4-5f, f8-6f, f1-0f, f8-2f, f6-6f, f0-1f, f2-4f, f6-5f, f7-6f, f1-2f, f6-2f, f4-1f, f5-0f, f1-6f, f8-7f, f1-7f, key0-1, f8-5f, key0-2, f0-7f, f7-5f, f3-3f, f3-7f, f4-7f, f6-0f, f8-0f, f4-4f, f6-7f, f2-0f, f7-7f, f1-3f, f5-6f, f5-7f, f3-5f, f5-3f, f4-0f, f4-3f, f2-6f, key0-0, f7-3f, f5-1f, f0-6f, f4-2f, f2-5f, f0-3f, f2-1f, f8-3f, f5-4f, f4-6f, f2-2f, f7-2f, f6-3f, f3-2f, f7-1f, f0-4f, f3-0f, f0-5f, f3-4f },
    keywordstyle=[4]\color{blue}\bfseries,
}

\lstset{
    basicstyle=\footnotesize\ttfamily,
    keywordstyle=\bfseries, % This will apply bold to all keywords
    % Define colors for different groups of keywords
    morekeywords=[1]{Domain},
    keywordstyle=[1]\color{red}\bfseries,
    morekeywords=[2]{Objects, Primitive, Goal, Initial, Plan, plan},
    keywordstyle=[2]\bfseries,
    morekeywords=[3]{putdown, move, pickup, and, loose, unlock, pickup },
    keywordstyle=[3]\color{orange}\bfseries,
    morekeywords=[4]{f0-2f, f0-0f, f2-3f, f3-6f, f7-4f, f3-1f, f6-4f, f2-7f, f5-2f, f8-1f, f1-4f, f5-5f, shape0, f8-4f, f1-1f, f6-1f, f7-0f, f1-5f, f4-5f, f8-6f, f1-0f, f8-2f, f6-6f, f0-1f, f2-4f, f6-5f, f7-6f, f1-2f, f6-2f, f4-1f, f5-0f, f1-6f, f8-7f, f1-7f, key0-1, f8-5f, key0-2, f0-7f, f7-5f, f3-3f, f3-7f, f4-7f, f6-0f, f8-0f, f4-4f, f6-7f, f2-0f, f7-7f, f1-3f, f5-6f, f5-7f, f3-5f, f5-3f, f4-0f, f4-3f, f2-6f, key0-0, f7-3f, f5-1f, f0-6f, f4-2f, f2-5f, f0-3f, f2-1f, f8-3f, f5-4f, f4-6f, f2-2f, f7-2f, f6-3f, f3-2f, f7-1f, f0-4f, f3-0f, f0-5f, f3-4f },
    keywordstyle=[4]\color{blue}\bfseries,
}

\lstset{
    basicstyle=\footnotesize\ttfamily,
    keywordstyle=\bfseries, % This will apply bold to all keywords
    % Define colors for different groups of keywords
    morekeywords=[1]{Domain},
    keywordstyle=[1]\color{red}\bfseries,
    morekeywords=[2]{Objects, Primitive, Goal, Initial, Plan, plan},
    keywordstyle=[2]\bfseries,
    morekeywords=[3]{putdown, move, pickup, and, loose, unlock, pickup },
    keywordstyle=[3]\color{orange}\bfseries,
    morekeywords=[4]{f2-3f, f0-0f, key2-2, f2-7f, f7-4f, shape1, f6-1f, f8-6f, f2-4f, f6-5f, f6-2f, f0-7f, f7-7f, f4-0f, f7-3f, key2-1, f2-1f, f8-3f, f5-4f, f3-2f, f0-4f, f0-5f, f3-1f, shape0, f5-2f, f8-1f, f1-4f, f8-4f, f1-5f, f7-0f, f1-0f, f6-6f, f0-1f, f1-2f, key2-0, f8-5f, f7-5f, f3-3f, f4-7f, f3-5f, f4-3f, f2-6f, f0-6f, f4-2f, f6-7f, f8-7f, f6-4f, f1-1f, f8-2f, shape2, f4-1f, f1-7f, f3-7f, f6-0f, f8-0f, f4-4f, f2-0f, f1-3f, f5-7f, f5-3f, f5-1f, f4-6f, f2-2f, f7-2f, f6-3f, f7-1f, f3-0f, f3-4f, f0-2f, f5-5f, f4-5f, f7-6f, f1-6f, f5-0f, f5-6f, f0-3f, f3-6f, f2-5f },
    keywordstyle=[4]\color{blue}\bfseries,
}

\lstset{
    basicstyle=\footnotesize\ttfamily,
    keywordstyle=\bfseries, % This will apply bold to all keywords
    % Define colors for different groups of keywords
    morekeywords=[1]{Domain},
    keywordstyle=[1]\color{red}\bfseries,
    morekeywords=[2]{Objects, Primitive, Goal, Initial, Plan, plan},
    keywordstyle=[2]\bfseries,
    morekeywords=[3]{putdown, move, pickup, and, loose, unlock, pickup },
    keywordstyle=[3]\color{orange}\bfseries,
    morekeywords=[4]{f2-3f, f0-0f, key2-2, f2-7f, f7-4f, shape1, f6-1f, f8-6f, f2-4f, f6-5f, f6-2f, f0-7f, f7-7f, f4-0f, f7-3f, key2-1, f2-1f, f8-3f, f5-4f, f3-2f, f0-4f, f0-5f, f3-1f, shape0, f5-2f, f8-1f, f1-4f, f8-4f, f1-5f, f7-0f, f1-0f, f6-6f, f0-1f, f1-2f, key2-0, f8-5f, f7-5f, f3-3f, f4-7f, f3-5f, f4-3f, f2-6f, f0-6f, f4-2f, f6-7f, f8-7f, f6-4f, f1-1f, f8-2f, shape2, f4-1f, f1-7f, f3-7f, f6-0f, f8-0f, f4-4f, f2-0f, f1-3f, f5-7f, f5-3f, f5-1f, f4-6f, f2-2f, f7-2f, f6-3f, f7-1f, f3-0f, f3-4f, f0-2f, f5-5f, f4-5f, f7-6f, f1-6f, f5-0f, f5-6f, f0-3f, f3-6f, f2-5f },
    keywordstyle=[4]\color{blue}\bfseries,
}

\lstset{
    basicstyle=\footnotesize\ttfamily,
    keywordstyle=\bfseries, % This will apply bold to all keywords
    % Define colors for different groups of keywords
    morekeywords=[1]{Domain},
    keywordstyle=[1]\color{red}\bfseries,
    morekeywords=[2]{Objects, Primitive, Goal, Initial, Plan, plan},
    keywordstyle=[2]\bfseries,
    morekeywords=[3]{putdown, move, pickup, and, loose, unlock, pickup },
    keywordstyle=[3]\color{orange}\bfseries,
    morekeywords=[4]{f2-3f, f0-0f, f2-7f, f7-4f, f6-1f, f8-6f, f2-4f, f6-5f, f6-2f, f0-7f, f7-7f, f4-0f, f7-3f, f2-1f, f8-3f, f5-4f, f3-2f, f0-4f, f0-5f, f3-1f, shape0, f5-2f, f8-1f, f1-4f, f8-4f, f0-8f, f1-5f, f7-0f, f1-0f, f6-6f, f0-1f, f1-2f, f8-5f, f5-8f, f7-5f, f3-3f, f4-7f, f3-5f, f4-3f, f2-6f, f0-6f, f4-2f, f6-7f, f8-7f, f6-4f, f2-8f, f1-1f, f7-8f, f8-2f, f4-1f, f1-7f, f3-7f, f6-0f, f8-0f, f4-4f, f2-0f, f1-3f, f6-8f, f5-7f, f5-3f, f5-1f, f1-8f, f4-6f, f2-2f, f7-2f, f6-3f, f7-1f, f3-0f, f3-4f, f0-2f, f5-5f, f4-5f, f7-6f, f1-6f, f5-0f, key0-1, f4-8f, f3-8f, f5-6f, key0-0, f8-8f, f0-3f, f3-6f, f2-5f },
    keywordstyle=[4]\color{blue}\bfseries,
}

\begin{figure*}
\footnotesize
% [inline block 108: 1 envs, 9577 chars -> code_tex | \begin{lstlisting}[basicstyle=\footnotesize\ttfamily] Name: grid-x9-y9-t1-k2-l3-p100 (grid_x-9_y-9_t-1_k-2_l-3.pddl)...]

\end{figure*}

\clearpage

\lstset{
    basicstyle=\footnotesize\ttfamily,
    keywordstyle=\bfseries, % This will apply bold to all keywords
    % Define colors for different groups of keywords
    morekeywords=[1]{Domain},
    keywordstyle=[1]\color{red}\bfseries,
    morekeywords=[2]{Objects, Primitive, Goal, Initial, Plan, plan},
    keywordstyle=[2]\bfseries,
    morekeywords=[3]{putdown, move, pickup, and, loose, unlock, pickup },
    keywordstyle=[3]\color{orange}\bfseries,
    morekeywords=[4]{f2-3f, f0-0f, f2-7f, f7-4f, f6-1f, f8-6f, f2-4f, f6-5f, f6-2f, f0-7f, f7-7f, f4-0f, f7-3f, f2-1f, f8-3f, f5-4f, f3-2f, f0-4f, f0-5f, f3-1f, shape0, f5-2f, f8-1f, f1-4f, f8-4f, f0-8f, f1-5f, f7-0f, f1-0f, f6-6f, f0-1f, f1-2f, f8-5f, f5-8f, f7-5f, f3-3f, f4-7f, f3-5f, f4-3f, f2-6f, f0-6f, f4-2f, f6-7f, f8-7f, f6-4f, f2-8f, f1-1f, f7-8f, f8-2f, f4-1f, f1-7f, f3-7f, f6-0f, f8-0f, f4-4f, f2-0f, f1-3f, f6-8f, f5-7f, f5-3f, f5-1f, f1-8f, f4-6f, f2-2f, f7-2f, f6-3f, f7-1f, f3-0f, f3-4f, f0-2f, f5-5f, f4-5f, f7-6f, f1-6f, f5-0f, key0-1, f4-8f, f3-8f, f5-6f, key0-0, f8-8f, f0-3f, f3-6f, f2-5f },
    keywordstyle=[4]\color{blue}\bfseries,
}

\begin{figure*}
\footnotesize
% [inline block 109: 1 envs, 9577 chars -> code_tex | \begin{lstlisting}[basicstyle=\footnotesize\ttfamily] Name: grid-x9-y9-t1-k2-l3-p100 (grid_x-9_y-9_t-1_k-2_l-3.pddl)...]

\end{figure*}

\clearpage

\lstset{
    basicstyle=\footnotesize\ttfamily,
    keywordstyle=\bfseries, % This will apply bold to all keywords
    % Define colors for different groups of keywords
    morekeywords=[1]{Domain},
    keywordstyle=[1]\color{red}\bfseries,
    morekeywords=[2]{Objects, Primitive, Goal, Initial, Plan, plan},
    keywordstyle=[2]\bfseries,
    morekeywords=[3]{putdown, move, pickup, and, loose, unlock, pickup },
    keywordstyle=[3]\color{orange}\bfseries,
    morekeywords=[4]{f2-3f, f0-0f, f2-7f, f7-4f, f6-1f, f8-6f, f2-4f, f6-5f, f6-2f, f0-7f, f7-7f, f4-0f, f7-3f, f2-1f, f8-3f, f5-4f, f3-2f, f0-4f, f0-5f, f3-1f, shape0, f5-2f, f8-1f, f1-4f, f8-4f, f0-8f, f1-5f, f7-0f, f1-0f, f6-6f, f0-1f, f1-2f, f8-5f, f5-8f, f7-5f, f3-3f, f4-7f, f3-5f, f4-3f, f2-6f, f0-6f, f4-2f, f6-7f, f8-7f, f6-4f, f2-8f, f1-1f, f7-8f, f8-2f, f4-1f, f1-7f, f3-7f, f6-0f, f8-0f, f4-4f, f2-0f, f1-3f, f6-8f, f5-7f, f5-3f, f5-1f, f1-8f, f4-6f, f2-2f, f7-2f, f6-3f, f7-1f, f3-0f, f3-4f, f0-2f, f5-5f, f4-5f, f7-6f, f1-6f, f5-0f, key0-1, f4-8f, f3-8f, f5-6f, key0-0, f8-8f, f0-3f, f3-6f, f2-5f },
    keywordstyle=[4]\color{blue}\bfseries,
}

\begin{figure*}
\footnotesize
% [inline block 110: 1 envs, 9395 chars -> code_tex | \begin{lstlisting}[basicstyle=\footnotesize\ttfamily] Name: grid-x9-y9-t1-k2-l3-p100 (grid_x-9_y-9_t-1_k-2_l-3.pddl)...]

\end{figure*}

\clearpage

\lstset{
    basicstyle=\footnotesize\ttfamily,
    keywordstyle=\bfseries, % This will apply bold to all keywords
    % Define colors for different groups of keywords
    morekeywords=[1]{Domain},
    keywordstyle=[1]\color{red}\bfseries,
    morekeywords=[2]{Objects, Primitive, Goal, Initial, Plan, plan},
    keywordstyle=[2]\bfseries,
    morekeywords=[3]{putdown, move, pickup, and, loose, unlock, pickup },
    keywordstyle=[3]\color{orange}\bfseries,
    morekeywords=[4]{f2-3f, f0-0f, f2-7f, f7-4f, f6-1f, f8-6f, f2-4f, f6-5f, f6-2f, f0-7f, f7-7f, f4-0f, f7-3f, f2-1f, f8-3f, f5-4f, f3-2f, f0-4f, f0-5f, f3-1f, shape0, f5-2f, f8-1f, f1-4f, f8-4f, f0-8f, f1-5f, f7-0f, f1-0f, f6-6f, f0-1f, f1-2f, f8-5f, f5-8f, f7-5f, f3-3f, f4-7f, f3-5f, f4-3f, f2-6f, f0-6f, f4-2f, f6-7f, f8-7f, f6-4f, f2-8f, f1-1f, f7-8f, f8-2f, f4-1f, f1-7f, f3-7f, f6-0f, f8-0f, f4-4f, f2-0f, f1-3f, f6-8f, f5-7f, f5-3f, f5-1f, f1-8f, f4-6f, f2-2f, f7-2f, f6-3f, f7-1f, f3-0f, f3-4f, f0-2f, f5-5f, f4-5f, f7-6f, f1-6f, f5-0f, key0-1, f4-8f, f3-8f, f5-6f, key0-0, f8-8f, f0-3f, f3-6f, f2-5f },
    keywordstyle=[4]\color{blue}\bfseries,
}

\begin{figure*}
\footnotesize
% [inline block 111: 1 envs, 9577 chars -> code_tex | \begin{lstlisting}[basicstyle=\footnotesize\ttfamily] Name: grid-x9-y9-t1-k2-l3-p100 (grid_x-9_y-9_t-1_k-2_l-3.pddl)...]

\end{figure*}

\clearpage

\lstset{
    basicstyle=\footnotesize\ttfamily,
    keywordstyle=\bfseries, % This will apply bold to all keywords
    % Define colors for different groups of keywords
    morekeywords=[1]{Domain},
    keywordstyle=[1]\color{red}\bfseries,
    morekeywords=[2]{Objects, Primitive, Goal, Initial, Plan, plan},
    keywordstyle=[2]\bfseries,
    morekeywords=[3]{putdown, move, pickup, and, loose, unlock, pickup },
    keywordstyle=[3]\color{orange}\bfseries,
    morekeywords=[4]{f2-3f, f0-0f, f2-7f, f7-4f, shape1, f6-1f, f8-6f, f2-4f, f6-5f, f6-2f, f0-7f, f7-7f, f4-0f, f7-3f, shape3, f2-1f, f8-3f, f5-4f, f3-2f, f0-4f, f0-5f, f3-1f, shape0, f5-2f, f8-1f, f1-4f, f8-4f, f0-8f, f1-5f, f7-0f, f1-0f, f6-6f, f0-1f, f1-2f, f8-5f, f5-8f, f7-5f, f3-3f, f4-7f, key3-3, f3-5f, f4-3f, f2-6f, f0-6f, f4-2f, f6-7f, f8-7f, f6-4f, f2-8f, f1-1f, f7-8f, f8-2f, shape2, f4-1f, f1-7f, f3-7f, f6-0f, f8-0f, f4-4f, f2-0f, f1-3f, f6-8f, f5-7f, f5-3f, f5-1f, f1-8f, f4-6f, f2-2f, f7-2f, f6-3f, f7-1f, f3-0f, f3-4f, f0-2f, f5-5f, key3-0, f4-5f, f7-6f, f1-6f, f5-0f, key3-1, f4-8f, f3-8f, f5-6f, f8-8f, f0-3f, f3-6f, f2-5f, key3-2 },
    keywordstyle=[4]\color{blue}\bfseries,
}

\lstset{
    basicstyle=\footnotesize\ttfamily,
    keywordstyle=\bfseries, % This will apply bold to all keywords
    % Define colors for different groups of keywords
    morekeywords=[1]{Domain},
    keywordstyle=[1]\color{red}\bfseries,
    morekeywords=[2]{Objects, Primitive, Goal, Initial, Plan, plan},
    keywordstyle=[2]\bfseries,
    morekeywords=[3]{putdown, move, pickup, and, loose, unlock, pickup },
    keywordstyle=[3]\color{orange}\bfseries,
    morekeywords=[4]{f2-3f, f0-0f, f2-7f, f7-4f, shape1, f6-1f, f8-6f, f2-4f, f6-5f, f6-2f, f0-7f, f7-7f, f4-0f, f7-3f, shape3, f2-1f, f8-3f, f5-4f, f3-2f, f0-4f, f0-5f, f3-1f, shape0, f5-2f, f8-1f, f1-4f, f8-4f, f0-8f, f1-5f, f7-0f, f1-0f, f6-6f, f0-1f, f1-2f, f8-5f, f5-8f, f7-5f, f3-3f, f4-7f, key3-3, f3-5f, f4-3f, f2-6f, f0-6f, f4-2f, f6-7f, f8-7f, f6-4f, f2-8f, f1-1f, f7-8f, f8-2f, shape2, f4-1f, f1-7f, f3-7f, f6-0f, f8-0f, f4-4f, f2-0f, f1-3f, f6-8f, f5-7f, f5-3f, f5-1f, f1-8f, f4-6f, f2-2f, f7-2f, f6-3f, f7-1f, f3-0f, f3-4f, f0-2f, f5-5f, key3-0, f4-5f, f7-6f, f1-6f, f5-0f, key3-1, f4-8f, f3-8f, f5-6f, f8-8f, f0-3f, f3-6f, f2-5f, key3-2 },
    keywordstyle=[4]\color{blue}\bfseries,
}
