# Supplementary material for: Sketch Decompositions for Classical Planning via Deep Reinforcement Learning
Source: arXiv:2412.08574 source file (2025-08-15)
Supplement: Supplementary file 2 [file logistics.tex]

\lstset{
    basicstyle=\footnotesize\ttfamily,
    keywordstyle=\bfseries, % This will apply bold to all keywords
    % Define colors for different groups of keywords
    morekeywords=[1]{Domain},
    keywordstyle=[1]\color{red}\bfseries,
    morekeywords=[2]{Objects, Primitive, Goal, Initial, Plan, plan},
    keywordstyle=[2]\bfseries,
    morekeywords=[3]{UNLOAD, TRUCK, UNLOAD, AIRPLANE, LOAD, TRUCK, FLY, AIRPLANE, DRIVE, TRUCK, LOAD, AIRPLANE },
    keywordstyle=[3]\color{orange}\bfseries,
    morekeywords=[4]{p0, t0, p3, p6, p4, p5, l0-0, l0-1, c0, p1, p8, p7, p2, a0 },
    keywordstyle=[4]\color{blue}\bfseries,
}

\begin{figure*}
\footnotesize
\begin{lstlisting}[basicstyle=\footnotesize\ttfamily]
Domain: logistics
Types: object
Predicates: airplane/1, airport/1, at/2, city/1, in/2, in-city/2, location/1, package/1, truck/1
Action schemas:
load-truck(?obj: object, ?truck: object, ?loc: object)
pre:  +package(?obj),  +truck(?truck),  +location(?loc),  +at(?truck, ?loc),  +at(?obj, ?loc)
eff:  -at(?obj, ?loc),  +in(?obj, ?truck)
load-airplane(?obj: object, ?airplane: object, ?loc: object)
pre:  +package(?obj),  +airplane(?airplane),  +location(?loc),  +at(?obj, ?loc),  +at(?airplane, ?loc)
eff:  -at(?obj, ?loc),  +in(?obj, ?airplane)
unload-truck(?obj: object, ?truck: object, ?loc: object)
pre:  +package(?obj),  +truck(?truck),  +location(?loc),  +at(?truck, ?loc),  +in(?obj, ?truck)
eff:  -in(?obj, ?truck),  +at(?obj, ?loc)
unload-airplane(?obj: object, ?airplane: object, ?loc: object)
pre:  +package(?obj),  +airplane(?airplane),  +location(?loc),  +in(?obj, ?airplane),  +at(?airplane, ?loc)
eff:  -in(?obj, ?airplane),  +at(?obj, ?loc)
drive-truck(?truck: object, ?loc-from: object, ?loc-to: object, ?city: object)
pre:  +truck(?truck),  +location(?loc-from),  +location(?loc-to),  +city(?city),  +at(?truck, ?loc-from),  +in-city(?loc-from, ?city),  +in-city(?loc-to, ?city)
eff:  -at(?truck, ?loc-from),  +at(?truck, ?loc-to)
fly-airplane(?airplane: object, ?loc-from: object, ?loc-to: object)
pre:  +airplane(?airplane),  +airport(?loc-from),  +airport(?loc-to),  +at(?airplane, ?loc-from)
eff:  -at(?airplane, ?loc-from),  +at(?airplane, ?loc-to)

Name: logistics-c1-s2-p9-a1 (logistics_a-1_c-1_s-2_p-9_t-1.pddl)
Objects: 
    a0, c0, l0-0, l0-1, p0, p1, p2, p3, p4, p5, p6, p7, p8, t0
Initial: 
    package(p0), package(p1), package(p2), package(p3), package(p4), package(p5)
package(p6), package(p7), package(p8), truck(t0), location(l0-0), location(l0-1)
airplane(a0), city(c0), airport(l0-0), at(a0, l0-0), at(p0, l0-0), at(p1, l0-0)
at(p3, l0-0), at(p6, l0-0), at(p8, l0-0), at(t0, l0-1), at(p2, l0-1), at(p4
l0-1), at(p5, l0-1), at(p7, l0-1), in-city(l0-0, c0), in-city(l0-1, c0)
Goal: 
    at(p0, l0-0), at(p1, l0-1), at(p2, l0-0), at(p3, l0-1), at(p4, l0-1), at(p5
l0-1), at(p6, l0-1), at(p7, l0-1), at(p8, l0-1)

Plan has path-cycle: unchecked
Plan has subgoal-cycle: false
Primitive plan: 18
Plan: 10
1  drive-truck(t0, l0-1, l0-0, c0) -> load-truck(p6, t0, l0-0)
2  drive-truck(t0, l0-0, l0-1, c0) -> unload-truck(p6, t0, l0-1)
3  drive-truck(t0, l0-1, l0-0, c0) -> load-truck(p3, t0, l0-0)
4  drive-truck(t0, l0-0, l0-1, c0) -> unload-truck(p3, t0, l0-1)
5  drive-truck(t0, l0-1, l0-0, c0) -> load-truck(p1, t0, l0-0)
6  drive-truck(t0, l0-0, l0-1, c0) -> unload-truck(p1, t0, l0-1)
7  load-truck(p2, t0, l0-1)
8  drive-truck(t0, l0-1, l0-0, c0) -> load-truck(p8, t0, l0-0)
9  unload-truck(p2, t0, l0-0)
10 drive-truck(t0, l0-0, l0-1, c0) -> unload-truck(p8, t0, l0-1)
\end{lstlisting}
\end{figure*}

\clearpage

\lstset{
    basicstyle=\footnotesize\ttfamily,
    keywordstyle=\bfseries, % This will apply bold to all keywords
    % Define colors for different groups of keywords
    morekeywords=[1]{Domain},
    keywordstyle=[1]\color{red}\bfseries,
    morekeywords=[2]{Objects, Primitive, Goal, Initial, Plan, plan},
    keywordstyle=[2]\bfseries,
    morekeywords=[3]{UNLOAD, TRUCK, UNLOAD, AIRPLANE, LOAD, TRUCK, FLY, AIRPLANE, DRIVE, TRUCK, LOAD, AIRPLANE },
    keywordstyle=[3]\color{orange}\bfseries,
    morekeywords=[4]{p0, t0, p3, p6, p4, p5, l0-0, l0-1, c0, p1, p8, p7, p2, a0 },
    keywordstyle=[4]\color{blue}\bfseries,
}

\begin{figure*}
\footnotesize
\begin{lstlisting}[basicstyle=\footnotesize\ttfamily]
Name: logistics-c1-s2-p9-a1 (logistics_a-1_c-1_s-2_p-9_t-1.pddl)
Objects: 
    a0, c0, l0-0, l0-1, p0, p1, p2, p3, p4, p5, p6, p7, p8, t0
Initial: 
    package(p0), package(p1), package(p2), package(p3), package(p4), package(p5)
package(p6), package(p7), package(p8), truck(t0), location(l0-0), location(l0-1)
airplane(a0), city(c0), airport(l0-0), at(a0, l0-0), at(p0, l0-0), at(p1, l0-0)
at(p3, l0-0), at(p6, l0-0), at(p8, l0-0), at(t0, l0-1), at(p2, l0-1), at(p4
l0-1), at(p5, l0-1), at(p7, l0-1), in-city(l0-0, c0), in-city(l0-1, c0)
Goal: 
    at(p0, l0-0), at(p1, l0-1), at(p2, l0-0), at(p3, l0-1), at(p4, l0-1), at(p5
l0-1), at(p6, l0-1), at(p7, l0-1), at(p8, l0-1)

Plan has path-cycle: unchecked
Plan has subgoal-cycle: false
Primitive plan: 18
Plan: 10
1  drive-truck(t0, l0-1, l0-0, c0) -> load-truck(p6, t0, l0-0)
2  drive-truck(t0, l0-0, l0-1, c0) -> unload-truck(p6, t0, l0-1)
3  drive-truck(t0, l0-1, l0-0, c0) -> load-truck(p8, t0, l0-0)
4  drive-truck(t0, l0-0, l0-1, c0) -> unload-truck(p8, t0, l0-1)
5  drive-truck(t0, l0-1, l0-0, c0) -> load-truck(p1, t0, l0-0)
6  drive-truck(t0, l0-0, l0-1, c0) -> unload-truck(p1, t0, l0-1)
7  load-truck(p2, t0, l0-1)
8  drive-truck(t0, l0-1, l0-0, c0) -> load-truck(p3, t0, l0-0)
9  unload-truck(p2, t0, l0-0)
10 drive-truck(t0, l0-0, l0-1, c0) -> unload-truck(p3, t0, l0-1)
\end{lstlisting}
\end{figure*}

\clearpage

\lstset{
    basicstyle=\footnotesize\ttfamily,
    keywordstyle=\bfseries, % This will apply bold to all keywords
    % Define colors for different groups of keywords
    morekeywords=[1]{Domain},
    keywordstyle=[1]\color{red}\bfseries,
    morekeywords=[2]{Objects, Primitive, Goal, Initial, Plan, plan},
    keywordstyle=[2]\bfseries,
    morekeywords=[3]{UNLOAD, TRUCK, UNLOAD, AIRPLANE, LOAD, TRUCK, FLY, AIRPLANE, DRIVE, TRUCK, LOAD, AIRPLANE },
    keywordstyle=[3]\color{orange}\bfseries,
    morekeywords=[4]{p0, t0, p3, p6, p4, p5, l0-0, l0-1, c0, p1, p8, p7, p2, a0 },
    keywordstyle=[4]\color{blue}\bfseries,
}

\begin{figure*}
\footnotesize
\begin{lstlisting}[basicstyle=\footnotesize\ttfamily]
Name: logistics-c1-s2-p9-a1 (logistics_a-1_c-1_s-2_p-9_t-1.pddl)
Objects: 
    a0, c0, l0-0, l0-1, p0, p1, p2, p3, p4, p5, p6, p7, p8, t0
Initial: 
    package(p0), package(p1), package(p2), package(p3), package(p4), package(p5)
package(p6), package(p7), package(p8), truck(t0), location(l0-0), location(l0-1)
airplane(a0), city(c0), airport(l0-0), at(a0, l0-0), at(p0, l0-0), at(p1, l0-0)
at(p3, l0-0), at(p6, l0-0), at(p8, l0-0), at(t0, l0-1), at(p2, l0-1), at(p4
l0-1), at(p5, l0-1), at(p7, l0-1), in-city(l0-0, c0), in-city(l0-1, c0)
Goal: 
    at(p0, l0-0), at(p1, l0-1), at(p2, l0-0), at(p3, l0-1), at(p4, l0-1), at(p5
l0-1), at(p6, l0-1), at(p7, l0-1), at(p8, l0-1)

Plan has path-cycle: unchecked
Plan has subgoal-cycle: false
Primitive plan: 18
Plan: 10
1  drive-truck(t0, l0-1, l0-0, c0) -> load-truck(p1, t0, l0-0)
2  drive-truck(t0, l0-0, l0-1, c0) -> unload-truck(p1, t0, l0-1)
3  drive-truck(t0, l0-1, l0-0, c0) -> load-truck(p6, t0, l0-0)
4  drive-truck(t0, l0-0, l0-1, c0) -> unload-truck(p6, t0, l0-1)
5  drive-truck(t0, l0-1, l0-0, c0) -> load-truck(p3, t0, l0-0)
6  drive-truck(t0, l0-0, l0-1, c0) -> unload-truck(p3, t0, l0-1)
7  load-truck(p2, t0, l0-1)
8  drive-truck(t0, l0-1, l0-0, c0) -> load-truck(p8, t0, l0-0)
9  unload-truck(p2, t0, l0-0)
10 drive-truck(t0, l0-0, l0-1, c0) -> unload-truck(p8, t0, l0-1)
\end{lstlisting}
\end{figure*}

\clearpage

\lstset{
    basicstyle=\footnotesize\ttfamily,
    keywordstyle=\bfseries, % This will apply bold to all keywords
    % Define colors for different groups of keywords
    morekeywords=[1]{Domain},
    keywordstyle=[1]\color{red}\bfseries,
    morekeywords=[2]{Objects, Primitive, Goal, Initial, Plan, plan},
    keywordstyle=[2]\bfseries,
    morekeywords=[3]{UNLOAD, TRUCK, UNLOAD, AIRPLANE, LOAD, TRUCK, FLY, AIRPLANE, DRIVE, TRUCK, LOAD, AIRPLANE },
    keywordstyle=[3]\color{orange}\bfseries,
    morekeywords=[4]{p0, t0, p3, p6, p4, p5, l0-0, l0-1, c0, p1, p8, p7, p2, a0 },
    keywordstyle=[4]\color{blue}\bfseries,
}

\begin{figure*}
\footnotesize
\begin{lstlisting}[basicstyle=\footnotesize\ttfamily]
Name: logistics-c1-s2-p9-a1 (logistics_a-1_c-1_s-2_p-9_t-1.pddl)
Objects: 
    a0, c0, l0-0, l0-1, p0, p1, p2, p3, p4, p5, p6, p7, p8, t0
Initial: 
    package(p0), package(p1), package(p2), package(p3), package(p4), package(p5)
package(p6), package(p7), package(p8), truck(t0), location(l0-0), location(l0-1)
airplane(a0), city(c0), airport(l0-0), at(a0, l0-0), at(p0, l0-0), at(p1, l0-0)
at(p3, l0-0), at(p6, l0-0), at(p8, l0-0), at(t0, l0-1), at(p2, l0-1), at(p4
l0-1), at(p5, l0-1), at(p7, l0-1), in-city(l0-0, c0), in-city(l0-1, c0)
Goal: 
    at(p0, l0-0), at(p1, l0-1), at(p2, l0-0), at(p3, l0-1), at(p4, l0-1), at(p5
l0-1), at(p6, l0-1), at(p7, l0-1), at(p8, l0-1)

Plan has path-cycle: unchecked
Plan has subgoal-cycle: false
Primitive plan: 18
Plan: 10
1  drive-truck(t0, l0-1, l0-0, c0) -> load-truck(p8, t0, l0-0)
2  drive-truck(t0, l0-0, l0-1, c0) -> unload-truck(p8, t0, l0-1)
3  drive-truck(t0, l0-1, l0-0, c0) -> load-truck(p6, t0, l0-0)
4  drive-truck(t0, l0-0, l0-1, c0) -> unload-truck(p6, t0, l0-1)
5  drive-truck(t0, l0-1, l0-0, c0) -> load-truck(p1, t0, l0-0)
6  drive-truck(t0, l0-0, l0-1, c0) -> unload-truck(p1, t0, l0-1)
7  load-truck(p2, t0, l0-1)
8  drive-truck(t0, l0-1, l0-0, c0) -> load-truck(p3, t0, l0-0)
9  unload-truck(p2, t0, l0-0)
10 drive-truck(t0, l0-0, l0-1, c0) -> unload-truck(p3, t0, l0-1)
\end{lstlisting}
\end{figure*}

\clearpage

\lstset{
    basicstyle=\footnotesize\ttfamily,
    keywordstyle=\bfseries, % This will apply bold to all keywords
    % Define colors for different groups of keywords
    morekeywords=[1]{Domain},
    keywordstyle=[1]\color{red}\bfseries,
    morekeywords=[2]{Objects, Primitive, Goal, Initial, Plan, plan},
    keywordstyle=[2]\bfseries,
    morekeywords=[3]{UNLOAD, TRUCK, UNLOAD, AIRPLANE, LOAD, TRUCK, FLY, AIRPLANE, DRIVE, TRUCK, LOAD, AIRPLANE },
    keywordstyle=[3]\color{orange}\bfseries,
    morekeywords=[4]{t1, l1-1, t0, p0, p3, l1-0, p4, l0-0, c1, l0-1, c0, p1, p5, p2, a0 },
    keywordstyle=[4]\color{blue}\bfseries,
}

\begin{figure*}
\footnotesize
\begin{lstlisting}[basicstyle=\footnotesize\ttfamily]
Name: logistics-c2-s2-p6-a1 (logistics_a-1_c-2_s-2_p-6_t-2.pddl)
Objects: 
    a0, c0, c1, l0-0, l0-1, l1-0, l1-1, p0, p1, p2, p3, p4, p5, t0, t1
Initial: 
    package(p0), package(p1), package(p2), package(p3), package(p4), package(p5)
truck(t0), truck(t1), location(l0-0), location(l0-1), location(l1-0)
location(l1-1), airplane(a0), city(c0), city(c1), airport(l0-0), airport(l1-0)
at(p0, l0-0), at(p3, l0-0), at(t0, l0-1), at(p1, l0-1), at(a0, l1-0), at(p2
l1-0), at(p4, l1-0), at(t1, l1-1), at(p5, l1-1), in-city(l0-0, c0), in-city(l0-1
c0), in-city(l1-0, c1), in-city(l1-1, c1)
Goal: 
    at(p0, l0-0), at(p1, l1-0), at(p2, l0-0), at(p3, l0-0), at(p4, l1-1), at(p5
l0-1)

Plan has path-cycle: unchecked
Plan has subgoal-cycle: false
Primitive plan: 34
Plan: 20
1  drive-truck(t1, l1-1, l1-0, c1) -> load-truck(p2, t1, l1-0)
2  load-truck(p1, t0, l0-1)
3  drive-truck(t1, l1-0, l1-1, c1) -> load-truck(p5, t1, l1-1)
4  drive-truck(t1, l1-1, l1-0, c1) -> load-truck(p4, t1, l1-0)
5  drive-truck(t1, l1-0, l1-1, c1) -> unload-truck(p4, t1, l1-1)
6  fly-airplane(a0, l1-0, l0-0)
7  drive-truck(t0, l0-1, l0-0, c0)
8  fly-airplane(a0, l0-0, l1-0)
9  drive-truck(t1, l1-1, l1-0, c1) -> unload-truck(p2, t1, l1-0) -> load-airplane(p2, a0, l1-0)
10 fly-airplane(a0, l1-0, l0-0) -> unload-airplane(p2, a0, l0-0)
11 drive-truck(t1, l1-0, l1-1, c1)
12 drive-truck(t0, l0-0, l0-1, c0)
13 fly-airplane(a0, l0-0, l1-0)
14 drive-truck(t1, l1-1, l1-0, c1)
15 fly-airplane(a0, l1-0, l0-0)
16 drive-truck(t0, l0-1, l0-0, c0) -> unload-truck(p1, t0, l0-0) -> load-airplane(p1, a0, l0-0)
17 fly-airplane(a0, l0-0, l1-0) -> unload-airplane(p1, a0, l1-0)
18 unload-truck(p5, t1, l1-0) -> load-airplane(p5, a0, l1-0)
19 fly-airplane(a0, l1-0, l0-0) -> unload-airplane(p5, a0, l0-0) -> load-truck(p5, t0, l0-0)
20 drive-truck(t0, l0-0, l0-1, c0) -> unload-truck(p5, t0, l0-1)
\end{lstlisting}
\end{figure*}

\clearpage

\lstset{
    basicstyle=\footnotesize\ttfamily,
    keywordstyle=\bfseries, % This will apply bold to all keywords
    % Define colors for different groups of keywords
    morekeywords=[1]{Domain},
    keywordstyle=[1]\color{red}\bfseries,
    morekeywords=[2]{Objects, Primitive, Goal, Initial, Plan, plan},
    keywordstyle=[2]\bfseries,
    morekeywords=[3]{UNLOAD, TRUCK, UNLOAD, AIRPLANE, LOAD, TRUCK, FLY, AIRPLANE, DRIVE, TRUCK, LOAD, AIRPLANE },
    keywordstyle=[3]\color{orange}\bfseries,
    morekeywords=[4]{t1, l1-1, t0, p0, p3, l1-0, p4, l0-0, c1, l0-1, c0, p1, p5, p2, a0 },
    keywordstyle=[4]\color{blue}\bfseries,
}

\begin{figure*}
\footnotesize
\begin{lstlisting}[basicstyle=\footnotesize\ttfamily]
Name: logistics-c2-s2-p6-a1 (logistics_a-1_c-2_s-2_p-6_t-2.pddl)
Objects: 
    a0, c0, c1, l0-0, l0-1, l1-0, l1-1, p0, p1, p2, p3, p4, p5, t0, t1
Initial: 
    package(p0), package(p1), package(p2), package(p3), package(p4), package(p5)
truck(t0), truck(t1), location(l0-0), location(l0-1), location(l1-0)
location(l1-1), airplane(a0), city(c0), city(c1), airport(l0-0), airport(l1-0)
at(p0, l0-0), at(p3, l0-0), at(t0, l0-1), at(p1, l0-1), at(a0, l1-0), at(p2
l1-0), at(p4, l1-0), at(t1, l1-1), at(p5, l1-1), in-city(l0-0, c0), in-city(l0-1
c0), in-city(l1-0, c1), in-city(l1-1, c1)
Goal: 
    at(p0, l0-0), at(p1, l1-0), at(p2, l0-0), at(p3, l0-0), at(p4, l1-1), at(p5
l0-1)

Plan has path-cycle: unchecked
Plan has subgoal-cycle: false
Primitive plan: 34
Plan: 20
1  drive-truck(t1, l1-1, l1-0, c1) -> load-truck(p2, t1, l1-0)
2  load-truck(p1, t0, l0-1)
3  drive-truck(t1, l1-0, l1-1, c1) -> load-truck(p5, t1, l1-1)
4  drive-truck(t1, l1-1, l1-0, c1) -> load-truck(p4, t1, l1-0)
5  drive-truck(t1, l1-0, l1-1, c1) -> unload-truck(p4, t1, l1-1)
6  fly-airplane(a0, l1-0, l0-0)
7  drive-truck(t0, l0-1, l0-0, c0)
8  fly-airplane(a0, l0-0, l1-0)
9  drive-truck(t1, l1-1, l1-0, c1) -> unload-truck(p2, t1, l1-0) -> load-airplane(p2, a0, l1-0)
10 fly-airplane(a0, l1-0, l0-0) -> unload-airplane(p2, a0, l0-0)
11 drive-truck(t1, l1-0, l1-1, c1)
12 drive-truck(t0, l0-0, l0-1, c0)
13 fly-airplane(a0, l0-0, l1-0)
14 drive-truck(t1, l1-1, l1-0, c1)
15 fly-airplane(a0, l1-0, l0-0)
16 drive-truck(t0, l0-1, l0-0, c0) -> unload-truck(p1, t0, l0-0) -> load-airplane(p1, a0, l0-0)
17 fly-airplane(a0, l0-0, l1-0) -> unload-airplane(p1, a0, l1-0)
18 unload-truck(p5, t1, l1-0) -> load-airplane(p5, a0, l1-0)
19 fly-airplane(a0, l1-0, l0-0) -> unload-airplane(p5, a0, l0-0) -> load-truck(p5, t0, l0-0)
20 drive-truck(t0, l0-0, l0-1, c0) -> unload-truck(p5, t0, l0-1)
\end{lstlisting}
\end{figure*}

\clearpage

\lstset{
    basicstyle=\footnotesize\ttfamily,
    keywordstyle=\bfseries, % This will apply bold to all keywords
    % Define colors for different groups of keywords
    morekeywords=[1]{Domain},
    keywordstyle=[1]\color{red}\bfseries,
    morekeywords=[2]{Objects, Primitive, Goal, Initial, Plan, plan},
    keywordstyle=[2]\bfseries,
    morekeywords=[3]{UNLOAD, TRUCK, UNLOAD, AIRPLANE, LOAD, TRUCK, FLY, AIRPLANE, DRIVE, TRUCK, LOAD, AIRPLANE },
    keywordstyle=[3]\color{orange}\bfseries,
    morekeywords=[4]{t1, l1-1, t0, p0, p3, p6, l1-0, p4, l0-0, c1, l0-1, c0, p1, p5, p8, p7, p2, a0 },
    keywordstyle=[4]\color{blue}\bfseries,
}

\lstset{
    basicstyle=\footnotesize\ttfamily,
    keywordstyle=\bfseries, % This will apply bold to all keywords
    % Define colors for different groups of keywords
    morekeywords=[1]{Domain},
    keywordstyle=[1]\color{red}\bfseries,
    morekeywords=[2]{Objects, Primitive, Goal, Initial, Plan, plan},
    keywordstyle=[2]\bfseries,
    morekeywords=[3]{UNLOAD, TRUCK, UNLOAD, AIRPLANE, LOAD, TRUCK, FLY, AIRPLANE, DRIVE, TRUCK, LOAD, AIRPLANE },
    keywordstyle=[3]\color{orange}\bfseries,
    morekeywords=[4]{t1, l1-1, t0, p0, p3, p6, l1-0, p4, l0-0, c1, l0-1, c0, p1, p5, p8, p7, p2, a0 },
    keywordstyle=[4]\color{blue}\bfseries,
}

\lstset{
    basicstyle=\footnotesize\ttfamily,
    keywordstyle=\bfseries, % This will apply bold to all keywords
    % Define colors for different groups of keywords
    morekeywords=[1]{Domain},
    keywordstyle=[1]\color{red}\bfseries,
    morekeywords=[2]{Objects, Primitive, Goal, Initial, Plan, plan},
    keywordstyle=[2]\bfseries,
    morekeywords=[3]{UNLOAD, TRUCK, UNLOAD, AIRPLANE, LOAD, TRUCK, FLY, AIRPLANE, DRIVE, TRUCK, LOAD, AIRPLANE },
    keywordstyle=[3]\color{orange}\bfseries,
    morekeywords=[4]{t1, l1-1, t0, t2, p0, c2, l2-1, p3, l2-0, l1-0, p4, l0-0, c1, l0-1, c0, p1, p2, a0 },
    keywordstyle=[4]\color{blue}\bfseries,
}

\begin{figure*}
\footnotesize
\begin{lstlisting}[basicstyle=\footnotesize\ttfamily]
Name: logistics-c3-s2-p5-a1 (logistics_a-1_c-3_s-2_p-5_t-3.pddl)
Objects: 
    a0, c0, c1, c2, l0-0, l0-1, l1-0, l1-1, l2-0, l2-1, p0, p1, p2, p3, p4, t0, t1
t2
Initial: 
    package(p0), package(p1), package(p2), package(p3), package(p4), truck(t0)
truck(t1), truck(t2), location(l0-0), location(l0-1), location(l1-0)
location(l1-1), location(l2-0), location(l2-1), airplane(a0), city(c0), city(c1)
city(c2), airport(l0-0), airport(l1-0), airport(l2-0), at(a0, l0-0), at(p0
l0-0), at(t0, l0-1), at(p2, l1-0), at(t1, l1-1), at(p4, l1-1), at(t2, l2-0)
at(p1, l2-1), at(p3, l2-1), in-city(l0-0, c0), in-city(l0-1, c0), in-city(l1-0
c1), in-city(l1-1, c1), in-city(l2-0, c2), in-city(l2-1, c2)
Goal: 
    at(p0, l2-0), at(p1, l2-1), at(p2, l1-0), at(p3, l1-0), at(p4, l0-1)

Plan has path-cycle: unchecked
Plan has subgoal-cycle: false
Primitive plan: 55
Plan: 38
1  drive-truck(t2, l2-0, l2-1, c2) -> load-truck(p3, t2, l2-1)
2  load-truck(p4, t1, l1-1)
3  drive-truck(t0, l0-1, l0-0, c0) -> load-truck(p0, t0, l0-0)
4  drive-truck(t0, l0-0, l0-1, c0)
5  fly-airplane(a0, l0-0, l1-0)
6  drive-truck(t2, l2-1, l2-0, c2)
7  fly-airplane(a0, l1-0, l2-0)
8  drive-truck(t2, l2-0, l2-1, c2)
9  drive-truck(t2, l2-1, l2-0, c2) -> unload-truck(p3, t2, l2-0) -> load-airplane(p3, a0, l2-0)
10 fly-airplane(a0, l2-0, l1-0) -> unload-airplane(p3, a0, l1-0)
11 drive-truck(t1, l1-1, l1-0, c1) -> unload-truck(p4, t1, l1-0) -> load-airplane(p4, a0, l1-0)
12 fly-airplane(a0, l1-0, l2-0) -> unload-airplane(p4, a0, l2-0) -> load-truck(p4, t2, l2-0)
13 drive-truck(t2, l2-0, l2-1, c2)
14 drive-truck(t1, l1-0, l1-1, c1)
15 fly-airplane(a0, l2-0, l0-0)
16 drive-truck(t1, l1-1, l1-0, c1)
17 fly-airplane(a0, l0-0, l1-0)
18 drive-truck(t1, l1-0, l1-1, c1)
19 drive-truck(t2, l2-1, l2-0, c2)
20 fly-airplane(a0, l1-0, l2-0)
21 fly-airplane(a0, l2-0, l0-0)
22 drive-truck(t1, l1-1, l1-0, c1)
23 fly-airplane(a0, l0-0, l1-0)
24 drive-truck(t0, l0-1, l0-0, c0)
25 drive-truck(t2, l2-0, l2-1, c2)
26 fly-airplane(a0, l1-0, l0-0)
27 drive-truck(t2, l2-1, l2-0, c2)
28 drive-truck(t1, l1-0, l1-1, c1)
29 drive-truck(t2, l2-0, l2-1, c2)
30 fly-airplane(a0, l0-0, l2-0)
31 drive-truck(t2, l2-1, l2-0, c2)
32 drive-truck(t1, l1-1, l1-0, c1)
33 drive-truck(t2, l2-0, l2-1, c2)
34 drive-truck(t2, l2-1, l2-0, c2) -> unload-truck(p4, t2, l2-0) -> load-airplane(p4, a0, l2-0)
35 fly-airplane(a0, l2-0, l0-0) -> unload-airplane(p4, a0, l0-0) -> load-truck(p4, t0, l0-0)
36 drive-truck(t0, l0-0, l0-1, c0) -> unload-truck(p4, t0, l0-1)
37 drive-truck(t0, l0-1, l0-0, c0) -> unload-truck(p0, t0, l0-0) -> load-airplane(p0, a0, l0-0)
38 fly-airplane(a0, l0-0, l2-0) -> unload-airplane(p0, a0, l2-0)
\end{lstlisting}
\end{figure*}

\clearpage

\lstset{
    basicstyle=\footnotesize\ttfamily,
    keywordstyle=\bfseries, % This will apply bold to all keywords
    % Define colors for different groups of keywords
    morekeywords=[1]{Domain},
    keywordstyle=[1]\color{red}\bfseries,
    morekeywords=[2]{Objects, Primitive, Goal, Initial, Plan, plan},
    keywordstyle=[2]\bfseries,
    morekeywords=[3]{UNLOAD, TRUCK, UNLOAD, AIRPLANE, LOAD, TRUCK, FLY, AIRPLANE, DRIVE, TRUCK, LOAD, AIRPLANE },
    keywordstyle=[3]\color{orange}\bfseries,
    morekeywords=[4]{t1, l1-1, t0, t2, p0, c2, l2-1, p3, l2-0, l1-0, p4, l0-0, c1, l0-1, c0, p1, p2, a0 },
    keywordstyle=[4]\color{blue}\bfseries,
}

\begin{figure*}
\footnotesize
\begin{lstlisting}[basicstyle=\footnotesize\ttfamily]
Name: logistics-c3-s2-p5-a1 (logistics_a-1_c-3_s-2_p-5_t-3.pddl)
Objects: 
    a0, c0, c1, c2, l0-0, l0-1, l1-0, l1-1, l2-0, l2-1, p0, p1, p2, p3, p4, t0, t1
t2
Initial: 
    package(p0), package(p1), package(p2), package(p3), package(p4), truck(t0)
truck(t1), truck(t2), location(l0-0), location(l0-1), location(l1-0)
location(l1-1), location(l2-0), location(l2-1), airplane(a0), city(c0), city(c1)
city(c2), airport(l0-0), airport(l1-0), airport(l2-0), at(a0, l0-0), at(p0
l0-0), at(t0, l0-1), at(p2, l1-0), at(t1, l1-1), at(p4, l1-1), at(t2, l2-0)
at(p1, l2-1), at(p3, l2-1), in-city(l0-0, c0), in-city(l0-1, c0), in-city(l1-0
c1), in-city(l1-1, c1), in-city(l2-0, c2), in-city(l2-1, c2)
Goal: 
    at(p0, l2-0), at(p1, l2-1), at(p2, l1-0), at(p3, l1-0), at(p4, l0-1)

Plan has path-cycle: unchecked
Plan has subgoal-cycle: false
Primitive plan: 58
Plan: 41
1  drive-truck(t2, l2-0, l2-1, c2) -> load-truck(p3, t2, l2-1)
2  load-truck(p4, t1, l1-1)
3  drive-truck(t0, l0-1, l0-0, c0) -> load-truck(p0, t0, l0-0)
4  drive-truck(t0, l0-0, l0-1, c0)
5  fly-airplane(a0, l0-0, l1-0)
6  drive-truck(t2, l2-1, l2-0, c2)
7  fly-airplane(a0, l1-0, l2-0)
8  drive-truck(t2, l2-0, l2-1, c2)
9  drive-truck(t2, l2-1, l2-0, c2) -> unload-truck(p3, t2, l2-0) -> load-airplane(p3, a0, l2-0)
10 fly-airplane(a0, l2-0, l1-0) -> unload-airplane(p3, a0, l1-0)
11 drive-truck(t1, l1-1, l1-0, c1) -> unload-truck(p4, t1, l1-0) -> load-airplane(p4, a0, l1-0)
12 fly-airplane(a0, l1-0, l2-0) -> unload-airplane(p4, a0, l2-0) -> load-truck(p4, t2, l2-0)
13 drive-truck(t2, l2-0, l2-1, c2)
14 fly-airplane(a0, l2-0, l0-0)
15 drive-truck(t1, l1-0, l1-1, c1)
16 fly-airplane(a0, l0-0, l2-0)
17 drive-truck(t2, l2-1, l2-0, c2)
18 fly-airplane(a0, l2-0, l0-0)
19 drive-truck(t1, l1-1, l1-0, c1)
20 fly-airplane(a0, l0-0, l1-0)
21 drive-truck(t2, l2-0, l2-1, c2)
22 drive-truck(t1, l1-0, l1-1, c1)
23 drive-truck(t2, l2-1, l2-0, c2)
24 drive-truck(t0, l0-1, l0-0, c0)
25 drive-truck(t2, l2-0, l2-1, c2)
26 fly-airplane(a0, l1-0, l0-0)
27 drive-truck(t1, l1-1, l1-0, c1)
28 drive-truck(t2, l2-1, l2-0, c2)
29 drive-truck(t1, l1-0, l1-1, c1)
30 fly-airplane(a0, l0-0, l2-0)
31 drive-truck(t2, l2-0, l2-1, c2)
32 drive-truck(t1, l1-1, l1-0, c1)
33 drive-truck(t2, l2-1, l2-0, c2)
34 fly-airplane(a0, l2-0, l1-0)
35 drive-truck(t2, l2-0, l2-1, c2)
36 drive-truck(t2, l2-1, l2-0, c2) -> unload-truck(p4, t2, l2-0)
37 fly-airplane(a0, l1-0, l2-0) -> load-airplane(p4, a0, l2-0)
38 fly-airplane(a0, l2-0, l0-0) -> unload-airplane(p4, a0, l0-0) -> load-truck(p4, t0, l0-0)
39 drive-truck(t0, l0-0, l0-1, c0) -> unload-truck(p4, t0, l0-1)
40 drive-truck(t0, l0-1, l0-0, c0) -> unload-truck(p0, t0, l0-0) -> load-airplane(p0, a0, l0-0)
41 fly-airplane(a0, l0-0, l2-0) -> unload-airplane(p0, a0, l2-0)
\end{lstlisting}
\end{figure*}

\clearpage

\lstset{
    basicstyle=\footnotesize\ttfamily,
    keywordstyle=\bfseries, % This will apply bold to all keywords
    % Define colors for different groups of keywords
    morekeywords=[1]{Domain},
    keywordstyle=[1]\color{red}\bfseries,
    morekeywords=[2]{Objects, Primitive, Goal, Initial, Plan, plan},
    keywordstyle=[2]\bfseries,
    morekeywords=[3]{UNLOAD, TRUCK, UNLOAD, AIRPLANE, LOAD, TRUCK, FLY, AIRPLANE, DRIVE, TRUCK, LOAD, AIRPLANE },
    keywordstyle=[3]\color{orange}\bfseries,
    morekeywords=[4]{t2, p3, l1-0, l0-1, p2, l3-0, p1, l3-1, t1, t0, l2-0, l0-0, t3, l1-1, p0, c2, l2-1, c3, c1, c0, a0 },
    keywordstyle=[4]\color{blue}\bfseries,
}

\begin{figure*}
\footnotesize
\begin{lstlisting}[basicstyle=\footnotesize\ttfamily]
Name: logistics-c4-s2-p4-a1 (logistics_a-1_c-4_s-2_p-4_t-4.pddl)
Objects: 
    a0, c0, c1, c2, c3, l0-0, l0-1, l1-0, l1-1, l2-0, l2-1, l3-0, l3-1, p0, p1, p2
p3, t0, t1, t2, t3
Initial: 
    package(p0), package(p1), package(p2), package(p3), truck(t0), truck(t1)
truck(t2), truck(t3), location(l0-0), location(l0-1), location(l1-0)
location(l1-1), location(l2-0), location(l2-1), location(l3-0), location(l3-1)
airplane(a0), city(c0), city(c1), city(c2), city(c3), airport(l0-0)
airport(l1-0), airport(l2-0), airport(l3-0), at(t0, l0-1), at(p0, l0-1), at(p3
l1-0), at(t1, l1-1), at(a0, l2-0), at(t2, l2-0), at(p2, l2-0), at(t3, l3-0)
at(p1, l3-0), in-city(l0-0, c0), in-city(l0-1, c0), in-city(l1-0, c1)
in-city(l1-1, c1), in-city(l2-0, c2), in-city(l2-1, c2), in-city(l3-0, c3)
in-city(l3-1, c3)
Goal: 
    at(p0, l3-1), at(p1, l2-0), at(p2, l1-0), at(p3, l0-0)

Plan has path-cycle: unchecked
Plan has subgoal-cycle: false
Primitive plan: 24
Plan: 12
1  load-truck(p0, t0, l0-1)
2  load-truck(p1, t3, l3-0)
3  drive-truck(t1, l1-1, l1-0, c1) -> load-truck(p3, t1, l1-0)
4  load-airplane(p2, a0, l2-0)
5  fly-airplane(a0, l2-0, l1-0) -> unload-airplane(p2, a0, l1-0)
6  unload-truck(p3, t1, l1-0) -> load-airplane(p3, a0, l1-0)
7  fly-airplane(a0, l1-0, l0-0) -> unload-airplane(p3, a0, l0-0)
8  drive-truck(t0, l0-1, l0-0, c0) -> unload-truck(p0, t0, l0-0) -> load-airplane(p0, a0, l0-0)
9  fly-airplane(a0, l0-0, l3-0) -> unload-airplane(p0, a0, l3-0) -> load-truck(p0, t3, l3-0)
10 drive-truck(t3, l3-0, l3-1, c3) -> unload-truck(p0, t3, l3-1)
11 drive-truck(t3, l3-1, l3-0, c3) -> unload-truck(p1, t3, l3-0) -> load-airplane(p1, a0, l3-0)
12 fly-airplane(a0, l3-0, l2-0) -> unload-airplane(p1, a0, l2-0)
\end{lstlisting}
\end{figure*}

\clearpage

\lstset{
    basicstyle=\footnotesize\ttfamily,
    keywordstyle=\bfseries, % This will apply bold to all keywords
    % Define colors for different groups of keywords
    morekeywords=[1]{Domain},
    keywordstyle=[1]\color{red}\bfseries,
    morekeywords=[2]{Objects, Primitive, Goal, Initial, Plan, plan},
    keywordstyle=[2]\bfseries,
    morekeywords=[3]{UNLOAD, TRUCK, UNLOAD, AIRPLANE, LOAD, TRUCK, FLY, AIRPLANE, DRIVE, TRUCK, LOAD, AIRPLANE },
    keywordstyle=[3]\color{orange}\bfseries,
    morekeywords=[4]{t2, p3, l1-0, l0-1, p2, l3-0, p1, l3-1, t1, t0, l2-0, l0-0, t3, l1-1, p0, c2, l2-1, c3, c1, c0, a0 },
    keywordstyle=[4]\color{blue}\bfseries,
}

\begin{figure*}
\footnotesize
\begin{lstlisting}[basicstyle=\footnotesize\ttfamily]
Name: logistics-c4-s2-p4-a1 (logistics_a-1_c-4_s-2_p-4_t-4.pddl)
Objects: 
    a0, c0, c1, c2, c3, l0-0, l0-1, l1-0, l1-1, l2-0, l2-1, l3-0, l3-1, p0, p1, p2
p3, t0, t1, t2, t3
Initial: 
    package(p0), package(p1), package(p2), package(p3), truck(t0), truck(t1)
truck(t2), truck(t3), location(l0-0), location(l0-1), location(l1-0)
location(l1-1), location(l2-0), location(l2-1), location(l3-0), location(l3-1)
airplane(a0), city(c0), city(c1), city(c2), city(c3), airport(l0-0)
airport(l1-0), airport(l2-0), airport(l3-0), at(t0, l0-1), at(p0, l0-1), at(p3
l1-0), at(t1, l1-1), at(a0, l2-0), at(t2, l2-0), at(p2, l2-0), at(t3, l3-0)
at(p1, l3-0), in-city(l0-0, c0), in-city(l0-1, c0), in-city(l1-0, c1)
in-city(l1-1, c1), in-city(l2-0, c2), in-city(l2-1, c2), in-city(l3-0, c3)
in-city(l3-1, c3)
Goal: 
    at(p0, l3-1), at(p1, l2-0), at(p2, l1-0), at(p3, l0-0)

Plan has path-cycle: unchecked
Plan has subgoal-cycle: false
Primitive plan: 24
Plan: 12
1  load-truck(p0, t0, l0-1)
2  load-truck(p1, t3, l3-0)
3  drive-truck(t1, l1-1, l1-0, c1) -> load-truck(p3, t1, l1-0)
4  load-airplane(p2, a0, l2-0)
5  fly-airplane(a0, l2-0, l1-0) -> unload-airplane(p2, a0, l1-0)
6  unload-truck(p3, t1, l1-0) -> load-airplane(p3, a0, l1-0)
7  fly-airplane(a0, l1-0, l0-0) -> unload-airplane(p3, a0, l0-0)
8  drive-truck(t0, l0-1, l0-0, c0) -> unload-truck(p0, t0, l0-0) -> load-airplane(p0, a0, l0-0)
9  fly-airplane(a0, l0-0, l3-0) -> unload-airplane(p0, a0, l3-0) -> load-truck(p0, t3, l3-0)
10 drive-truck(t3, l3-0, l3-1, c3) -> unload-truck(p0, t3, l3-1)
11 drive-truck(t3, l3-1, l3-0, c3) -> unload-truck(p1, t3, l3-0) -> load-airplane(p1, a0, l3-0)
12 fly-airplane(a0, l3-0, l2-0) -> unload-airplane(p1, a0, l2-0)
\end{lstlisting}
\end{figure*}

\clearpage

\lstset{
    basicstyle=\footnotesize\ttfamily,
    keywordstyle=\bfseries, % This will apply bold to all keywords
    % Define colors for different groups of keywords
    morekeywords=[1]{Domain},
    keywordstyle=[1]\color{red}\bfseries,
    morekeywords=[2]{Objects, Primitive, Goal, Initial, Plan, plan},
    keywordstyle=[2]\bfseries,
    morekeywords=[3]{UNLOAD, TRUCK, UNLOAD, AIRPLANE, LOAD, TRUCK, FLY, AIRPLANE, DRIVE, TRUCK, LOAD, AIRPLANE },
    keywordstyle=[3]\color{orange}\bfseries,
    morekeywords=[4]{t2, p3, l1-0, l0-1, p2, l3-0, p1, l3-1, t1, t0, l2-0, l0-0, t3, l1-1, p0, c2, l2-1, c3, c1, c0, a0 },
    keywordstyle=[4]\color{blue}\bfseries,
}

\begin{figure*}
\footnotesize
\begin{lstlisting}[basicstyle=\footnotesize\ttfamily]
Name: logistics-c4-s2-p4-a1 (logistics_a-1_c-4_s-2_p-4_t-4.pddl)
Objects: 
    a0, c0, c1, c2, c3, l0-0, l0-1, l1-0, l1-1, l2-0, l2-1, l3-0, l3-1, p0, p1, p2
p3, t0, t1, t2, t3
Initial: 
    package(p0), package(p1), package(p2), package(p3), truck(t0), truck(t1)
truck(t2), truck(t3), location(l0-0), location(l0-1), location(l1-0)
location(l1-1), location(l2-0), location(l2-1), location(l3-0), location(l3-1)
airplane(a0), city(c0), city(c1), city(c2), city(c3), airport(l0-0)
airport(l1-0), airport(l2-0), airport(l3-0), at(t0, l0-1), at(p0, l0-1), at(p3
l1-0), at(t1, l1-1), at(a0, l2-0), at(t2, l2-0), at(p2, l2-0), at(t3, l3-0)
at(p1, l3-0), in-city(l0-0, c0), in-city(l0-1, c0), in-city(l1-0, c1)
in-city(l1-1, c1), in-city(l2-0, c2), in-city(l2-1, c2), in-city(l3-0, c3)
in-city(l3-1, c3)
Goal: 
    at(p0, l3-1), at(p1, l2-0), at(p2, l1-0), at(p3, l0-0)

Plan has path-cycle: unchecked
Plan has subgoal-cycle: false
Primitive plan: 24
Plan: 12
1  load-truck(p0, t0, l0-1)
2  load-truck(p1, t3, l3-0)
3  drive-truck(t1, l1-1, l1-0, c1) -> load-truck(p3, t1, l1-0)
4  load-airplane(p2, a0, l2-0)
5  fly-airplane(a0, l2-0, l1-0) -> unload-airplane(p2, a0, l1-0)
6  unload-truck(p3, t1, l1-0) -> load-airplane(p3, a0, l1-0)
7  fly-airplane(a0, l1-0, l0-0) -> unload-airplane(p3, a0, l0-0)
8  drive-truck(t0, l0-1, l0-0, c0) -> unload-truck(p0, t0, l0-0) -> load-airplane(p0, a0, l0-0)
9  fly-airplane(a0, l0-0, l3-0) -> unload-airplane(p0, a0, l3-0) -> load-truck(p0, t3, l3-0)
10 drive-truck(t3, l3-0, l3-1, c3) -> unload-truck(p0, t3, l3-1)
11 drive-truck(t3, l3-1, l3-0, c3) -> unload-truck(p1, t3, l3-0) -> load-airplane(p1, a0, l3-0)
12 fly-airplane(a0, l3-0, l2-0) -> unload-airplane(p1, a0, l2-0)
\end{lstlisting}
\end{figure*}

\clearpage

\lstset{
    basicstyle=\footnotesize\ttfamily,
    keywordstyle=\bfseries, % This will apply bold to all keywords
    % Define colors for different groups of keywords
    morekeywords=[1]{Domain},
    keywordstyle=[1]\color{red}\bfseries,
    morekeywords=[2]{Objects, Primitive, Goal, Initial, Plan, plan},
    keywordstyle=[2]\bfseries,
    morekeywords=[3]{UNLOAD, TRUCK, UNLOAD, AIRPLANE, LOAD, TRUCK, FLY, AIRPLANE, DRIVE, TRUCK, LOAD, AIRPLANE },
    keywordstyle=[3]\color{orange}\bfseries,
    morekeywords=[4]{t2, p3, l1-0, l0-1, p2, l3-0, p1, l3-1, t1, t0, l2-0, l0-0, t3, l1-1, p0, c2, l2-1, c3, c1, c0, a0 },
    keywordstyle=[4]\color{blue}\bfseries,
}

\begin{figure*}
\footnotesize
\begin{lstlisting}[basicstyle=\footnotesize\ttfamily]
Name: logistics-c4-s2-p4-a1 (logistics_a-1_c-4_s-2_p-4_t-4.pddl)
Objects: 
    a0, c0, c1, c2, c3, l0-0, l0-1, l1-0, l1-1, l2-0, l2-1, l3-0, l3-1, p0, p1, p2
p3, t0, t1, t2, t3
Initial: 
    package(p0), package(p1), package(p2), package(p3), truck(t0), truck(t1)
truck(t2), truck(t3), location(l0-0), location(l0-1), location(l1-0)
location(l1-1), location(l2-0), location(l2-1), location(l3-0), location(l3-1)
airplane(a0), city(c0), city(c1), city(c2), city(c3), airport(l0-0)
airport(l1-0), airport(l2-0), airport(l3-0), at(t0, l0-1), at(p0, l0-1), at(p3
l1-0), at(t1, l1-1), at(a0, l2-0), at(t2, l2-0), at(p2, l2-0), at(t3, l3-0)
at(p1, l3-0), in-city(l0-0, c0), in-city(l0-1, c0), in-city(l1-0, c1)
in-city(l1-1, c1), in-city(l2-0, c2), in-city(l2-1, c2), in-city(l3-0, c3)
in-city(l3-1, c3)
Goal: 
    at(p0, l3-1), at(p1, l2-0), at(p2, l1-0), at(p3, l0-0)

Plan has path-cycle: unchecked
Plan has subgoal-cycle: false
Primitive plan: 24
Plan: 12
1  load-truck(p0, t0, l0-1)
2  load-truck(p1, t3, l3-0)
3  drive-truck(t1, l1-1, l1-0, c1) -> load-truck(p3, t1, l1-0)
4  load-airplane(p2, a0, l2-0)
5  fly-airplane(a0, l2-0, l1-0) -> unload-airplane(p2, a0, l1-0)
6  unload-truck(p3, t1, l1-0) -> load-airplane(p3, a0, l1-0)
7  fly-airplane(a0, l1-0, l0-0) -> unload-airplane(p3, a0, l0-0)
8  drive-truck(t0, l0-1, l0-0, c0) -> unload-truck(p0, t0, l0-0) -> load-airplane(p0, a0, l0-0)
9  fly-airplane(a0, l0-0, l3-0) -> unload-airplane(p0, a0, l3-0) -> load-truck(p0, t3, l3-0)
10 drive-truck(t3, l3-0, l3-1, c3) -> unload-truck(p0, t3, l3-1)
11 drive-truck(t3, l3-1, l3-0, c3) -> unload-truck(p1, t3, l3-0) -> load-airplane(p1, a0, l3-0)
12 fly-airplane(a0, l3-0, l2-0) -> unload-airplane(p1, a0, l2-0)
\end{lstlisting}
\end{figure*}

\clearpage

\lstset{
    basicstyle=\footnotesize\ttfamily,
    keywordstyle=\bfseries, % This will apply bold to all keywords
    % Define colors for different groups of keywords
    morekeywords=[1]{Domain},
    keywordstyle=[1]\color{red}\bfseries,
    morekeywords=[2]{Objects, Primitive, Goal, Initial, Plan, plan},
    keywordstyle=[2]\bfseries,
    morekeywords=[3]{UNLOAD, TRUCK, UNLOAD, AIRPLANE, LOAD, TRUCK, FLY, AIRPLANE, DRIVE, TRUCK, LOAD, AIRPLANE },
    keywordstyle=[3]\color{orange}\bfseries,
    morekeywords=[4]{t2, p3, l1-0, l0-1, p2, l3-0, p5, p1, l3-1, t1, t0, l2-0, l0-0, t3, l1-1, p0, c2, l2-1, p6, c3, p4, c1, c0, a0 },
    keywordstyle=[4]\color{blue}\bfseries,
}

\lstset{
    basicstyle=\footnotesize\ttfamily,
    keywordstyle=\bfseries, % This will apply bold to all keywords
    % Define colors for different groups of keywords
    morekeywords=[1]{Domain},
    keywordstyle=[1]\color{red}\bfseries,
    morekeywords=[2]{Objects, Primitive, Goal, Initial, Plan, plan},
    keywordstyle=[2]\bfseries,
    morekeywords=[3]{UNLOAD, TRUCK, UNLOAD, AIRPLANE, LOAD, TRUCK, FLY, AIRPLANE, DRIVE, TRUCK, LOAD, AIRPLANE },
    keywordstyle=[3]\color{orange}\bfseries,
    morekeywords=[4]{t2, p3, l1-0, l0-1, p2, l3-0, p5, p1, l3-1, t1, t0, l2-0, l0-0, t3, l1-1, p0, c2, l2-1, p6, c3, p4, c1, c0, a0 },
    keywordstyle=[4]\color{blue}\bfseries,
}

\lstset{
    basicstyle=\footnotesize\ttfamily,
    keywordstyle=\bfseries, % This will apply bold to all keywords
    % Define colors for different groups of keywords
    morekeywords=[1]{Domain},
    keywordstyle=[1]\color{red}\bfseries,
    morekeywords=[2]{Objects, Primitive, Goal, Initial, Plan, plan},
    keywordstyle=[2]\bfseries,
    morekeywords=[3]{UNLOAD, TRUCK, UNLOAD, AIRPLANE, LOAD, TRUCK, FLY, AIRPLANE, DRIVE, TRUCK, LOAD, AIRPLANE },
    keywordstyle=[3]\color{orange}\bfseries,
    morekeywords=[4]{t4, t2, l1-0, l4-0, l0-1, l3-0, p1, l3-1, l4-1, t1, t0, c4, l2-0, l0-0, t3, l1-1, p0, c2, l2-1, c3, c1, c0, a0 },
    keywordstyle=[4]\color{blue}\bfseries,
}

\begin{figure*}
\footnotesize
\begin{lstlisting}[basicstyle=\footnotesize\ttfamily]
Name: logistics-c5-s2-p2-a1 (logistics_a-1_c-5_s-2_p-2_t-5.pddl)
Objects: 
    a0, c0, c1, c2, c3, c4, l0-0, l0-1, l1-0, l1-1, l2-0, l2-1, l3-0, l3-1, l4-0
l4-1, p0, p1, t0, t1, t2, t3, t4
Initial: 
    package(p0), package(p1), truck(t0), truck(t1), truck(t2), truck(t3), truck(t4)
location(l0-0), location(l0-1), location(l1-0), location(l1-1), location(l2-0)
location(l2-1), location(l3-0), location(l3-1), location(l4-0), location(l4-1)
airplane(a0), city(c0), city(c1), city(c2), city(c3), city(c4), airport(l0-0)
airport(l1-0), airport(l2-0), airport(l3-0), airport(l4-0), at(t0, l0-1), at(t1
l1-1), at(t2, l2-0), at(a0, l3-0), at(t3, l3-0), at(p0, l3-1), at(t4, l4-0)
at(p1, l4-0), in-city(l0-0, c0), in-city(l0-1, c0), in-city(l1-0, c1)
in-city(l1-1, c1), in-city(l2-0, c2), in-city(l2-1, c2), in-city(l3-0, c3)
in-city(l3-1, c3), in-city(l4-0, c4), in-city(l4-1, c4)
Goal: 
    at(p0, l2-1), at(p1, l0-1)

Plan has path-cycle: unchecked
Plan has subgoal-cycle: false
Primitive plan: 23
Plan: 10
1  drive-truck(t3, l3-0, l3-1, c3) -> load-truck(p0, t3, l3-1)
2  drive-truck(t3, l3-1, l3-0, c3) -> unload-truck(p0, t3, l3-0) -> load-airplane(p0, a0, l3-0)
3  fly-airplane(a0, l3-0, l4-0) -> load-airplane(p1, a0, l4-0)
4  fly-airplane(a0, l4-0, l2-0) -> unload-airplane(p1, a0, l2-0) -> load-truck(p1, t2, l2-0)
5  unload-airplane(p0, a0, l2-0) -> load-truck(p0, t2, l2-0)
6  drive-truck(t2, l2-0, l2-1, c2) -> unload-truck(p0, t2, l2-1)
7  drive-truck(t2, l2-1, l2-0, c2) -> unload-truck(p1, t2, l2-0) -> load-airplane(p1, a0, l2-0)
8  drive-truck(t0, l0-1, l0-0, c0)
9  fly-airplane(a0, l2-0, l0-0) -> unload-airplane(p1, a0, l0-0) -> load-truck(p1, t0, l0-0)
10 drive-truck(t0, l0-0, l0-1, c0) -> unload-truck(p1, t0, l0-1)
\end{lstlisting}
\end{figure*}

\clearpage

\lstset{
    basicstyle=\footnotesize\ttfamily,
    keywordstyle=\bfseries, % This will apply bold to all keywords
    % Define colors for different groups of keywords
    morekeywords=[1]{Domain},
    keywordstyle=[1]\color{red}\bfseries,
    morekeywords=[2]{Objects, Primitive, Goal, Initial, Plan, plan},
    keywordstyle=[2]\bfseries,
    morekeywords=[3]{UNLOAD, TRUCK, UNLOAD, AIRPLANE, LOAD, TRUCK, FLY, AIRPLANE, DRIVE, TRUCK, LOAD, AIRPLANE },
    keywordstyle=[3]\color{orange}\bfseries,
    morekeywords=[4]{t4, t2, l1-0, l4-0, l0-1, l3-0, p1, l3-1, l4-1, t1, t0, c4, l2-0, l0-0, t3, l1-1, p0, c2, l2-1, c3, c1, c0, a0 },
    keywordstyle=[4]\color{blue}\bfseries,
}

\begin{figure*}
\footnotesize
\begin{lstlisting}[basicstyle=\footnotesize\ttfamily]
Name: logistics-c5-s2-p2-a1 (logistics_a-1_c-5_s-2_p-2_t-5.pddl)
Objects: 
    a0, c0, c1, c2, c3, c4, l0-0, l0-1, l1-0, l1-1, l2-0, l2-1, l3-0, l3-1, l4-0
l4-1, p0, p1, t0, t1, t2, t3, t4
Initial: 
    package(p0), package(p1), truck(t0), truck(t1), truck(t2), truck(t3), truck(t4)
location(l0-0), location(l0-1), location(l1-0), location(l1-1), location(l2-0)
location(l2-1), location(l3-0), location(l3-1), location(l4-0), location(l4-1)
airplane(a0), city(c0), city(c1), city(c2), city(c3), city(c4), airport(l0-0)
airport(l1-0), airport(l2-0), airport(l3-0), airport(l4-0), at(t0, l0-1), at(t1
l1-1), at(t2, l2-0), at(a0, l3-0), at(t3, l3-0), at(p0, l3-1), at(t4, l4-0)
at(p1, l4-0), in-city(l0-0, c0), in-city(l0-1, c0), in-city(l1-0, c1)
in-city(l1-1, c1), in-city(l2-0, c2), in-city(l2-1, c2), in-city(l3-0, c3)
in-city(l3-1, c3), in-city(l4-0, c4), in-city(l4-1, c4)
Goal: 
    at(p0, l2-1), at(p1, l0-1)

Plan has path-cycle: unchecked
Plan has subgoal-cycle: false
Primitive plan: 23
Plan: 10
1  drive-truck(t3, l3-0, l3-1, c3) -> load-truck(p0, t3, l3-1)
2  drive-truck(t3, l3-1, l3-0, c3) -> unload-truck(p0, t3, l3-0) -> load-airplane(p0, a0, l3-0)
3  fly-airplane(a0, l3-0, l4-0) -> load-airplane(p1, a0, l4-0)
4  fly-airplane(a0, l4-0, l2-0) -> unload-airplane(p1, a0, l2-0) -> load-truck(p1, t2, l2-0)
5  unload-airplane(p0, a0, l2-0) -> load-truck(p0, t2, l2-0)
6  drive-truck(t2, l2-0, l2-1, c2) -> unload-truck(p0, t2, l2-1)
7  drive-truck(t2, l2-1, l2-0, c2) -> unload-truck(p1, t2, l2-0) -> load-airplane(p1, a0, l2-0)
8  drive-truck(t0, l0-1, l0-0, c0)
9  fly-airplane(a0, l2-0, l0-0) -> unload-airplane(p1, a0, l0-0) -> load-truck(p1, t0, l0-0)
10 drive-truck(t0, l0-0, l0-1, c0) -> unload-truck(p1, t0, l0-1)
\end{lstlisting}
\end{figure*}

\clearpage

\lstset{
    basicstyle=\footnotesize\ttfamily,
    keywordstyle=\bfseries, % This will apply bold to all keywords
    % Define colors for different groups of keywords
    morekeywords=[1]{Domain},
    keywordstyle=[1]\color{red}\bfseries,
    morekeywords=[2]{Objects, Primitive, Goal, Initial, Plan, plan},
    keywordstyle=[2]\bfseries,
    morekeywords=[3]{UNLOAD, TRUCK, UNLOAD, AIRPLANE, LOAD, TRUCK, FLY, AIRPLANE, DRIVE, TRUCK, LOAD, AIRPLANE },
    keywordstyle=[3]\color{orange}\bfseries,
    morekeywords=[4]{t4, t2, l1-0, l4-0, l0-1, l3-0, p1, l3-1, l4-1, t1, t0, c4, l2-0, l0-0, t3, l1-1, p0, c2, l2-1, c3, c1, c0, a0 },
    keywordstyle=[4]\color{blue}\bfseries,
}

\begin{figure*}
\footnotesize
\begin{lstlisting}[basicstyle=\footnotesize\ttfamily]
Name: logistics-c5-s2-p2-a1 (logistics_a-1_c-5_s-2_p-2_t-5.pddl)
Objects: 
    a0, c0, c1, c2, c3, c4, l0-0, l0-1, l1-0, l1-1, l2-0, l2-1, l3-0, l3-1, l4-0
l4-1, p0, p1, t0, t1, t2, t3, t4
Initial: 
    package(p0), package(p1), truck(t0), truck(t1), truck(t2), truck(t3), truck(t4)
location(l0-0), location(l0-1), location(l1-0), location(l1-1), location(l2-0)
location(l2-1), location(l3-0), location(l3-1), location(l4-0), location(l4-1)
airplane(a0), city(c0), city(c1), city(c2), city(c3), city(c4), airport(l0-0)
airport(l1-0), airport(l2-0), airport(l3-0), airport(l4-0), at(t0, l0-1), at(t1
l1-1), at(t2, l2-0), at(a0, l3-0), at(t3, l3-0), at(p0, l3-1), at(t4, l4-0)
at(p1, l4-0), in-city(l0-0, c0), in-city(l0-1, c0), in-city(l1-0, c1)
in-city(l1-1, c1), in-city(l2-0, c2), in-city(l2-1, c2), in-city(l3-0, c3)
in-city(l3-1, c3), in-city(l4-0, c4), in-city(l4-1, c4)
Goal: 
    at(p0, l2-1), at(p1, l0-1)

Plan has path-cycle: unchecked
Plan has subgoal-cycle: false
Primitive plan: 23
Plan: 10
1  drive-truck(t3, l3-0, l3-1, c3) -> load-truck(p0, t3, l3-1)
2  drive-truck(t3, l3-1, l3-0, c3) -> unload-truck(p0, t3, l3-0) -> load-airplane(p0, a0, l3-0)
3  fly-airplane(a0, l3-0, l4-0) -> load-airplane(p1, a0, l4-0)
4  fly-airplane(a0, l4-0, l2-0) -> unload-airplane(p1, a0, l2-0) -> load-truck(p1, t2, l2-0)
5  unload-airplane(p0, a0, l2-0) -> load-truck(p0, t2, l2-0)
6  drive-truck(t2, l2-0, l2-1, c2) -> unload-truck(p0, t2, l2-1)
7  drive-truck(t2, l2-1, l2-0, c2) -> unload-truck(p1, t2, l2-0) -> load-airplane(p1, a0, l2-0)
8  drive-truck(t0, l0-1, l0-0, c0)
9  fly-airplane(a0, l2-0, l0-0) -> unload-airplane(p1, a0, l0-0) -> load-truck(p1, t0, l0-0)
10 drive-truck(t0, l0-0, l0-1, c0) -> unload-truck(p1, t0, l0-1)
\end{lstlisting}
\end{figure*}

\clearpage

\lstset{
    basicstyle=\footnotesize\ttfamily,
    keywordstyle=\bfseries, % This will apply bold to all keywords
    % Define colors for different groups of keywords
    morekeywords=[1]{Domain},
    keywordstyle=[1]\color{red}\bfseries,
    morekeywords=[2]{Objects, Primitive, Goal, Initial, Plan, plan},
    keywordstyle=[2]\bfseries,
    morekeywords=[3]{UNLOAD, TRUCK, UNLOAD, AIRPLANE, LOAD, TRUCK, FLY, AIRPLANE, DRIVE, TRUCK, LOAD, AIRPLANE },
    keywordstyle=[3]\color{orange}\bfseries,
    morekeywords=[4]{t4, t2, l1-0, l4-0, l0-1, l3-0, p1, l3-1, l4-1, t1, t0, c4, l2-0, l0-0, t3, l1-1, p0, c2, l2-1, c3, c1, c0, a0 },
    keywordstyle=[4]\color{blue}\bfseries,
}

\begin{figure*}
\footnotesize
\begin{lstlisting}[basicstyle=\footnotesize\ttfamily]
Name: logistics-c5-s2-p2-a1 (logistics_a-1_c-5_s-2_p-2_t-5.pddl)
Objects: 
    a0, c0, c1, c2, c3, c4, l0-0, l0-1, l1-0, l1-1, l2-0, l2-1, l3-0, l3-1, l4-0
l4-1, p0, p1, t0, t1, t2, t3, t4
Initial: 
    package(p0), package(p1), truck(t0), truck(t1), truck(t2), truck(t3), truck(t4)
location(l0-0), location(l0-1), location(l1-0), location(l1-1), location(l2-0)
location(l2-1), location(l3-0), location(l3-1), location(l4-0), location(l4-1)
airplane(a0), city(c0), city(c1), city(c2), city(c3), city(c4), airport(l0-0)
airport(l1-0), airport(l2-0), airport(l3-0), airport(l4-0), at(t0, l0-1), at(t1
l1-1), at(t2, l2-0), at(a0, l3-0), at(t3, l3-0), at(p0, l3-1), at(t4, l4-0)
at(p1, l4-0), in-city(l0-0, c0), in-city(l0-1, c0), in-city(l1-0, c1)
in-city(l1-1, c1), in-city(l2-0, c2), in-city(l2-1, c2), in-city(l3-0, c3)
in-city(l3-1, c3), in-city(l4-0, c4), in-city(l4-1, c4)
Goal: 
    at(p0, l2-1), at(p1, l0-1)

Plan has path-cycle: unchecked
Plan has subgoal-cycle: false
Primitive plan: 23
Plan: 10
1  drive-truck(t3, l3-0, l3-1, c3) -> load-truck(p0, t3, l3-1)
2  drive-truck(t3, l3-1, l3-0, c3) -> unload-truck(p0, t3, l3-0) -> load-airplane(p0, a0, l3-0)
3  fly-airplane(a0, l3-0, l4-0) -> load-airplane(p1, a0, l4-0)
4  fly-airplane(a0, l4-0, l2-0) -> unload-airplane(p1, a0, l2-0) -> load-truck(p1, t2, l2-0)
5  unload-airplane(p0, a0, l2-0) -> load-truck(p0, t2, l2-0)
6  drive-truck(t2, l2-0, l2-1, c2) -> unload-truck(p0, t2, l2-1)
7  drive-truck(t2, l2-1, l2-0, c2) -> unload-truck(p1, t2, l2-0) -> load-airplane(p1, a0, l2-0)
8  drive-truck(t0, l0-1, l0-0, c0)
9  fly-airplane(a0, l2-0, l0-0) -> unload-airplane(p1, a0, l0-0) -> load-truck(p1, t0, l0-0)
10 drive-truck(t0, l0-0, l0-1, c0) -> unload-truck(p1, t0, l0-1)
\end{lstlisting}
\end{figure*}

\clearpage

\lstset{
    basicstyle=\footnotesize\ttfamily,
    keywordstyle=\bfseries, % This will apply bold to all keywords
    % Define colors for different groups of keywords
    morekeywords=[1]{Domain},
    keywordstyle=[1]\color{red}\bfseries,
    morekeywords=[2]{Objects, Primitive, Goal, Initial, Plan, plan},
    keywordstyle=[2]\bfseries,
    morekeywords=[3]{UNLOAD, TRUCK, UNLOAD, AIRPLANE, LOAD, TRUCK, FLY, AIRPLANE, DRIVE, TRUCK, LOAD, AIRPLANE },
    keywordstyle=[3]\color{orange}\bfseries,
    morekeywords=[4]{t4, t2, p3, l1-0, l4-0, l0-1, p2, l3-0, p1, l3-1, l4-1, t1, t0, c4, l2-0, l0-0, t3, l1-1, p0, c2, l2-1, c3, p4, c1, c0, a0 },
    keywordstyle=[4]\color{blue}\bfseries,
}

\begin{figure*}
\footnotesize
\begin{lstlisting}[basicstyle=\footnotesize\ttfamily]
Name: logistics-c5-s2-p5-a1 (logistics_a-1_c-5_s-2_p-5_t-5.pddl)
Objects: 
    a0, c0, c1, c2, c3, c4, l0-0, l0-1, l1-0, l1-1, l2-0, l2-1, l3-0, l3-1, l4-0
l4-1, p0, p1, p2, p3, p4, t0, t1, t2, t3, t4
Initial: 
    package(p0), package(p1), package(p2), package(p3), package(p4), truck(t0)
truck(t1), truck(t2), truck(t3), truck(t4), location(l0-0), location(l0-1)
location(l1-0), location(l1-1), location(l2-0), location(l2-1), location(l3-0)
location(l3-1), location(l4-0), location(l4-1), airplane(a0), city(c0), city(c1)
city(c2), city(c3), city(c4), airport(l0-0), airport(l1-0), airport(l2-0)
airport(l3-0), airport(l4-0), at(t0, l0-1), at(p3, l0-1), at(t1, l1-1), at(t2
l2-0), at(p2, l2-1), at(t3, l3-0), at(p4, l3-0), at(p0, l3-1), at(a0, l4-0)
at(t4, l4-0), at(p1, l4-0), in-city(l0-0, c0), in-city(l0-1, c0), in-city(l1-0
c1), in-city(l1-1, c1), in-city(l2-0, c2), in-city(l2-1, c2), in-city(l3-0, c3)
in-city(l3-1, c3), in-city(l4-0, c4), in-city(l4-1, c4)
Goal: 
    at(p0, l3-1), at(p1, l2-0), at(p2, l0-0), at(p3, l0-1), at(p4, l3-0)

Plan has path-cycle: unchecked
Plan has subgoal-cycle: false
Primitive plan: 10
Plan: 5
1 drive-truck(t2, l2-0, l2-1, c2) -> load-truck(p2, t2, l2-1)
2 load-airplane(p1, a0, l4-0)
3 fly-airplane(a0, l4-0, l2-0) -> unload-airplane(p1, a0, l2-0)
4 drive-truck(t2, l2-1, l2-0, c2) -> unload-truck(p2, t2, l2-0) -> load-airplane(p2, a0, l2-0)
5 fly-airplane(a0, l2-0, l0-0) -> unload-airplane(p2, a0, l0-0)
\end{lstlisting}
\end{figure*}

\clearpage

\lstset{
    basicstyle=\footnotesize\ttfamily,
    keywordstyle=\bfseries, % This will apply bold to all keywords
    % Define colors for different groups of keywords
    morekeywords=[1]{Domain},
    keywordstyle=[1]\color{red}\bfseries,
    morekeywords=[2]{Objects, Primitive, Goal, Initial, Plan, plan},
    keywordstyle=[2]\bfseries,
    morekeywords=[3]{UNLOAD, TRUCK, UNLOAD, AIRPLANE, LOAD, TRUCK, FLY, AIRPLANE, DRIVE, TRUCK, LOAD, AIRPLANE },
    keywordstyle=[3]\color{orange}\bfseries,
    morekeywords=[4]{t4, t2, p3, l1-0, l4-0, l0-1, p2, l3-0, p1, l3-1, l4-1, t1, t0, c4, l2-0, l0-0, t3, l1-1, p0, c2, l2-1, c3, p4, c1, c0, a0 },
    keywordstyle=[4]\color{blue}\bfseries,
}

\begin{figure*}
\footnotesize
\begin{lstlisting}[basicstyle=\footnotesize\ttfamily]
Name: logistics-c5-s2-p5-a1 (logistics_a-1_c-5_s-2_p-5_t-5.pddl)
Objects: 
    a0, c0, c1, c2, c3, c4, l0-0, l0-1, l1-0, l1-1, l2-0, l2-1, l3-0, l3-1, l4-0
l4-1, p0, p1, p2, p3, p4, t0, t1, t2, t3, t4
Initial: 
    package(p0), package(p1), package(p2), package(p3), package(p4), truck(t0)
truck(t1), truck(t2), truck(t3), truck(t4), location(l0-0), location(l0-1)
location(l1-0), location(l1-1), location(l2-0), location(l2-1), location(l3-0)
location(l3-1), location(l4-0), location(l4-1), airplane(a0), city(c0), city(c1)
city(c2), city(c3), city(c4), airport(l0-0), airport(l1-0), airport(l2-0)
airport(l3-0), airport(l4-0), at(t0, l0-1), at(p3, l0-1), at(t1, l1-1), at(t2
l2-0), at(p2, l2-1), at(t3, l3-0), at(p4, l3-0), at(p0, l3-1), at(a0, l4-0)
at(t4, l4-0), at(p1, l4-0), in-city(l0-0, c0), in-city(l0-1, c0), in-city(l1-0
c1), in-city(l1-1, c1), in-city(l2-0, c2), in-city(l2-1, c2), in-city(l3-0, c3)
in-city(l3-1, c3), in-city(l4-0, c4), in-city(l4-1, c4)
Goal: 
    at(p0, l3-1), at(p1, l2-0), at(p2, l0-0), at(p3, l0-1), at(p4, l3-0)

Plan has path-cycle: unchecked
Plan has subgoal-cycle: false
Primitive plan: 10
Plan: 5
1 drive-truck(t2, l2-0, l2-1, c2) -> load-truck(p2, t2, l2-1)
2 load-airplane(p1, a0, l4-0)
3 fly-airplane(a0, l4-0, l2-0) -> unload-airplane(p1, a0, l2-0)
4 drive-truck(t2, l2-1, l2-0, c2) -> unload-truck(p2, t2, l2-0) -> load-airplane(p2, a0, l2-0)
5 fly-airplane(a0, l2-0, l0-0) -> unload-airplane(p2, a0, l0-0)
\end{lstlisting}
\end{figure*}

\clearpage

\lstset{
    basicstyle=\footnotesize\ttfamily,
    keywordstyle=\bfseries, % This will apply bold to all keywords
    % Define colors for different groups of keywords
    morekeywords=[1]{Domain},
    keywordstyle=[1]\color{red}\bfseries,
    morekeywords=[2]{Objects, Primitive, Goal, Initial, Plan, plan},
    keywordstyle=[2]\bfseries,
    morekeywords=[3]{UNLOAD, TRUCK, UNLOAD, AIRPLANE, LOAD, TRUCK, FLY, AIRPLANE, DRIVE, TRUCK, LOAD, AIRPLANE },
    keywordstyle=[3]\color{orange}\bfseries,
    morekeywords=[4]{t4, t2, p3, l1-0, l4-0, l0-1, p2, l3-0, p1, l3-1, l4-1, t1, t0, c4, l2-0, l0-0, t3, l1-1, p0, c2, l2-1, c3, p4, c1, c0, a0 },
    keywordstyle=[4]\color{blue}\bfseries,
}

\begin{figure*}
\footnotesize
\begin{lstlisting}[basicstyle=\footnotesize\ttfamily]
Name: logistics-c5-s2-p5-a1 (logistics_a-1_c-5_s-2_p-5_t-5.pddl)
Objects: 
    a0, c0, c1, c2, c3, c4, l0-0, l0-1, l1-0, l1-1, l2-0, l2-1, l3-0, l3-1, l4-0
l4-1, p0, p1, p2, p3, p4, t0, t1, t2, t3, t4
Initial: 
    package(p0), package(p1), package(p2), package(p3), package(p4), truck(t0)
truck(t1), truck(t2), truck(t3), truck(t4), location(l0-0), location(l0-1)
location(l1-0), location(l1-1), location(l2-0), location(l2-1), location(l3-0)
location(l3-1), location(l4-0), location(l4-1), airplane(a0), city(c0), city(c1)
city(c2), city(c3), city(c4), airport(l0-0), airport(l1-0), airport(l2-0)
airport(l3-0), airport(l4-0), at(t0, l0-1), at(p3, l0-1), at(t1, l1-1), at(t2
l2-0), at(p2, l2-1), at(t3, l3-0), at(p4, l3-0), at(p0, l3-1), at(a0, l4-0)
at(t4, l4-0), at(p1, l4-0), in-city(l0-0, c0), in-city(l0-1, c0), in-city(l1-0
c1), in-city(l1-1, c1), in-city(l2-0, c2), in-city(l2-1, c2), in-city(l3-0, c3)
in-city(l3-1, c3), in-city(l4-0, c4), in-city(l4-1, c4)
Goal: 
    at(p0, l3-1), at(p1, l2-0), at(p2, l0-0), at(p3, l0-1), at(p4, l3-0)

Plan has path-cycle: unchecked
Plan has subgoal-cycle: false
Primitive plan: 10
Plan: 5
1 drive-truck(t2, l2-0, l2-1, c2) -> load-truck(p2, t2, l2-1)
2 load-airplane(p1, a0, l4-0)
3 fly-airplane(a0, l4-0, l2-0) -> unload-airplane(p1, a0, l2-0)
4 drive-truck(t2, l2-1, l2-0, c2) -> unload-truck(p2, t2, l2-0) -> load-airplane(p2, a0, l2-0)
5 fly-airplane(a0, l2-0, l0-0) -> unload-airplane(p2, a0, l0-0)
\end{lstlisting}
\end{figure*}

\clearpage

\lstset{
    basicstyle=\footnotesize\ttfamily,
    keywordstyle=\bfseries, % This will apply bold to all keywords
    % Define colors for different groups of keywords
    morekeywords=[1]{Domain},
    keywordstyle=[1]\color{red}\bfseries,
    morekeywords=[2]{Objects, Primitive, Goal, Initial, Plan, plan},
    keywordstyle=[2]\bfseries,
    morekeywords=[3]{UNLOAD, TRUCK, UNLOAD, AIRPLANE, LOAD, TRUCK, FLY, AIRPLANE, DRIVE, TRUCK, LOAD, AIRPLANE },
    keywordstyle=[3]\color{orange}\bfseries,
    morekeywords=[4]{t4, t2, p3, l1-0, l4-0, l0-1, p2, l3-0, p1, l3-1, l4-1, t1, t0, c4, l2-0, l0-0, t3, l1-1, p0, c2, l2-1, c3, p4, c1, c0, a0 },
    keywordstyle=[4]\color{blue}\bfseries,
}

\begin{figure*}
\footnotesize
\begin{lstlisting}[basicstyle=\footnotesize\ttfamily]
Name: logistics-c5-s2-p5-a1 (logistics_a-1_c-5_s-2_p-5_t-5.pddl)
Objects: 
    a0, c0, c1, c2, c3, c4, l0-0, l0-1, l1-0, l1-1, l2-0, l2-1, l3-0, l3-1, l4-0
l4-1, p0, p1, p2, p3, p4, t0, t1, t2, t3, t4
Initial: 
    package(p0), package(p1), package(p2), package(p3), package(p4), truck(t0)
truck(t1), truck(t2), truck(t3), truck(t4), location(l0-0), location(l0-1)
location(l1-0), location(l1-1), location(l2-0), location(l2-1), location(l3-0)
location(l3-1), location(l4-0), location(l4-1), airplane(a0), city(c0), city(c1)
city(c2), city(c3), city(c4), airport(l0-0), airport(l1-0), airport(l2-0)
airport(l3-0), airport(l4-0), at(t0, l0-1), at(p3, l0-1), at(t1, l1-1), at(t2
l2-0), at(p2, l2-1), at(t3, l3-0), at(p4, l3-0), at(p0, l3-1), at(a0, l4-0)
at(t4, l4-0), at(p1, l4-0), in-city(l0-0, c0), in-city(l0-1, c0), in-city(l1-0
c1), in-city(l1-1, c1), in-city(l2-0, c2), in-city(l2-1, c2), in-city(l3-0, c3)
in-city(l3-1, c3), in-city(l4-0, c4), in-city(l4-1, c4)
Goal: 
    at(p0, l3-1), at(p1, l2-0), at(p2, l0-0), at(p3, l0-1), at(p4, l3-0)

Plan has path-cycle: unchecked
Plan has subgoal-cycle: false
Primitive plan: 10
Plan: 5
1 drive-truck(t2, l2-0, l2-1, c2) -> load-truck(p2, t2, l2-1)
2 load-airplane(p1, a0, l4-0)
3 fly-airplane(a0, l4-0, l2-0) -> unload-airplane(p1, a0, l2-0)
4 drive-truck(t2, l2-1, l2-0, c2) -> unload-truck(p2, t2, l2-0) -> load-airplane(p2, a0, l2-0)
5 fly-airplane(a0, l2-0, l0-0) -> unload-airplane(p2, a0, l0-0)
\end{lstlisting}
\end{figure*}

\clearpage

\lstset{
    basicstyle=\footnotesize\ttfamily,
    keywordstyle=\bfseries, % This will apply bold to all keywords
    % Define colors for different groups of keywords
    morekeywords=[1]{Domain},
    keywordstyle=[1]\color{red}\bfseries,
    morekeywords=[2]{Objects, Primitive, Goal, Initial, Plan, plan},
    keywordstyle=[2]\bfseries,
    morekeywords=[3]{UNLOAD, TRUCK, UNLOAD, AIRPLANE, LOAD, TRUCK, FLY, AIRPLANE, DRIVE, TRUCK, LOAD, AIRPLANE },
    keywordstyle=[3]\color{orange}\bfseries,
    morekeywords=[4]{p2, p0, t0, p3, p6, p4, p5, l0-0, l0-1, c0, p1, p7, a1, a0 },
    keywordstyle=[4]\color{blue}\bfseries,
}

\begin{figure*}
\footnotesize
\begin{lstlisting}[basicstyle=\footnotesize\ttfamily]
Name: logistics-c1-s2-p8-a2 (logistics_a-2_c-1_s-2_p-8_t-1.pddl)
Objects: 
    a0, a1, c0, l0-0, l0-1, p0, p1, p2, p3, p4, p5, p6, p7, t0
Initial: 
    package(p0), package(p1), package(p2), package(p3), package(p4), package(p5)
package(p6), package(p7), truck(t0), location(l0-0), location(l0-1)
airplane(a0), airplane(a1), city(c0), airport(l0-0), at(a0, l0-0), at(a1, l0-0)
at(p0, l0-0), at(p1, l0-0), at(p3, l0-0), at(p6, l0-0), at(t0, l0-1), at(p2
l0-1), at(p4, l0-1), at(p5, l0-1), at(p7, l0-1), in-city(l0-0, c0), in-city(l0-1
c0)
Goal: 
    at(p0, l0-0), at(p1, l0-0), at(p2, l0-1), at(p3, l0-0), at(p4, l0-1), at(p5
l0-1), at(p6, l0-1), at(p7, l0-1)

Plan has path-cycle: unchecked
Plan has subgoal-cycle: false
Primitive plan: 4
Plan: 2
1 drive-truck(t0, l0-1, l0-0, c0) -> load-truck(p6, t0, l0-0)
2 drive-truck(t0, l0-0, l0-1, c0) -> unload-truck(p6, t0, l0-1)
\end{lstlisting}
\end{figure*}

\clearpage

\lstset{
    basicstyle=\footnotesize\ttfamily,
    keywordstyle=\bfseries, % This will apply bold to all keywords
    % Define colors for different groups of keywords
    morekeywords=[1]{Domain},
    keywordstyle=[1]\color{red}\bfseries,
    morekeywords=[2]{Objects, Primitive, Goal, Initial, Plan, plan},
    keywordstyle=[2]\bfseries,
    morekeywords=[3]{UNLOAD, TRUCK, UNLOAD, AIRPLANE, LOAD, TRUCK, FLY, AIRPLANE, DRIVE, TRUCK, LOAD, AIRPLANE },
    keywordstyle=[3]\color{orange}\bfseries,
    morekeywords=[4]{p2, p0, t0, p3, p6, p4, p5, l0-0, l0-1, c0, p1, p7, a1, a0 },
    keywordstyle=[4]\color{blue}\bfseries,
}

\begin{figure*}
\footnotesize
\begin{lstlisting}[basicstyle=\footnotesize\ttfamily]
Name: logistics-c1-s2-p8-a2 (logistics_a-2_c-1_s-2_p-8_t-1.pddl)
Objects: 
    a0, a1, c0, l0-0, l0-1, p0, p1, p2, p3, p4, p5, p6, p7, t0
Initial: 
    package(p0), package(p1), package(p2), package(p3), package(p4), package(p5)
package(p6), package(p7), truck(t0), location(l0-0), location(l0-1)
airplane(a0), airplane(a1), city(c0), airport(l0-0), at(a0, l0-0), at(a1, l0-0)
at(p0, l0-0), at(p1, l0-0), at(p3, l0-0), at(p6, l0-0), at(t0, l0-1), at(p2
l0-1), at(p4, l0-1), at(p5, l0-1), at(p7, l0-1), in-city(l0-0, c0), in-city(l0-1
c0)
Goal: 
    at(p0, l0-0), at(p1, l0-0), at(p2, l0-1), at(p3, l0-0), at(p4, l0-1), at(p5
l0-1), at(p6, l0-1), at(p7, l0-1)

Plan has path-cycle: unchecked
Plan has subgoal-cycle: false
Primitive plan: 4
Plan: 2
1 drive-truck(t0, l0-1, l0-0, c0) -> load-truck(p6, t0, l0-0)
2 drive-truck(t0, l0-0, l0-1, c0) -> unload-truck(p6, t0, l0-1)
\end{lstlisting}
\end{figure*}

\clearpage

\lstset{
    basicstyle=\footnotesize\ttfamily,
    keywordstyle=\bfseries, % This will apply bold to all keywords
    % Define colors for different groups of keywords
    morekeywords=[1]{Domain},
    keywordstyle=[1]\color{red}\bfseries,
    morekeywords=[2]{Objects, Primitive, Goal, Initial, Plan, plan},
    keywordstyle=[2]\bfseries,
    morekeywords=[3]{UNLOAD, TRUCK, UNLOAD, AIRPLANE, LOAD, TRUCK, FLY, AIRPLANE, DRIVE, TRUCK, LOAD, AIRPLANE },
    keywordstyle=[3]\color{orange}\bfseries,
    morekeywords=[4]{p2, p0, t0, p3, p6, p4, p5, l0-0, l0-1, c0, p1, p7, a1, a0 },
    keywordstyle=[4]\color{blue}\bfseries,
}

\begin{figure*}
\footnotesize
\begin{lstlisting}[basicstyle=\footnotesize\ttfamily]
Name: logistics-c1-s2-p8-a2 (logistics_a-2_c-1_s-2_p-8_t-1.pddl)
Objects: 
    a0, a1, c0, l0-0, l0-1, p0, p1, p2, p3, p4, p5, p6, p7, t0
Initial: 
    package(p0), package(p1), package(p2), package(p3), package(p4), package(p5)
package(p6), package(p7), truck(t0), location(l0-0), location(l0-1)
airplane(a0), airplane(a1), city(c0), airport(l0-0), at(a0, l0-0), at(a1, l0-0)
at(p0, l0-0), at(p1, l0-0), at(p3, l0-0), at(p6, l0-0), at(t0, l0-1), at(p2
l0-1), at(p4, l0-1), at(p5, l0-1), at(p7, l0-1), in-city(l0-0, c0), in-city(l0-1
c0)
Goal: 
    at(p0, l0-0), at(p1, l0-0), at(p2, l0-1), at(p3, l0-0), at(p4, l0-1), at(p5
l0-1), at(p6, l0-1), at(p7, l0-1)

Plan has path-cycle: unchecked
Plan has subgoal-cycle: false
Primitive plan: 4
Plan: 2
1 drive-truck(t0, l0-1, l0-0, c0) -> load-truck(p6, t0, l0-0)
2 drive-truck(t0, l0-0, l0-1, c0) -> unload-truck(p6, t0, l0-1)
\end{lstlisting}
\end{figure*}

\clearpage

\lstset{
    basicstyle=\footnotesize\ttfamily,
    keywordstyle=\bfseries, % This will apply bold to all keywords
    % Define colors for different groups of keywords
    morekeywords=[1]{Domain},
    keywordstyle=[1]\color{red}\bfseries,
    morekeywords=[2]{Objects, Primitive, Goal, Initial, Plan, plan},
    keywordstyle=[2]\bfseries,
    morekeywords=[3]{UNLOAD, TRUCK, UNLOAD, AIRPLANE, LOAD, TRUCK, FLY, AIRPLANE, DRIVE, TRUCK, LOAD, AIRPLANE },
    keywordstyle=[3]\color{orange}\bfseries,
    morekeywords=[4]{p2, p0, t0, p3, p6, p4, p5, l0-0, l0-1, c0, p1, p7, a1, a0 },
    keywordstyle=[4]\color{blue}\bfseries,
}

\begin{figure*}
\footnotesize
\begin{lstlisting}[basicstyle=\footnotesize\ttfamily]
Name: logistics-c1-s2-p8-a2 (logistics_a-2_c-1_s-2_p-8_t-1.pddl)
Objects: 
    a0, a1, c0, l0-0, l0-1, p0, p1, p2, p3, p4, p5, p6, p7, t0
Initial: 
    package(p0), package(p1), package(p2), package(p3), package(p4), package(p5)
package(p6), package(p7), truck(t0), location(l0-0), location(l0-1)
airplane(a0), airplane(a1), city(c0), airport(l0-0), at(a0, l0-0), at(a1, l0-0)
at(p0, l0-0), at(p1, l0-0), at(p3, l0-0), at(p6, l0-0), at(t0, l0-1), at(p2
l0-1), at(p4, l0-1), at(p5, l0-1), at(p7, l0-1), in-city(l0-0, c0), in-city(l0-1
c0)
Goal: 
    at(p0, l0-0), at(p1, l0-0), at(p2, l0-1), at(p3, l0-0), at(p4, l0-1), at(p5
l0-1), at(p6, l0-1), at(p7, l0-1)

Plan has path-cycle: unchecked
Plan has subgoal-cycle: false
Primitive plan: 4
Plan: 2
1 drive-truck(t0, l0-1, l0-0, c0) -> load-truck(p6, t0, l0-0)
2 drive-truck(t0, l0-0, l0-1, c0) -> unload-truck(p6, t0, l0-1)
\end{lstlisting}
\end{figure*}

\clearpage

\lstset{
    basicstyle=\footnotesize\ttfamily,
    keywordstyle=\bfseries, % This will apply bold to all keywords
    % Define colors for different groups of keywords
    morekeywords=[1]{Domain},
    keywordstyle=[1]\color{red}\bfseries,
    morekeywords=[2]{Objects, Primitive, Goal, Initial, Plan, plan},
    keywordstyle=[2]\bfseries,
    morekeywords=[3]{UNLOAD, TRUCK, UNLOAD, AIRPLANE, LOAD, TRUCK, FLY, AIRPLANE, DRIVE, TRUCK, LOAD, AIRPLANE },
    keywordstyle=[3]\color{orange}\bfseries,
    morekeywords=[4]{p2, t1, l1-1, t0, p0, p3, l1-0, p4, l0-0, c1, l0-1, c0, p1, a1, a0 },
    keywordstyle=[4]\color{blue}\bfseries,
}

\begin{figure*}
\footnotesize
\begin{lstlisting}[basicstyle=\footnotesize\ttfamily]
Name: logistics-c2-s2-p5-a2 (logistics_a-2_c-2_s-2_p-5_t-2.pddl)
Objects: 
    a0, a1, c0, c1, l0-0, l0-1, l1-0, l1-1, p0, p1, p2, p3, p4, t0, t1
Initial: 
    package(p0), package(p1), package(p2), package(p3), package(p4), truck(t0)
truck(t1), location(l0-0), location(l0-1), location(l1-0), location(l1-1)
airplane(a0), airplane(a1), city(c0), city(c1), airport(l0-0), airport(l1-0)
at(p0, l0-0), at(p3, l0-0), at(t0, l0-1), at(p1, l0-1), at(a0, l1-0), at(a1
l1-0), at(p2, l1-0), at(p4, l1-0), at(t1, l1-1), in-city(l0-0, c0), in-city(l0-1
c0), in-city(l1-0, c1), in-city(l1-1, c1)
Goal: 
    at(p0, l1-1), at(p1, l0-0), at(p2, l1-0), at(p3, l0-0), at(p4, l0-0)

Plan has path-cycle: unchecked
Plan has subgoal-cycle: false
Primitive plan: 39
Plan: 27
1  load-truck(p1, t0, l0-1)
2  drive-truck(t1, l1-1, l1-0, c1) -> load-truck(p4, t1, l1-0)
3  drive-truck(t0, l0-1, l0-0, c0) -> unload-truck(p1, t0, l0-0)
4  load-truck(p0, t0, l0-0)
5  drive-truck(t0, l0-0, l0-1, c0)
6  drive-truck(t1, l1-0, l1-1, c1)
7  fly-airplane(a1, l1-0, l0-0)
8  fly-airplane(a0, l1-0, l0-0)
9  fly-airplane(a1, l0-0, l1-0)
10 drive-truck(t1, l1-1, l1-0, c1)
11 fly-airplane(a1, l1-0, l0-0)
12 fly-airplane(a0, l0-0, l1-0)
13 drive-truck(t0, l0-1, l0-0, c0)
14 drive-truck(t1, l1-0, l1-1, c1)
15 fly-airplane(a0, l1-0, l0-0)
16 unload-truck(p0, t0, l0-0) -> load-airplane(p0, a1, l0-0)
17 drive-truck(t0, l0-0, l0-1, c0)
18 unload-airplane(p0, a1, l0-0) -> load-airplane(p0, a0, l0-0)
19 drive-truck(t0, l0-1, l0-0, c0)
20 fly-airplane(a1, l0-0, l1-0)
21 unload-airplane(p0, a0, l0-0) -> load-truck(p0, t0, l0-0)
22 fly-airplane(a0, l0-0, l1-0)
23 drive-truck(t1, l1-1, l1-0, c1) -> unload-truck(p4, t1, l1-0) -> load-airplane(p4, a1, l1-0)
24 fly-airplane(a1, l1-0, l0-0) -> unload-airplane(p4, a1, l0-0)
25 unload-truck(p0, t0, l0-0) -> load-airplane(p0, a1, l0-0)
26 fly-airplane(a1, l0-0, l1-0) -> unload-airplane(p0, a1, l1-0) -> load-truck(p0, t1, l1-0)
27 drive-truck(t1, l1-0, l1-1, c1) -> unload-truck(p0, t1, l1-1)
\end{lstlisting}
\end{figure*}

\clearpage

\lstset{
    basicstyle=\footnotesize\ttfamily,
    keywordstyle=\bfseries, % This will apply bold to all keywords
    % Define colors for different groups of keywords
    morekeywords=[1]{Domain},
    keywordstyle=[1]\color{red}\bfseries,
    morekeywords=[2]{Objects, Primitive, Goal, Initial, Plan, plan},
    keywordstyle=[2]\bfseries,
    morekeywords=[3]{UNLOAD, TRUCK, UNLOAD, AIRPLANE, LOAD, TRUCK, FLY, AIRPLANE, DRIVE, TRUCK, LOAD, AIRPLANE },
    keywordstyle=[3]\color{orange}\bfseries,
    morekeywords=[4]{p2, t1, l1-1, t0, p0, p3, l1-0, p4, l0-0, c1, l0-1, c0, p1, a1, a0 },
    keywordstyle=[4]\color{blue}\bfseries,
}

\begin{figure*}
\footnotesize
\begin{lstlisting}[basicstyle=\footnotesize\ttfamily]
Name: logistics-c2-s2-p5-a2 (logistics_a-2_c-2_s-2_p-5_t-2.pddl)
Objects: 
    a0, a1, c0, c1, l0-0, l0-1, l1-0, l1-1, p0, p1, p2, p3, p4, t0, t1
Initial: 
    package(p0), package(p1), package(p2), package(p3), package(p4), truck(t0)
truck(t1), location(l0-0), location(l0-1), location(l1-0), location(l1-1)
airplane(a0), airplane(a1), city(c0), city(c1), airport(l0-0), airport(l1-0)
at(p0, l0-0), at(p3, l0-0), at(t0, l0-1), at(p1, l0-1), at(a0, l1-0), at(a1
l1-0), at(p2, l1-0), at(p4, l1-0), at(t1, l1-1), in-city(l0-0, c0), in-city(l0-1
c0), in-city(l1-0, c1), in-city(l1-1, c1)
Goal: 
    at(p0, l1-1), at(p1, l0-0), at(p2, l1-0), at(p3, l0-0), at(p4, l0-0)

Plan has path-cycle: unchecked
Plan has subgoal-cycle: false
Primitive plan: 39
Plan: 27
1  load-truck(p1, t0, l0-1)
2  drive-truck(t1, l1-1, l1-0, c1) -> load-truck(p4, t1, l1-0)
3  drive-truck(t0, l0-1, l0-0, c0) -> unload-truck(p1, t0, l0-0)
4  load-truck(p0, t0, l0-0)
5  drive-truck(t0, l0-0, l0-1, c0)
6  drive-truck(t1, l1-0, l1-1, c1)
7  fly-airplane(a1, l1-0, l0-0)
8  fly-airplane(a0, l1-0, l0-0)
9  fly-airplane(a1, l0-0, l1-0)
10 drive-truck(t1, l1-1, l1-0, c1)
11 fly-airplane(a1, l1-0, l0-0)
12 fly-airplane(a0, l0-0, l1-0)
13 drive-truck(t0, l0-1, l0-0, c0)
14 drive-truck(t1, l1-0, l1-1, c1)
15 fly-airplane(a0, l1-0, l0-0)
16 unload-truck(p0, t0, l0-0) -> load-airplane(p0, a1, l0-0)
17 drive-truck(t0, l0-0, l0-1, c0)
18 unload-airplane(p0, a1, l0-0) -> load-airplane(p0, a0, l0-0)
19 drive-truck(t0, l0-1, l0-0, c0)
20 fly-airplane(a1, l0-0, l1-0)
21 unload-airplane(p0, a0, l0-0) -> load-truck(p0, t0, l0-0)
22 fly-airplane(a0, l0-0, l1-0)
23 drive-truck(t1, l1-1, l1-0, c1) -> unload-truck(p4, t1, l1-0) -> load-airplane(p4, a1, l1-0)
24 fly-airplane(a1, l1-0, l0-0) -> unload-airplane(p4, a1, l0-0)
25 unload-truck(p0, t0, l0-0) -> load-airplane(p0, a1, l0-0)
26 fly-airplane(a1, l0-0, l1-0) -> unload-airplane(p0, a1, l1-0) -> load-truck(p0, t1, l1-0)
27 drive-truck(t1, l1-0, l1-1, c1) -> unload-truck(p0, t1, l1-1)
\end{lstlisting}
\end{figure*}

\clearpage

\lstset{
    basicstyle=\footnotesize\ttfamily,
    keywordstyle=\bfseries, % This will apply bold to all keywords
    % Define colors for different groups of keywords
    morekeywords=[1]{Domain},
    keywordstyle=[1]\color{red}\bfseries,
    morekeywords=[2]{Objects, Primitive, Goal, Initial, Plan, plan},
    keywordstyle=[2]\bfseries,
    morekeywords=[3]{UNLOAD, TRUCK, UNLOAD, AIRPLANE, LOAD, TRUCK, FLY, AIRPLANE, DRIVE, TRUCK, LOAD, AIRPLANE },
    keywordstyle=[3]\color{orange}\bfseries,
    morekeywords=[4]{p2, t1, l1-1, t0, p0, p3, p6, l1-0, p4, l0-0, c1, l0-1, c0, p1, p5, p7, a1, a0 },
    keywordstyle=[4]\color{blue}\bfseries,
}

\begin{figure*}
\footnotesize
\begin{lstlisting}[basicstyle=\footnotesize\ttfamily]
Name: logistics-c2-s2-p8-a2 (logistics_a-2_c-2_s-2_p-8_t-2.pddl)
Objects: 
    a0, a1, c0, c1, l0-0, l0-1, l1-0, l1-1, p0, p1, p2, p3, p4, p5, p6, p7, t0, t1
Initial: 
    package(p0), package(p1), package(p2), package(p3), package(p4), package(p5)
package(p6), package(p7), truck(t0), truck(t1), location(l0-0), location(l0-1)
location(l1-0), location(l1-1), airplane(a0), airplane(a1), city(c0), city(c1)
airport(l0-0), airport(l1-0), at(p0, l0-0), at(p3, l0-0), at(p6, l0-0), at(t0
l0-1), at(p1, l0-1), at(a0, l1-0), at(a1, l1-0), at(p2, l1-0), at(p4, l1-0)
at(p7, l1-0), at(t1, l1-1), at(p5, l1-1), in-city(l0-0, c0), in-city(l0-1, c0)
in-city(l1-0, c1), in-city(l1-1, c1)
Goal: 
    at(p0, l0-0), at(p1, l0-0), at(p2, l1-1), at(p3, l0-1), at(p4, l1-0), at(p5
l1-1), at(p6, l1-0), at(p7, l1-0)

Plan has path-cycle: unchecked
Plan has subgoal-cycle: false
Primitive plan: 19
Plan: 11
1  load-truck(p1, t0, l0-1)
2  drive-truck(t0, l0-1, l0-0, c0) -> load-truck(p3, t0, l0-0)
3  drive-truck(t0, l0-0, l0-1, c0) -> unload-truck(p3, t0, l0-1)
4  drive-truck(t0, l0-1, l0-0, c0) -> load-truck(p6, t0, l0-0)
5  drive-truck(t1, l1-1, l1-0, c1) -> load-truck(p2, t1, l1-0)
6  drive-truck(t1, l1-0, l1-1, c1) -> unload-truck(p2, t1, l1-1)
7  unload-truck(p1, t0, l0-0)
8  drive-truck(t0, l0-0, l0-1, c0)
9  fly-airplane(a0, l1-0, l0-0)
10 drive-truck(t0, l0-1, l0-0, c0) -> unload-truck(p6, t0, l0-0) -> load-airplane(p6, a0, l0-0)
11 fly-airplane(a0, l0-0, l1-0) -> unload-airplane(p6, a0, l1-0)
\end{lstlisting}
\end{figure*}

\clearpage

\lstset{
    basicstyle=\footnotesize\ttfamily,
    keywordstyle=\bfseries, % This will apply bold to all keywords
    % Define colors for different groups of keywords
    morekeywords=[1]{Domain},
    keywordstyle=[1]\color{red}\bfseries,
    morekeywords=[2]{Objects, Primitive, Goal, Initial, Plan, plan},
    keywordstyle=[2]\bfseries,
    morekeywords=[3]{UNLOAD, TRUCK, UNLOAD, AIRPLANE, LOAD, TRUCK, FLY, AIRPLANE, DRIVE, TRUCK, LOAD, AIRPLANE },
    keywordstyle=[3]\color{orange}\bfseries,
    morekeywords=[4]{p2, t1, l1-1, t0, p0, p3, p6, l1-0, p4, l0-0, c1, l0-1, c0, p1, p5, p7, a1, a0 },
    keywordstyle=[4]\color{blue}\bfseries,
}

\begin{figure*}
\footnotesize
\begin{lstlisting}[basicstyle=\footnotesize\ttfamily]
Name: logistics-c2-s2-p8-a2 (logistics_a-2_c-2_s-2_p-8_t-2.pddl)
Objects: 
    a0, a1, c0, c1, l0-0, l0-1, l1-0, l1-1, p0, p1, p2, p3, p4, p5, p6, p7, t0, t1
Initial: 
    package(p0), package(p1), package(p2), package(p3), package(p4), package(p5)
package(p6), package(p7), truck(t0), truck(t1), location(l0-0), location(l0-1)
location(l1-0), location(l1-1), airplane(a0), airplane(a1), city(c0), city(c1)
airport(l0-0), airport(l1-0), at(p0, l0-0), at(p3, l0-0), at(p6, l0-0), at(t0
l0-1), at(p1, l0-1), at(a0, l1-0), at(a1, l1-0), at(p2, l1-0), at(p4, l1-0)
at(p7, l1-0), at(t1, l1-1), at(p5, l1-1), in-city(l0-0, c0), in-city(l0-1, c0)
in-city(l1-0, c1), in-city(l1-1, c1)
Goal: 
    at(p0, l0-0), at(p1, l0-0), at(p2, l1-1), at(p3, l0-1), at(p4, l1-0), at(p5
l1-1), at(p6, l1-0), at(p7, l1-0)

Plan has path-cycle: unchecked
Plan has subgoal-cycle: false
Primitive plan: 19
Plan: 11
1  load-truck(p1, t0, l0-1)
2  drive-truck(t0, l0-1, l0-0, c0) -> load-truck(p3, t0, l0-0)
3  drive-truck(t0, l0-0, l0-1, c0) -> unload-truck(p3, t0, l0-1)
4  drive-truck(t0, l0-1, l0-0, c0) -> load-truck(p6, t0, l0-0)
5  drive-truck(t1, l1-1, l1-0, c1) -> load-truck(p2, t1, l1-0)
6  drive-truck(t1, l1-0, l1-1, c1) -> unload-truck(p2, t1, l1-1)
7  unload-truck(p1, t0, l0-0)
8  drive-truck(t0, l0-0, l0-1, c0)
9  fly-airplane(a1, l1-0, l0-0)
10 drive-truck(t0, l0-1, l0-0, c0) -> unload-truck(p6, t0, l0-0) -> load-airplane(p6, a1, l0-0)
11 fly-airplane(a1, l0-0, l1-0) -> unload-airplane(p6, a1, l1-0)
\end{lstlisting}
\end{figure*}

\clearpage

\lstset{
    basicstyle=\footnotesize\ttfamily,
    keywordstyle=\bfseries, % This will apply bold to all keywords
    % Define colors for different groups of keywords
    morekeywords=[1]{Domain},
    keywordstyle=[1]\color{red}\bfseries,
    morekeywords=[2]{Objects, Primitive, Goal, Initial, Plan, plan},
    keywordstyle=[2]\bfseries,
    morekeywords=[3]{UNLOAD, TRUCK, UNLOAD, AIRPLANE, LOAD, TRUCK, FLY, AIRPLANE, DRIVE, TRUCK, LOAD, AIRPLANE },
    keywordstyle=[3]\color{orange}\bfseries,
    morekeywords=[4]{p2, t1, l1-1, t0, p0, p3, p6, l1-0, p4, l0-0, c1, l0-1, c0, p1, p5, p7, a1, a0 },
    keywordstyle=[4]\color{blue}\bfseries,
}

\begin{figure*}
\footnotesize
\begin{lstlisting}[basicstyle=\footnotesize\ttfamily]
Name: logistics-c2-s2-p8-a2 (logistics_a-2_c-2_s-2_p-8_t-2.pddl)
Objects: 
    a0, a1, c0, c1, l0-0, l0-1, l1-0, l1-1, p0, p1, p2, p3, p4, p5, p6, p7, t0, t1
Initial: 
    package(p0), package(p1), package(p2), package(p3), package(p4), package(p5)
package(p6), package(p7), truck(t0), truck(t1), location(l0-0), location(l0-1)
location(l1-0), location(l1-1), airplane(a0), airplane(a1), city(c0), city(c1)
airport(l0-0), airport(l1-0), at(p0, l0-0), at(p3, l0-0), at(p6, l0-0), at(t0
l0-1), at(p1, l0-1), at(a0, l1-0), at(a1, l1-0), at(p2, l1-0), at(p4, l1-0)
at(p7, l1-0), at(t1, l1-1), at(p5, l1-1), in-city(l0-0, c0), in-city(l0-1, c0)
in-city(l1-0, c1), in-city(l1-1, c1)
Goal: 
    at(p0, l0-0), at(p1, l0-0), at(p2, l1-1), at(p3, l0-1), at(p4, l1-0), at(p5
l1-1), at(p6, l1-0), at(p7, l1-0)

Plan has path-cycle: unchecked
Plan has subgoal-cycle: false
Primitive plan: 19
Plan: 11
1  load-truck(p1, t0, l0-1)
2  drive-truck(t0, l0-1, l0-0, c0) -> load-truck(p3, t0, l0-0)
3  drive-truck(t0, l0-0, l0-1, c0) -> unload-truck(p3, t0, l0-1)
4  drive-truck(t0, l0-1, l0-0, c0) -> load-truck(p6, t0, l0-0)
5  drive-truck(t1, l1-1, l1-0, c1) -> load-truck(p2, t1, l1-0)
6  drive-truck(t1, l1-0, l1-1, c1) -> unload-truck(p2, t1, l1-1)
7  unload-truck(p1, t0, l0-0)
8  drive-truck(t0, l0-0, l0-1, c0)
9  fly-airplane(a1, l1-0, l0-0)
10 drive-truck(t0, l0-1, l0-0, c0) -> unload-truck(p6, t0, l0-0) -> load-airplane(p6, a1, l0-0)
11 fly-airplane(a1, l0-0, l1-0) -> unload-airplane(p6, a1, l1-0)
\end{lstlisting}
\end{figure*}

\clearpage

\lstset{
    basicstyle=\footnotesize\ttfamily,
    keywordstyle=\bfseries, % This will apply bold to all keywords
    % Define colors for different groups of keywords
    morekeywords=[1]{Domain},
    keywordstyle=[1]\color{red}\bfseries,
    morekeywords=[2]{Objects, Primitive, Goal, Initial, Plan, plan},
    keywordstyle=[2]\bfseries,
    morekeywords=[3]{UNLOAD, TRUCK, UNLOAD, AIRPLANE, LOAD, TRUCK, FLY, AIRPLANE, DRIVE, TRUCK, LOAD, AIRPLANE },
    keywordstyle=[3]\color{orange}\bfseries,
    morekeywords=[4]{p2, t1, l1-1, t0, p0, p3, p6, l1-0, p4, l0-0, c1, l0-1, c0, p1, p5, p7, a1, a0 },
    keywordstyle=[4]\color{blue}\bfseries,
}

\begin{figure*}
\footnotesize
\begin{lstlisting}[basicstyle=\footnotesize\ttfamily]
Name: logistics-c2-s2-p8-a2 (logistics_a-2_c-2_s-2_p-8_t-2.pddl)
Objects: 
    a0, a1, c0, c1, l0-0, l0-1, l1-0, l1-1, p0, p1, p2, p3, p4, p5, p6, p7, t0, t1
Initial: 
    package(p0), package(p1), package(p2), package(p3), package(p4), package(p5)
package(p6), package(p7), truck(t0), truck(t1), location(l0-0), location(l0-1)
location(l1-0), location(l1-1), airplane(a0), airplane(a1), city(c0), city(c1)
airport(l0-0), airport(l1-0), at(p0, l0-0), at(p3, l0-0), at(p6, l0-0), at(t0
l0-1), at(p1, l0-1), at(a0, l1-0), at(a1, l1-0), at(p2, l1-0), at(p4, l1-0)
at(p7, l1-0), at(t1, l1-1), at(p5, l1-1), in-city(l0-0, c0), in-city(l0-1, c0)
in-city(l1-0, c1), in-city(l1-1, c1)
Goal: 
    at(p0, l0-0), at(p1, l0-0), at(p2, l1-1), at(p3, l0-1), at(p4, l1-0), at(p5
l1-1), at(p6, l1-0), at(p7, l1-0)

Plan has path-cycle: unchecked
Plan has subgoal-cycle: false
Primitive plan: 19
Plan: 11
1  load-truck(p1, t0, l0-1)
2  drive-truck(t0, l0-1, l0-0, c0) -> load-truck(p3, t0, l0-0)
3  drive-truck(t0, l0-0, l0-1, c0) -> unload-truck(p3, t0, l0-1)
4  drive-truck(t0, l0-1, l0-0, c0) -> load-truck(p6, t0, l0-0)
5  drive-truck(t1, l1-1, l1-0, c1) -> load-truck(p2, t1, l1-0)
6  drive-truck(t1, l1-0, l1-1, c1) -> unload-truck(p2, t1, l1-1)
7  unload-truck(p1, t0, l0-0)
8  drive-truck(t0, l0-0, l0-1, c0)
9  fly-airplane(a1, l1-0, l0-0)
10 drive-truck(t0, l0-1, l0-0, c0) -> unload-truck(p6, t0, l0-0) -> load-airplane(p6, a1, l0-0)
11 fly-airplane(a1, l0-0, l1-0) -> unload-airplane(p6, a1, l1-0)
\end{lstlisting}
\end{figure*}

\clearpage

\lstset{
    basicstyle=\footnotesize\ttfamily,
    keywordstyle=\bfseries, % This will apply bold to all keywords
    % Define colors for different groups of keywords
    morekeywords=[1]{Domain},
    keywordstyle=[1]\color{red}\bfseries,
    morekeywords=[2]{Objects, Primitive, Goal, Initial, Plan, plan},
    keywordstyle=[2]\bfseries,
    morekeywords=[3]{UNLOAD, TRUCK, UNLOAD, AIRPLANE, LOAD, TRUCK, FLY, AIRPLANE, DRIVE, TRUCK, LOAD, AIRPLANE },
    keywordstyle=[3]\color{orange}\bfseries,
    morekeywords=[4]{p2, t1, l1-1, t0, t2, p0, c2, l2-1, p3, l2-0, l1-0, l0-0, c1, l0-1, c0, p1, a1, a0 },
    keywordstyle=[4]\color{blue}\bfseries,
}

\lstset{
    basicstyle=\footnotesize\ttfamily,
    keywordstyle=\bfseries, % This will apply bold to all keywords
    % Define colors for different groups of keywords
    morekeywords=[1]{Domain},
    keywordstyle=[1]\color{red}\bfseries,
    morekeywords=[2]{Objects, Primitive, Goal, Initial, Plan, plan},
    keywordstyle=[2]\bfseries,
    morekeywords=[3]{UNLOAD, TRUCK, UNLOAD, AIRPLANE, LOAD, TRUCK, FLY, AIRPLANE, DRIVE, TRUCK, LOAD, AIRPLANE },
    keywordstyle=[3]\color{orange}\bfseries,
    morekeywords=[4]{p2, t1, l1-1, t0, t2, p0, c2, l2-1, p3, l2-0, l1-0, l0-0, c1, l0-1, c0, p1, a1, a0 },
    keywordstyle=[4]\color{blue}\bfseries,
}

\lstset{
    basicstyle=\footnotesize\ttfamily,
    keywordstyle=\bfseries, % This will apply bold to all keywords
    % Define colors for different groups of keywords
    morekeywords=[1]{Domain},
    keywordstyle=[1]\color{red}\bfseries,
    morekeywords=[2]{Objects, Primitive, Goal, Initial, Plan, plan},
    keywordstyle=[2]\bfseries,
    morekeywords=[3]{UNLOAD, TRUCK, UNLOAD, AIRPLANE, LOAD, TRUCK, FLY, AIRPLANE, DRIVE, TRUCK, LOAD, AIRPLANE },
    keywordstyle=[3]\color{orange}\bfseries,
    morekeywords=[4]{t2, p3, l1-0, l0-1, p2, p5, p1, t1, t0, l2-0, l0-0, a1, l1-1, p0, c2, l2-1, p6, p4, c1, c0, a0 },
    keywordstyle=[4]\color{blue}\bfseries,
}

\lstset{
    basicstyle=\footnotesize\ttfamily,
    keywordstyle=\bfseries, % This will apply bold to all keywords
    % Define colors for different groups of keywords
    morekeywords=[1]{Domain},
    keywordstyle=[1]\color{red}\bfseries,
    morekeywords=[2]{Objects, Primitive, Goal, Initial, Plan, plan},
    keywordstyle=[2]\bfseries,
    morekeywords=[3]{UNLOAD, TRUCK, UNLOAD, AIRPLANE, LOAD, TRUCK, FLY, AIRPLANE, DRIVE, TRUCK, LOAD, AIRPLANE },
    keywordstyle=[3]\color{orange}\bfseries,
    morekeywords=[4]{t2, l1-0, l0-1, l3-0, p1, l3-1, t1, t0, l2-0, l0-0, a1, t3, l1-1, p0, c2, l2-1, c3, c1, c0, a0 },
    keywordstyle=[4]\color{blue}\bfseries,
}

\begin{figure*}
\footnotesize
\begin{lstlisting}[basicstyle=\footnotesize\ttfamily]
Name: logistics-c4-s2-p2-a2 (logistics_a-2_c-4_s-2_p-2_t-4.pddl)
Objects: 
    a0, a1, c0, c1, c2, c3, l0-0, l0-1, l1-0, l1-1, l2-0, l2-1, l3-0, l3-1, p0, p1
t0, t1, t2, t3
Initial: 
    package(p0), package(p1), truck(t0), truck(t1), truck(t2), truck(t3)
location(l0-0), location(l0-1), location(l1-0), location(l1-1), location(l2-0)
location(l2-1), location(l3-0), location(l3-1), airplane(a0), airplane(a1)
city(c0), city(c1), city(c2), city(c3), airport(l0-0), airport(l1-0)
airport(l2-0), airport(l3-0), at(t0, l0-1), at(p0, l0-1), at(a1, l1-0), at(t1
l1-1), at(t2, l2-0), at(a0, l3-0), at(t3, l3-0), at(p1, l3-0), in-city(l0-0, c0)
in-city(l0-1, c0), in-city(l1-0, c1), in-city(l1-1, c1), in-city(l2-0, c2)
in-city(l2-1, c2), in-city(l3-0, c3), in-city(l3-1, c3)
Goal: 
    at(p0, l2-0), at(p1, l1-0)

Plan has path-cycle: unchecked
Plan has subgoal-cycle: false
Primitive plan: 10
Plan: 6
1 load-airplane(p1, a0, l3-0)
2 fly-airplane(a0, l3-0, l1-0) -> unload-airplane(p1, a0, l1-0)
3 load-truck(p0, t0, l0-1)
4 drive-truck(t0, l0-1, l0-0, c0) -> unload-truck(p0, t0, l0-0)
5 fly-airplane(a0, l1-0, l0-0) -> load-airplane(p0, a0, l0-0)
6 fly-airplane(a0, l0-0, l2-0) -> unload-airplane(p0, a0, l2-0)
\end{lstlisting}
\end{figure*}

\clearpage

\lstset{
    basicstyle=\footnotesize\ttfamily,
    keywordstyle=\bfseries, % This will apply bold to all keywords
    % Define colors for different groups of keywords
    morekeywords=[1]{Domain},
    keywordstyle=[1]\color{red}\bfseries,
    morekeywords=[2]{Objects, Primitive, Goal, Initial, Plan, plan},
    keywordstyle=[2]\bfseries,
    morekeywords=[3]{UNLOAD, TRUCK, UNLOAD, AIRPLANE, LOAD, TRUCK, FLY, AIRPLANE, DRIVE, TRUCK, LOAD, AIRPLANE },
    keywordstyle=[3]\color{orange}\bfseries,
    morekeywords=[4]{t2, l1-0, l0-1, l3-0, p1, l3-1, t1, t0, l2-0, l0-0, a1, t3, l1-1, p0, c2, l2-1, c3, c1, c0, a0 },
    keywordstyle=[4]\color{blue}\bfseries,
}

\begin{figure*}
\footnotesize
\begin{lstlisting}[basicstyle=\footnotesize\ttfamily]
Name: logistics-c4-s2-p2-a2 (logistics_a-2_c-4_s-2_p-2_t-4.pddl)
Objects: 
    a0, a1, c0, c1, c2, c3, l0-0, l0-1, l1-0, l1-1, l2-0, l2-1, l3-0, l3-1, p0, p1
t0, t1, t2, t3
Initial: 
    package(p0), package(p1), truck(t0), truck(t1), truck(t2), truck(t3)
location(l0-0), location(l0-1), location(l1-0), location(l1-1), location(l2-0)
location(l2-1), location(l3-0), location(l3-1), airplane(a0), airplane(a1)
city(c0), city(c1), city(c2), city(c3), airport(l0-0), airport(l1-0)
airport(l2-0), airport(l3-0), at(t0, l0-1), at(p0, l0-1), at(a1, l1-0), at(t1
l1-1), at(t2, l2-0), at(a0, l3-0), at(t3, l3-0), at(p1, l3-0), in-city(l0-0, c0)
in-city(l0-1, c0), in-city(l1-0, c1), in-city(l1-1, c1), in-city(l2-0, c2)
in-city(l2-1, c2), in-city(l3-0, c3), in-city(l3-1, c3)
Goal: 
    at(p0, l2-0), at(p1, l1-0)

Plan has path-cycle: unchecked
Plan has subgoal-cycle: false
Primitive plan: 10
Plan: 6
1 load-airplane(p1, a0, l3-0)
2 fly-airplane(a0, l3-0, l1-0) -> unload-airplane(p1, a0, l1-0)
3 load-truck(p0, t0, l0-1)
4 drive-truck(t0, l0-1, l0-0, c0) -> unload-truck(p0, t0, l0-0)
5 fly-airplane(a0, l1-0, l0-0) -> load-airplane(p0, a0, l0-0)
6 fly-airplane(a0, l0-0, l2-0) -> unload-airplane(p0, a0, l2-0)
\end{lstlisting}
\end{figure*}

\clearpage

\lstset{
    basicstyle=\footnotesize\ttfamily,
    keywordstyle=\bfseries, % This will apply bold to all keywords
    % Define colors for different groups of keywords
    morekeywords=[1]{Domain},
    keywordstyle=[1]\color{red}\bfseries,
    morekeywords=[2]{Objects, Primitive, Goal, Initial, Plan, plan},
    keywordstyle=[2]\bfseries,
    morekeywords=[3]{UNLOAD, TRUCK, UNLOAD, AIRPLANE, LOAD, TRUCK, FLY, AIRPLANE, DRIVE, TRUCK, LOAD, AIRPLANE },
    keywordstyle=[3]\color{orange}\bfseries,
    morekeywords=[4]{t2, l1-0, l0-1, l3-0, p1, l3-1, t1, t0, l2-0, l0-0, a1, t3, l1-1, p0, c2, l2-1, c3, c1, c0, a0 },
    keywordstyle=[4]\color{blue}\bfseries,
}

\begin{figure*}
\footnotesize
\begin{lstlisting}[basicstyle=\footnotesize\ttfamily]
Name: logistics-c4-s2-p2-a2 (logistics_a-2_c-4_s-2_p-2_t-4.pddl)
Objects: 
    a0, a1, c0, c1, c2, c3, l0-0, l0-1, l1-0, l1-1, l2-0, l2-1, l3-0, l3-1, p0, p1
t0, t1, t2, t3
Initial: 
    package(p0), package(p1), truck(t0), truck(t1), truck(t2), truck(t3)
location(l0-0), location(l0-1), location(l1-0), location(l1-1), location(l2-0)
location(l2-1), location(l3-0), location(l3-1), airplane(a0), airplane(a1)
city(c0), city(c1), city(c2), city(c3), airport(l0-0), airport(l1-0)
airport(l2-0), airport(l3-0), at(t0, l0-1), at(p0, l0-1), at(a1, l1-0), at(t1
l1-1), at(t2, l2-0), at(a0, l3-0), at(t3, l3-0), at(p1, l3-0), in-city(l0-0, c0)
in-city(l0-1, c0), in-city(l1-0, c1), in-city(l1-1, c1), in-city(l2-0, c2)
in-city(l2-1, c2), in-city(l3-0, c3), in-city(l3-1, c3)
Goal: 
    at(p0, l2-0), at(p1, l1-0)

Plan has path-cycle: unchecked
Plan has subgoal-cycle: false
Primitive plan: 10
Plan: 6
1 load-airplane(p1, a0, l3-0)
2 fly-airplane(a0, l3-0, l1-0) -> unload-airplane(p1, a0, l1-0)
3 load-truck(p0, t0, l0-1)
4 drive-truck(t0, l0-1, l0-0, c0) -> unload-truck(p0, t0, l0-0)
5 fly-airplane(a0, l1-0, l0-0) -> load-airplane(p0, a0, l0-0)
6 fly-airplane(a0, l0-0, l2-0) -> unload-airplane(p0, a0, l2-0)
\end{lstlisting}
\end{figure*}

\clearpage

\lstset{
    basicstyle=\footnotesize\ttfamily,
    keywordstyle=\bfseries, % This will apply bold to all keywords
    % Define colors for different groups of keywords
    morekeywords=[1]{Domain},
    keywordstyle=[1]\color{red}\bfseries,
    morekeywords=[2]{Objects, Primitive, Goal, Initial, Plan, plan},
    keywordstyle=[2]\bfseries,
    morekeywords=[3]{UNLOAD, TRUCK, UNLOAD, AIRPLANE, LOAD, TRUCK, FLY, AIRPLANE, DRIVE, TRUCK, LOAD, AIRPLANE },
    keywordstyle=[3]\color{orange}\bfseries,
    morekeywords=[4]{t2, l1-0, l0-1, l3-0, p1, l3-1, t1, t0, l2-0, l0-0, a1, t3, l1-1, p0, c2, l2-1, c3, c1, c0, a0 },
    keywordstyle=[4]\color{blue}\bfseries,
}

\begin{figure*}
\footnotesize
\begin{lstlisting}[basicstyle=\footnotesize\ttfamily]
Name: logistics-c4-s2-p2-a2 (logistics_a-2_c-4_s-2_p-2_t-4.pddl)
Objects: 
    a0, a1, c0, c1, c2, c3, l0-0, l0-1, l1-0, l1-1, l2-0, l2-1, l3-0, l3-1, p0, p1
t0, t1, t2, t3
Initial: 
    package(p0), package(p1), truck(t0), truck(t1), truck(t2), truck(t3)
location(l0-0), location(l0-1), location(l1-0), location(l1-1), location(l2-0)
location(l2-1), location(l3-0), location(l3-1), airplane(a0), airplane(a1)
city(c0), city(c1), city(c2), city(c3), airport(l0-0), airport(l1-0)
airport(l2-0), airport(l3-0), at(t0, l0-1), at(p0, l0-1), at(a1, l1-0), at(t1
l1-1), at(t2, l2-0), at(a0, l3-0), at(t3, l3-0), at(p1, l3-0), in-city(l0-0, c0)
in-city(l0-1, c0), in-city(l1-0, c1), in-city(l1-1, c1), in-city(l2-0, c2)
in-city(l2-1, c2), in-city(l3-0, c3), in-city(l3-1, c3)
Goal: 
    at(p0, l2-0), at(p1, l1-0)

Plan has path-cycle: unchecked
Plan has subgoal-cycle: false
Primitive plan: 10
Plan: 6
1 load-airplane(p1, a0, l3-0)
2 fly-airplane(a0, l3-0, l1-0) -> unload-airplane(p1, a0, l1-0)
3 load-truck(p0, t0, l0-1)
4 drive-truck(t0, l0-1, l0-0, c0) -> unload-truck(p0, t0, l0-0)
5 fly-airplane(a1, l1-0, l0-0) -> load-airplane(p0, a1, l0-0)
6 fly-airplane(a1, l0-0, l2-0) -> unload-airplane(p0, a1, l2-0)
\end{lstlisting}
\end{figure*}

\clearpage

\lstset{
    basicstyle=\footnotesize\ttfamily,
    keywordstyle=\bfseries, % This will apply bold to all keywords
    % Define colors for different groups of keywords
    morekeywords=[1]{Domain},
    keywordstyle=[1]\color{red}\bfseries,
    morekeywords=[2]{Objects, Primitive, Goal, Initial, Plan, plan},
    keywordstyle=[2]\bfseries,
    morekeywords=[3]{UNLOAD, TRUCK, UNLOAD, AIRPLANE, LOAD, TRUCK, FLY, AIRPLANE, DRIVE, TRUCK, LOAD, AIRPLANE },
    keywordstyle=[3]\color{orange}\bfseries,
    morekeywords=[4]{t2, p3, l1-0, l0-1, p2, l3-0, p1, l3-1, t1, t0, l2-0, l0-0, a1, t3, l1-1, p0, c2, l2-1, c3, p4, c1, c0, a0 },
    keywordstyle=[4]\color{blue}\bfseries,
}

\begin{figure*}
\footnotesize
\begin{lstlisting}[basicstyle=\footnotesize\ttfamily]
Name: logistics-c4-s2-p5-a2 (logistics_a-2_c-4_s-2_p-5_t-4.pddl)
Objects: 
    a0, a1, c0, c1, c2, c3, l0-0, l0-1, l1-0, l1-1, l2-0, l2-1, l3-0, l3-1, p0, p1
p2, p3, p4, t0, t1, t2, t3
Initial: 
    package(p0), package(p1), package(p2), package(p3), package(p4), truck(t0)
truck(t1), truck(t2), truck(t3), location(l0-0), location(l0-1), location(l1-0)
location(l1-1), location(l2-0), location(l2-1), location(l3-0), location(l3-1)
airplane(a0), airplane(a1), city(c0), city(c1), city(c2), city(c3)
airport(l0-0), airport(l1-0), airport(l2-0), airport(l3-0), at(a0, l0-0), at(t0
l0-1), at(p0, l0-1), at(p3, l1-0), at(t1, l1-1), at(t2, l2-0), at(p2, l2-0)
at(a1, l3-0), at(t3, l3-0), at(p1, l3-0), at(p4, l3-1), in-city(l0-0, c0)
in-city(l0-1, c0), in-city(l1-0, c1), in-city(l1-1, c1), in-city(l2-0, c2)
in-city(l2-1, c2), in-city(l3-0, c3), in-city(l3-1, c3)
Goal: 
    at(p0, l2-0), at(p1, l1-0), at(p2, l0-0), at(p3, l2-0), at(p4, l3-1)

Plan has path-cycle: unchecked
Plan has subgoal-cycle: false
Primitive plan: 15
Plan: 9
1 load-truck(p0, t0, l0-1)
2 load-airplane(p1, a1, l3-0)
3 fly-airplane(a1, l3-0, l1-0) -> unload-airplane(p1, a1, l1-0)
4 load-airplane(p3, a1, l1-0)
5 fly-airplane(a1, l1-0, l2-0) -> unload-airplane(p3, a1, l2-0)
6 load-airplane(p2, a1, l2-0)
7 fly-airplane(a1, l2-0, l0-0) -> unload-airplane(p2, a1, l0-0)
8 drive-truck(t0, l0-1, l0-0, c0) -> unload-truck(p0, t0, l0-0) -> load-airplane(p0, a1, l0-0)
9 fly-airplane(a1, l0-0, l2-0) -> unload-airplane(p0, a1, l2-0)
\end{lstlisting}
\end{figure*}

\clearpage

\lstset{
    basicstyle=\footnotesize\ttfamily,
    keywordstyle=\bfseries, % This will apply bold to all keywords
    % Define colors for different groups of keywords
    morekeywords=[1]{Domain},
    keywordstyle=[1]\color{red}\bfseries,
    morekeywords=[2]{Objects, Primitive, Goal, Initial, Plan, plan},
    keywordstyle=[2]\bfseries,
    morekeywords=[3]{UNLOAD, TRUCK, UNLOAD, AIRPLANE, LOAD, TRUCK, FLY, AIRPLANE, DRIVE, TRUCK, LOAD, AIRPLANE },
    keywordstyle=[3]\color{orange}\bfseries,
    morekeywords=[4]{t2, p3, l1-0, l0-1, p2, l3-0, p1, l3-1, t1, t0, l2-0, l0-0, a1, t3, l1-1, p0, c2, l2-1, c3, p4, c1, c0, a0 },
    keywordstyle=[4]\color{blue}\bfseries,
}

\begin{figure*}
\footnotesize
\begin{lstlisting}[basicstyle=\footnotesize\ttfamily]
Name: logistics-c4-s2-p5-a2 (logistics_a-2_c-4_s-2_p-5_t-4.pddl)
Objects: 
    a0, a1, c0, c1, c2, c3, l0-0, l0-1, l1-0, l1-1, l2-0, l2-1, l3-0, l3-1, p0, p1
p2, p3, p4, t0, t1, t2, t3
Initial: 
    package(p0), package(p1), package(p2), package(p3), package(p4), truck(t0)
truck(t1), truck(t2), truck(t3), location(l0-0), location(l0-1), location(l1-0)
location(l1-1), location(l2-0), location(l2-1), location(l3-0), location(l3-1)
airplane(a0), airplane(a1), city(c0), city(c1), city(c2), city(c3)
airport(l0-0), airport(l1-0), airport(l2-0), airport(l3-0), at(a0, l0-0), at(t0
l0-1), at(p0, l0-1), at(p3, l1-0), at(t1, l1-1), at(t2, l2-0), at(p2, l2-0)
at(a1, l3-0), at(t3, l3-0), at(p1, l3-0), at(p4, l3-1), in-city(l0-0, c0)
in-city(l0-1, c0), in-city(l1-0, c1), in-city(l1-1, c1), in-city(l2-0, c2)
in-city(l2-1, c2), in-city(l3-0, c3), in-city(l3-1, c3)
Goal: 
    at(p0, l2-0), at(p1, l1-0), at(p2, l0-0), at(p3, l2-0), at(p4, l3-1)

Plan has path-cycle: unchecked
Plan has subgoal-cycle: false
Primitive plan: 15
Plan: 9
1 load-truck(p0, t0, l0-1)
2 load-airplane(p1, a1, l3-0)
3 fly-airplane(a1, l3-0, l1-0) -> unload-airplane(p1, a1, l1-0)
4 load-airplane(p3, a1, l1-0)
5 fly-airplane(a1, l1-0, l2-0) -> unload-airplane(p3, a1, l2-0)
6 load-airplane(p2, a1, l2-0)
7 fly-airplane(a1, l2-0, l0-0) -> unload-airplane(p2, a1, l0-0)
8 drive-truck(t0, l0-1, l0-0, c0) -> unload-truck(p0, t0, l0-0) -> load-airplane(p0, a1, l0-0)
9 fly-airplane(a1, l0-0, l2-0) -> unload-airplane(p0, a1, l2-0)
\end{lstlisting}
\end{figure*}

\clearpage

\lstset{
    basicstyle=\footnotesize\ttfamily,
    keywordstyle=\bfseries, % This will apply bold to all keywords
    % Define colors for different groups of keywords
    morekeywords=[1]{Domain},
    keywordstyle=[1]\color{red}\bfseries,
    morekeywords=[2]{Objects, Primitive, Goal, Initial, Plan, plan},
    keywordstyle=[2]\bfseries,
    morekeywords=[3]{UNLOAD, TRUCK, UNLOAD, AIRPLANE, LOAD, TRUCK, FLY, AIRPLANE, DRIVE, TRUCK, LOAD, AIRPLANE },
    keywordstyle=[3]\color{orange}\bfseries,
    morekeywords=[4]{t2, p3, l1-0, l0-1, p2, l3-0, p1, l3-1, t1, t0, l2-0, l0-0, a1, t3, l1-1, p0, c2, l2-1, c3, p4, c1, c0, a0 },
    keywordstyle=[4]\color{blue}\bfseries,
}

\begin{figure*}
\footnotesize
\begin{lstlisting}[basicstyle=\footnotesize\ttfamily]
Name: logistics-c4-s2-p5-a2 (logistics_a-2_c-4_s-2_p-5_t-4.pddl)
Objects: 
    a0, a1, c0, c1, c2, c3, l0-0, l0-1, l1-0, l1-1, l2-0, l2-1, l3-0, l3-1, p0, p1
p2, p3, p4, t0, t1, t2, t3
Initial: 
    package(p0), package(p1), package(p2), package(p3), package(p4), truck(t0)
truck(t1), truck(t2), truck(t3), location(l0-0), location(l0-1), location(l1-0)
location(l1-1), location(l2-0), location(l2-1), location(l3-0), location(l3-1)
airplane(a0), airplane(a1), city(c0), city(c1), city(c2), city(c3)
airport(l0-0), airport(l1-0), airport(l2-0), airport(l3-0), at(a0, l0-0), at(t0
l0-1), at(p0, l0-1), at(p3, l1-0), at(t1, l1-1), at(t2, l2-0), at(p2, l2-0)
at(a1, l3-0), at(t3, l3-0), at(p1, l3-0), at(p4, l3-1), in-city(l0-0, c0)
in-city(l0-1, c0), in-city(l1-0, c1), in-city(l1-1, c1), in-city(l2-0, c2)
in-city(l2-1, c2), in-city(l3-0, c3), in-city(l3-1, c3)
Goal: 
    at(p0, l2-0), at(p1, l1-0), at(p2, l0-0), at(p3, l2-0), at(p4, l3-1)

Plan has path-cycle: unchecked
Plan has subgoal-cycle: false
Primitive plan: 15
Plan: 9
1 load-truck(p0, t0, l0-1)
2 load-airplane(p1, a1, l3-0)
3 fly-airplane(a1, l3-0, l1-0) -> unload-airplane(p1, a1, l1-0)
4 load-airplane(p3, a1, l1-0)
5 fly-airplane(a1, l1-0, l2-0) -> unload-airplane(p3, a1, l2-0)
6 load-airplane(p2, a1, l2-0)
7 fly-airplane(a1, l2-0, l0-0) -> unload-airplane(p2, a1, l0-0)
8 drive-truck(t0, l0-1, l0-0, c0) -> unload-truck(p0, t0, l0-0) -> load-airplane(p0, a0, l0-0)
9 fly-airplane(a0, l0-0, l2-0) -> unload-airplane(p0, a0, l2-0)
\end{lstlisting}
\end{figure*}

\clearpage

\lstset{
    basicstyle=\footnotesize\ttfamily,
    keywordstyle=\bfseries, % This will apply bold to all keywords
    % Define colors for different groups of keywords
    morekeywords=[1]{Domain},
    keywordstyle=[1]\color{red}\bfseries,
    morekeywords=[2]{Objects, Primitive, Goal, Initial, Plan, plan},
    keywordstyle=[2]\bfseries,
    morekeywords=[3]{UNLOAD, TRUCK, UNLOAD, AIRPLANE, LOAD, TRUCK, FLY, AIRPLANE, DRIVE, TRUCK, LOAD, AIRPLANE },
    keywordstyle=[3]\color{orange}\bfseries,
    morekeywords=[4]{t2, p3, l1-0, l0-1, p2, l3-0, p1, l3-1, t1, t0, l2-0, l0-0, a1, t3, l1-1, p0, c2, l2-1, c3, p4, c1, c0, a0 },
    keywordstyle=[4]\color{blue}\bfseries,
}

\begin{figure*}
\footnotesize
\begin{lstlisting}[basicstyle=\footnotesize\ttfamily]
Name: logistics-c4-s2-p5-a2 (logistics_a-2_c-4_s-2_p-5_t-4.pddl)
Objects: 
    a0, a1, c0, c1, c2, c3, l0-0, l0-1, l1-0, l1-1, l2-0, l2-1, l3-0, l3-1, p0, p1
p2, p3, p4, t0, t1, t2, t3
Initial: 
    package(p0), package(p1), package(p2), package(p3), package(p4), truck(t0)
truck(t1), truck(t2), truck(t3), location(l0-0), location(l0-1), location(l1-0)
location(l1-1), location(l2-0), location(l2-1), location(l3-0), location(l3-1)
airplane(a0), airplane(a1), city(c0), city(c1), city(c2), city(c3)
airport(l0-0), airport(l1-0), airport(l2-0), airport(l3-0), at(a0, l0-0), at(t0
l0-1), at(p0, l0-1), at(p3, l1-0), at(t1, l1-1), at(t2, l2-0), at(p2, l2-0)
at(a1, l3-0), at(t3, l3-0), at(p1, l3-0), at(p4, l3-1), in-city(l0-0, c0)
in-city(l0-1, c0), in-city(l1-0, c1), in-city(l1-1, c1), in-city(l2-0, c2)
in-city(l2-1, c2), in-city(l3-0, c3), in-city(l3-1, c3)
Goal: 
    at(p0, l2-0), at(p1, l1-0), at(p2, l0-0), at(p3, l2-0), at(p4, l3-1)

Plan has path-cycle: unchecked
Plan has subgoal-cycle: false
Primitive plan: 15
Plan: 9
1 load-truck(p0, t0, l0-1)
2 load-airplane(p1, a1, l3-0)
3 fly-airplane(a1, l3-0, l1-0) -> unload-airplane(p1, a1, l1-0)
4 load-airplane(p3, a1, l1-0)
5 fly-airplane(a1, l1-0, l2-0) -> unload-airplane(p3, a1, l2-0)
6 load-airplane(p2, a1, l2-0)
7 fly-airplane(a1, l2-0, l0-0) -> unload-airplane(p2, a1, l0-0)
8 drive-truck(t0, l0-1, l0-0, c0) -> unload-truck(p0, t0, l0-0) -> load-airplane(p0, a1, l0-0)
9 fly-airplane(a1, l0-0, l2-0) -> unload-airplane(p0, a1, l2-0)
\end{lstlisting}
\end{figure*}

\clearpage

\lstset{
    basicstyle=\footnotesize\ttfamily,
    keywordstyle=\bfseries, % This will apply bold to all keywords
    % Define colors for different groups of keywords
    morekeywords=[1]{Domain},
    keywordstyle=[1]\color{red}\bfseries,
    morekeywords=[2]{Objects, Primitive, Goal, Initial, Plan, plan},
    keywordstyle=[2]\bfseries,
    morekeywords=[3]{UNLOAD, TRUCK, UNLOAD, AIRPLANE, LOAD, TRUCK, FLY, AIRPLANE, DRIVE, TRUCK, LOAD, AIRPLANE },
    keywordstyle=[3]\color{orange}\bfseries,
    morekeywords=[4]{t4, t2, l1-0, l4-0, l0-1, l3-0, p1, l3-1, l4-1, t1, t0, c4, l2-0, l0-0, a1, t3, l1-1, p0, c2, l2-1, c3, c1, c0, a0 },
    keywordstyle=[4]\color{blue}\bfseries,
}

\lstset{
    basicstyle=\footnotesize\ttfamily,
    keywordstyle=\bfseries, % This will apply bold to all keywords
    % Define colors for different groups of keywords
    morekeywords=[1]{Domain},
    keywordstyle=[1]\color{red}\bfseries,
    morekeywords=[2]{Objects, Primitive, Goal, Initial, Plan, plan},
    keywordstyle=[2]\bfseries,
    morekeywords=[3]{UNLOAD, TRUCK, UNLOAD, AIRPLANE, LOAD, TRUCK, FLY, AIRPLANE, DRIVE, TRUCK, LOAD, AIRPLANE },
    keywordstyle=[3]\color{orange}\bfseries,
    morekeywords=[4]{t4, t2, l1-0, l4-0, l0-1, l3-0, p1, l3-1, l4-1, t1, t0, c4, l2-0, l0-0, a1, t3, l1-1, p0, c2, l2-1, c3, c1, c0, a0 },
    keywordstyle=[4]\color{blue}\bfseries,
}

\lstset{
    basicstyle=\footnotesize\ttfamily,
    keywordstyle=\bfseries, % This will apply bold to all keywords
    % Define colors for different groups of keywords
    morekeywords=[1]{Domain},
    keywordstyle=[1]\color{red}\bfseries,
    morekeywords=[2]{Objects, Primitive, Goal, Initial, Plan, plan},
    keywordstyle=[2]\bfseries,
    morekeywords=[3]{UNLOAD, TRUCK, UNLOAD, AIRPLANE, LOAD, TRUCK, FLY, AIRPLANE, DRIVE, TRUCK, LOAD, AIRPLANE },
    keywordstyle=[3]\color{orange}\bfseries,
    morekeywords=[4]{t4, t2, p3, l1-0, l4-0, l0-1, p2, l3-0, p1, l3-1, l4-1, t1, t0, c4, l2-0, l0-0, a1, t3, l1-1, p0, c2, l2-1, c3, p4, c1, c0, a0 },
    keywordstyle=[4]\color{blue}\bfseries,
}

\begin{figure*}
\footnotesize
\begin{lstlisting}[basicstyle=\footnotesize\ttfamily]
Name: logistics-c5-s2-p5-a2 (logistics_a-2_c-5_s-2_p-5_t-5.pddl)
Objects: 
    a0, a1, c0, c1, c2, c3, c4, l0-0, l0-1, l1-0, l1-1, l2-0, l2-1, l3-0, l3-1, l4-0
l4-1, p0, p1, p2, p3, p4, t0, t1, t2, t3, t4
Initial: 
    package(p0), package(p1), package(p2), package(p3), package(p4), truck(t0)
truck(t1), truck(t2), truck(t3), truck(t4), location(l0-0), location(l0-1)
location(l1-0), location(l1-1), location(l2-0), location(l2-1), location(l3-0)
location(l3-1), location(l4-0), location(l4-1), airplane(a0), airplane(a1)
city(c0), city(c1), city(c2), city(c3), city(c4), airport(l0-0), airport(l1-0)
airport(l2-0), airport(l3-0), airport(l4-0), at(t0, l0-1), at(p3, l0-1), at(a1
l1-0), at(t1, l1-1), at(t2, l2-0), at(p2, l2-1), at(t3, l3-0), at(p4, l3-0)
at(p0, l3-1), at(a0, l4-0), at(t4, l4-0), at(p1, l4-0), in-city(l0-0, c0)
in-city(l0-1, c0), in-city(l1-0, c1), in-city(l1-1, c1), in-city(l2-0, c2)
in-city(l2-1, c2), in-city(l3-0, c3), in-city(l3-1, c3), in-city(l4-0, c4)
in-city(l4-1, c4)
Goal: 
    at(p0, l3-1), at(p1, l2-0), at(p2, l0-0), at(p3, l0-1), at(p4, l3-0)

Plan has path-cycle: unchecked
Plan has subgoal-cycle: false
Primitive plan: 11
Plan: 5
1 drive-truck(t2, l2-0, l2-1, c2) -> load-truck(p2, t2, l2-1)
2 fly-airplane(a1, l1-0, l4-0) -> load-airplane(p1, a1, l4-0)
3 fly-airplane(a1, l4-0, l2-0) -> unload-airplane(p1, a1, l2-0)
4 drive-truck(t2, l2-1, l2-0, c2) -> unload-truck(p2, t2, l2-0) -> load-airplane(p2, a1, l2-0)
5 fly-airplane(a1, l2-0, l0-0) -> unload-airplane(p2, a1, l0-0)
\end{lstlisting}
\end{figure*}

\clearpage

\lstset{
    basicstyle=\footnotesize\ttfamily,
    keywordstyle=\bfseries, % This will apply bold to all keywords
    % Define colors for different groups of keywords
    morekeywords=[1]{Domain},
    keywordstyle=[1]\color{red}\bfseries,
    morekeywords=[2]{Objects, Primitive, Goal, Initial, Plan, plan},
    keywordstyle=[2]\bfseries,
    morekeywords=[3]{UNLOAD, TRUCK, UNLOAD, AIRPLANE, LOAD, TRUCK, FLY, AIRPLANE, DRIVE, TRUCK, LOAD, AIRPLANE },
    keywordstyle=[3]\color{orange}\bfseries,
    morekeywords=[4]{t4, t2, p3, l1-0, l4-0, l0-1, p2, l3-0, p1, l3-1, l4-1, t1, t0, c4, l2-0, l0-0, a1, t3, l1-1, p0, c2, l2-1, c3, p4, c1, c0, a0 },
    keywordstyle=[4]\color{blue}\bfseries,
}

\begin{figure*}
\footnotesize
\begin{lstlisting}[basicstyle=\footnotesize\ttfamily]
Name: logistics-c5-s2-p5-a2 (logistics_a-2_c-5_s-2_p-5_t-5.pddl)
Objects: 
    a0, a1, c0, c1, c2, c3, c4, l0-0, l0-1, l1-0, l1-1, l2-0, l2-1, l3-0, l3-1, l4-0
l4-1, p0, p1, p2, p3, p4, t0, t1, t2, t3, t4
Initial: 
    package(p0), package(p1), package(p2), package(p3), package(p4), truck(t0)
truck(t1), truck(t2), truck(t3), truck(t4), location(l0-0), location(l0-1)
location(l1-0), location(l1-1), location(l2-0), location(l2-1), location(l3-0)
location(l3-1), location(l4-0), location(l4-1), airplane(a0), airplane(a1)
city(c0), city(c1), city(c2), city(c3), city(c4), airport(l0-0), airport(l1-0)
airport(l2-0), airport(l3-0), airport(l4-0), at(t0, l0-1), at(p3, l0-1), at(a1
l1-0), at(t1, l1-1), at(t2, l2-0), at(p2, l2-1), at(t3, l3-0), at(p4, l3-0)
at(p0, l3-1), at(a0, l4-0), at(t4, l4-0), at(p1, l4-0), in-city(l0-0, c0)
in-city(l0-1, c0), in-city(l1-0, c1), in-city(l1-1, c1), in-city(l2-0, c2)
in-city(l2-1, c2), in-city(l3-0, c3), in-city(l3-1, c3), in-city(l4-0, c4)
in-city(l4-1, c4)
Goal: 
    at(p0, l3-1), at(p1, l2-0), at(p2, l0-0), at(p3, l0-1), at(p4, l3-0)

Plan has path-cycle: unchecked
Plan has subgoal-cycle: false
Primitive plan: 11
Plan: 5
1 drive-truck(t2, l2-0, l2-1, c2) -> load-truck(p2, t2, l2-1)
2 fly-airplane(a1, l1-0, l4-0) -> load-airplane(p1, a1, l4-0)
3 fly-airplane(a1, l4-0, l2-0) -> unload-airplane(p1, a1, l2-0)
4 drive-truck(t2, l2-1, l2-0, c2) -> unload-truck(p2, t2, l2-0) -> load-airplane(p2, a1, l2-0)
5 fly-airplane(a1, l2-0, l0-0) -> unload-airplane(p2, a1, l0-0)
\end{lstlisting}
\end{figure*}

\clearpage

\lstset{
    basicstyle=\footnotesize\ttfamily,
    keywordstyle=\bfseries, % This will apply bold to all keywords
    % Define colors for different groups of keywords
    morekeywords=[1]{Domain},
    keywordstyle=[1]\color{red}\bfseries,
    morekeywords=[2]{Objects, Primitive, Goal, Initial, Plan, plan},
    keywordstyle=[2]\bfseries,
    morekeywords=[3]{UNLOAD, TRUCK, UNLOAD, AIRPLANE, LOAD, TRUCK, FLY, AIRPLANE, DRIVE, TRUCK, LOAD, AIRPLANE },
    keywordstyle=[3]\color{orange}\bfseries,
    morekeywords=[4]{t4, t2, p3, l1-0, l4-0, l0-1, p2, l3-0, p1, l3-1, l4-1, t1, t0, c4, l2-0, l0-0, a1, t3, l1-1, p0, c2, l2-1, c3, p4, c1, c0, a0 },
    keywordstyle=[4]\color{blue}\bfseries,
}

\begin{figure*}
\footnotesize
\begin{lstlisting}[basicstyle=\footnotesize\ttfamily]
Name: logistics-c5-s2-p5-a2 (logistics_a-2_c-5_s-2_p-5_t-5.pddl)
Objects: 
    a0, a1, c0, c1, c2, c3, c4, l0-0, l0-1, l1-0, l1-1, l2-0, l2-1, l3-0, l3-1, l4-0
l4-1, p0, p1, p2, p3, p4, t0, t1, t2, t3, t4
Initial: 
    package(p0), package(p1), package(p2), package(p3), package(p4), truck(t0)
truck(t1), truck(t2), truck(t3), truck(t4), location(l0-0), location(l0-1)
location(l1-0), location(l1-1), location(l2-0), location(l2-1), location(l3-0)
location(l3-1), location(l4-0), location(l4-1), airplane(a0), airplane(a1)
city(c0), city(c1), city(c2), city(c3), city(c4), airport(l0-0), airport(l1-0)
airport(l2-0), airport(l3-0), airport(l4-0), at(t0, l0-1), at(p3, l0-1), at(a1
l1-0), at(t1, l1-1), at(t2, l2-0), at(p2, l2-1), at(t3, l3-0), at(p4, l3-0)
at(p0, l3-1), at(a0, l4-0), at(t4, l4-0), at(p1, l4-0), in-city(l0-0, c0)
in-city(l0-1, c0), in-city(l1-0, c1), in-city(l1-1, c1), in-city(l2-0, c2)
in-city(l2-1, c2), in-city(l3-0, c3), in-city(l3-1, c3), in-city(l4-0, c4)
in-city(l4-1, c4)
Goal: 
    at(p0, l3-1), at(p1, l2-0), at(p2, l0-0), at(p3, l0-1), at(p4, l3-0)

Plan has path-cycle: unchecked
Plan has subgoal-cycle: false
Primitive plan: 11
Plan: 5
1 drive-truck(t2, l2-0, l2-1, c2) -> load-truck(p2, t2, l2-1)
2 fly-airplane(a1, l1-0, l4-0) -> load-airplane(p1, a1, l4-0)
3 fly-airplane(a1, l4-0, l2-0) -> unload-airplane(p1, a1, l2-0)
4 drive-truck(t2, l2-1, l2-0, c2) -> unload-truck(p2, t2, l2-0) -> load-airplane(p2, a1, l2-0)
5 fly-airplane(a1, l2-0, l0-0) -> unload-airplane(p2, a1, l0-0)
\end{lstlisting}
\end{figure*}

\clearpage

\lstset{
    basicstyle=\footnotesize\ttfamily,
    keywordstyle=\bfseries, % This will apply bold to all keywords
    % Define colors for different groups of keywords
    morekeywords=[1]{Domain},
    keywordstyle=[1]\color{red}\bfseries,
    morekeywords=[2]{Objects, Primitive, Goal, Initial, Plan, plan},
    keywordstyle=[2]\bfseries,
    morekeywords=[3]{UNLOAD, TRUCK, UNLOAD, AIRPLANE, LOAD, TRUCK, FLY, AIRPLANE, DRIVE, TRUCK, LOAD, AIRPLANE },
    keywordstyle=[3]\color{orange}\bfseries,
    morekeywords=[4]{t4, t2, p3, l1-0, l4-0, l0-1, p2, l3-0, p1, l3-1, l4-1, t1, t0, c4, l2-0, l0-0, a1, t3, l1-1, p0, c2, l2-1, c3, p4, c1, c0, a0 },
    keywordstyle=[4]\color{blue}\bfseries,
}

\begin{figure*}
\footnotesize
\begin{lstlisting}[basicstyle=\footnotesize\ttfamily]
Name: logistics-c5-s2-p5-a2 (logistics_a-2_c-5_s-2_p-5_t-5.pddl)
Objects: 
    a0, a1, c0, c1, c2, c3, c4, l0-0, l0-1, l1-0, l1-1, l2-0, l2-1, l3-0, l3-1, l4-0
l4-1, p0, p1, p2, p3, p4, t0, t1, t2, t3, t4
Initial: 
    package(p0), package(p1), package(p2), package(p3), package(p4), truck(t0)
truck(t1), truck(t2), truck(t3), truck(t4), location(l0-0), location(l0-1)
location(l1-0), location(l1-1), location(l2-0), location(l2-1), location(l3-0)
location(l3-1), location(l4-0), location(l4-1), airplane(a0), airplane(a1)
city(c0), city(c1), city(c2), city(c3), city(c4), airport(l0-0), airport(l1-0)
airport(l2-0), airport(l3-0), airport(l4-0), at(t0, l0-1), at(p3, l0-1), at(a1
l1-0), at(t1, l1-1), at(t2, l2-0), at(p2, l2-1), at(t3, l3-0), at(p4, l3-0)
at(p0, l3-1), at(a0, l4-0), at(t4, l4-0), at(p1, l4-0), in-city(l0-0, c0)
in-city(l0-1, c0), in-city(l1-0, c1), in-city(l1-1, c1), in-city(l2-0, c2)
in-city(l2-1, c2), in-city(l3-0, c3), in-city(l3-1, c3), in-city(l4-0, c4)
in-city(l4-1, c4)
Goal: 
    at(p0, l3-1), at(p1, l2-0), at(p2, l0-0), at(p3, l0-1), at(p4, l3-0)

Plan has path-cycle: unchecked
Plan has subgoal-cycle: false
Primitive plan: 11
Plan: 5
1 drive-truck(t2, l2-0, l2-1, c2) -> load-truck(p2, t2, l2-1)
2 fly-airplane(a1, l1-0, l4-0) -> load-airplane(p1, a1, l4-0)
3 fly-airplane(a1, l4-0, l2-0) -> unload-airplane(p1, a1, l2-0)
4 drive-truck(t2, l2-1, l2-0, c2) -> unload-truck(p2, t2, l2-0) -> load-airplane(p2, a1, l2-0)
5 fly-airplane(a1, l2-0, l0-0) -> unload-airplane(p2, a1, l0-0)
\end{lstlisting}
\end{figure*}

\clearpage

\lstset{
    basicstyle=\footnotesize\ttfamily,
    keywordstyle=\bfseries, % This will apply bold to all keywords
    % Define colors for different groups of keywords
    morekeywords=[1]{Domain},
    keywordstyle=[1]\color{red}\bfseries,
    morekeywords=[2]{Objects, Primitive, Goal, Initial, Plan, plan},
    keywordstyle=[2]\bfseries,
    morekeywords=[3]{UNLOAD, TRUCK, UNLOAD, AIRPLANE, LOAD, TRUCK, FLY, AIRPLANE, DRIVE, TRUCK, LOAD, AIRPLANE },
    keywordstyle=[3]\color{orange}\bfseries,
    morekeywords=[4]{p2, t1, l1-1, t0, p0, p3, a2, l1-0, l0-0, c1, l0-1, c0, p1, p4, a1, a0 },
    keywordstyle=[4]\color{blue}\bfseries,
}

\lstset{
    basicstyle=\footnotesize\ttfamily,
    keywordstyle=\bfseries, % This will apply bold to all keywords
    % Define colors for different groups of keywords
    morekeywords=[1]{Domain},
    keywordstyle=[1]\color{red}\bfseries,
    morekeywords=[2]{Objects, Primitive, Goal, Initial, Plan, plan},
    keywordstyle=[2]\bfseries,
    morekeywords=[3]{UNLOAD, TRUCK, UNLOAD, AIRPLANE, LOAD, TRUCK, FLY, AIRPLANE, DRIVE, TRUCK, LOAD, AIRPLANE },
    keywordstyle=[3]\color{orange}\bfseries,
    morekeywords=[4]{p2, t1, l1-1, t0, p0, p3, a2, l1-0, l0-0, c1, l0-1, c0, p1, p4, a1, a0 },
    keywordstyle=[4]\color{blue}\bfseries,
}

\lstset{
    basicstyle=\footnotesize\ttfamily,
    keywordstyle=\bfseries, % This will apply bold to all keywords
    % Define colors for different groups of keywords
    morekeywords=[1]{Domain},
    keywordstyle=[1]\color{red}\bfseries,
    morekeywords=[2]{Objects, Primitive, Goal, Initial, Plan, plan},
    keywordstyle=[2]\bfseries,
    morekeywords=[3]{UNLOAD, TRUCK, UNLOAD, AIRPLANE, LOAD, TRUCK, FLY, AIRPLANE, DRIVE, TRUCK, LOAD, AIRPLANE },
    keywordstyle=[3]\color{orange}\bfseries,
    morekeywords=[4]{t4, t2, p3, l1-0, l0-1, p2, p1, t1, t0, a2, l0-0, a1, t3, l1-1, p0, p4, c1, c0, a0 },
    keywordstyle=[4]\color{blue}\bfseries,
}

\lstset{
    basicstyle=\footnotesize\ttfamily,
    keywordstyle=\bfseries, % This will apply bold to all keywords
    % Define colors for different groups of keywords
    morekeywords=[1]{Domain},
    keywordstyle=[1]\color{red}\bfseries,
    morekeywords=[2]{Objects, Primitive, Goal, Initial, Plan, plan},
    keywordstyle=[2]\bfseries,
    morekeywords=[3]{UNLOAD, TRUCK, UNLOAD, AIRPLANE, LOAD, TRUCK, FLY, AIRPLANE, DRIVE, TRUCK, LOAD, AIRPLANE },
    keywordstyle=[3]\color{orange}\bfseries,
    morekeywords=[4]{t4, t2, p3, l1-0, l0-1, p2, p1, t1, t0, a2, l0-0, a1, t3, l1-1, p0, p4, c1, c0, a0 },
    keywordstyle=[4]\color{blue}\bfseries,
}

\lstset{
    basicstyle=\footnotesize\ttfamily,
    keywordstyle=\bfseries, % This will apply bold to all keywords
    % Define colors for different groups of keywords
    morekeywords=[1]{Domain},
    keywordstyle=[1]\color{red}\bfseries,
    morekeywords=[2]{Objects, Primitive, Goal, Initial, Plan, plan},
    keywordstyle=[2]\bfseries,
    morekeywords=[3]{UNLOAD, TRUCK, UNLOAD, AIRPLANE, LOAD, TRUCK, FLY, AIRPLANE, DRIVE, TRUCK, LOAD, AIRPLANE },
    keywordstyle=[3]\color{orange}\bfseries,
    morekeywords=[4]{p2, t1, l1-1, t0, p0, p3, a2, l1-0, l0-0, c1, l0-1, c0, p1, p4, p5, a1, a0 },
    keywordstyle=[4]\color{blue}\bfseries,
}

\lstset{
    basicstyle=\footnotesize\ttfamily,
    keywordstyle=\bfseries, % This will apply bold to all keywords
    % Define colors for different groups of keywords
    morekeywords=[1]{Domain},
    keywordstyle=[1]\color{red}\bfseries,
    morekeywords=[2]{Objects, Primitive, Goal, Initial, Plan, plan},
    keywordstyle=[2]\bfseries,
    morekeywords=[3]{UNLOAD, TRUCK, UNLOAD, AIRPLANE, LOAD, TRUCK, FLY, AIRPLANE, DRIVE, TRUCK, LOAD, AIRPLANE },
    keywordstyle=[3]\color{orange}\bfseries,
    morekeywords=[4]{p2, t1, l1-1, t0, p0, p3, a2, l1-0, l0-0, c1, l0-1, c0, p1, p4, p5, a1, a0 },
    keywordstyle=[4]\color{blue}\bfseries,
}

\lstset{
    basicstyle=\footnotesize\ttfamily,
    keywordstyle=\bfseries, % This will apply bold to all keywords
    % Define colors for different groups of keywords
    morekeywords=[1]{Domain},
    keywordstyle=[1]\color{red}\bfseries,
    morekeywords=[2]{Objects, Primitive, Goal, Initial, Plan, plan},
    keywordstyle=[2]\bfseries,
    morekeywords=[3]{UNLOAD, TRUCK, UNLOAD, AIRPLANE, LOAD, TRUCK, FLY, AIRPLANE, DRIVE, TRUCK, LOAD, AIRPLANE },
    keywordstyle=[3]\color{orange}\bfseries,
    morekeywords=[4]{t2, p3, l1-0, l0-1, p2, p5, p1, t1, t0, a2, l0-0, a1, t3, l1-1, p0, p6, p4, c1, c0, a0 },
    keywordstyle=[4]\color{blue}\bfseries,
}

\lstset{
    basicstyle=\footnotesize\ttfamily,
    keywordstyle=\bfseries, % This will apply bold to all keywords
    % Define colors for different groups of keywords
    morekeywords=[1]{Domain},
    keywordstyle=[1]\color{red}\bfseries,
    morekeywords=[2]{Objects, Primitive, Goal, Initial, Plan, plan},
    keywordstyle=[2]\bfseries,
    morekeywords=[3]{UNLOAD, TRUCK, UNLOAD, AIRPLANE, LOAD, TRUCK, FLY, AIRPLANE, DRIVE, TRUCK, LOAD, AIRPLANE },
    keywordstyle=[3]\color{orange}\bfseries,
    morekeywords=[4]{t2, p3, l1-0, l0-1, p2, p5, p1, t1, t0, a2, l0-0, a1, t3, l1-1, p0, p6, p4, c1, c0, a0 },
    keywordstyle=[4]\color{blue}\bfseries,
}

\lstset{
    basicstyle=\footnotesize\ttfamily,
    keywordstyle=\bfseries, % This will apply bold to all keywords
    % Define colors for different groups of keywords
    morekeywords=[1]{Domain},
    keywordstyle=[1]\color{red}\bfseries,
    morekeywords=[2]{Objects, Primitive, Goal, Initial, Plan, plan},
    keywordstyle=[2]\bfseries,
    morekeywords=[3]{UNLOAD, TRUCK, UNLOAD, AIRPLANE, LOAD, TRUCK, FLY, AIRPLANE, DRIVE, TRUCK, LOAD, AIRPLANE },
    keywordstyle=[3]\color{orange}\bfseries,
    morekeywords=[4]{p3, l1-0, l0-1, p2, p5, p1, p7, t1, t0, a2, l0-0, a1, l1-1, p0, p6, p4, c1, c0, a0 },
    keywordstyle=[4]\color{blue}\bfseries,
}

\lstset{
    basicstyle=\footnotesize\ttfamily,
    keywordstyle=\bfseries, % This will apply bold to all keywords
    % Define colors for different groups of keywords
    morekeywords=[1]{Domain},
    keywordstyle=[1]\color{red}\bfseries,
    morekeywords=[2]{Objects, Primitive, Goal, Initial, Plan, plan},
    keywordstyle=[2]\bfseries,
    morekeywords=[3]{UNLOAD, TRUCK, UNLOAD, AIRPLANE, LOAD, TRUCK, FLY, AIRPLANE, DRIVE, TRUCK, LOAD, AIRPLANE },
    keywordstyle=[3]\color{orange}\bfseries,
    morekeywords=[4]{p3, l1-0, l0-1, p2, p5, p1, p7, t1, t0, a2, l0-0, a1, l1-1, p0, p6, p4, c1, c0, a0 },
    keywordstyle=[4]\color{blue}\bfseries,
}

\lstset{
    basicstyle=\footnotesize\ttfamily,
    keywordstyle=\bfseries, % This will apply bold to all keywords
    % Define colors for different groups of keywords
    morekeywords=[1]{Domain},
    keywordstyle=[1]\color{red}\bfseries,
    morekeywords=[2]{Objects, Primitive, Goal, Initial, Plan, plan},
    keywordstyle=[2]\bfseries,
    morekeywords=[3]{UNLOAD, TRUCK, UNLOAD, AIRPLANE, LOAD, TRUCK, FLY, AIRPLANE, DRIVE, TRUCK, LOAD, AIRPLANE },
    keywordstyle=[3]\color{orange}\bfseries,
    morekeywords=[4]{t2, p3, l1-0, l0-1, p2, p5, p1, p7, t1, t0, a2, l0-0, p8, a1, l1-1, p0, p6, p4, c1, c0, a0 },
    keywordstyle=[4]\color{blue}\bfseries,
}

\lstset{
    basicstyle=\footnotesize\ttfamily,
    keywordstyle=\bfseries, % This will apply bold to all keywords
    % Define colors for different groups of keywords
    morekeywords=[1]{Domain},
    keywordstyle=[1]\color{red}\bfseries,
    morekeywords=[2]{Objects, Primitive, Goal, Initial, Plan, plan},
    keywordstyle=[2]\bfseries,
    morekeywords=[3]{UNLOAD, TRUCK, UNLOAD, AIRPLANE, LOAD, TRUCK, FLY, AIRPLANE, DRIVE, TRUCK, LOAD, AIRPLANE },
    keywordstyle=[3]\color{orange}\bfseries,
    morekeywords=[4]{t2, p3, l1-0, l0-1, p2, p5, p1, p7, t1, t0, a2, l0-0, p8, a1, l1-1, p0, p6, p4, c1, c0, a0 },
    keywordstyle=[4]\color{blue}\bfseries,
}

\lstset{
    basicstyle=\footnotesize\ttfamily,
    keywordstyle=\bfseries, % This will apply bold to all keywords
    % Define colors for different groups of keywords
    morekeywords=[1]{Domain},
    keywordstyle=[1]\color{red}\bfseries,
    morekeywords=[2]{Objects, Primitive, Goal, Initial, Plan, plan},
    keywordstyle=[2]\bfseries,
    morekeywords=[3]{UNLOAD, TRUCK, UNLOAD, AIRPLANE, LOAD, TRUCK, FLY, AIRPLANE, DRIVE, TRUCK, LOAD, AIRPLANE },
    keywordstyle=[3]\color{orange}\bfseries,
    morekeywords=[4]{t2, l1-2, p3, l1-0, l0-1, l0-2, p2, p5, p1, p7, t1, t0, a2, l0-0, p8, a1, l1-1, p0, p6, p4, c1, c0, a0 },
    keywordstyle=[4]\color{blue}\bfseries,
}

\lstset{
    basicstyle=\footnotesize\ttfamily,
    keywordstyle=\bfseries, % This will apply bold to all keywords
    % Define colors for different groups of keywords
    morekeywords=[1]{Domain},
    keywordstyle=[1]\color{red}\bfseries,
    morekeywords=[2]{Objects, Primitive, Goal, Initial, Plan, plan},
    keywordstyle=[2]\bfseries,
    morekeywords=[3]{UNLOAD, TRUCK, UNLOAD, AIRPLANE, LOAD, TRUCK, FLY, AIRPLANE, DRIVE, TRUCK, LOAD, AIRPLANE },
    keywordstyle=[3]\color{orange}\bfseries,
    morekeywords=[4]{t2, l1-2, p3, l1-0, l0-1, l0-2, p2, p5, p1, t1, t0, l2-0, a2, l2-2, l0-0, a1, l1-1, p0, c2, l2-1, p4, c1, c0, a0 },
    keywordstyle=[4]\color{blue}\bfseries,
}

\lstset{
    basicstyle=\footnotesize\ttfamily,
    keywordstyle=\bfseries, % This will apply bold to all keywords
    % Define colors for different groups of keywords
    morekeywords=[1]{Domain},
    keywordstyle=[1]\color{red}\bfseries,
    morekeywords=[2]{Objects, Primitive, Goal, Initial, Plan, plan},
    keywordstyle=[2]\bfseries,
    morekeywords=[3]{UNLOAD, TRUCK, UNLOAD, AIRPLANE, LOAD, TRUCK, FLY, AIRPLANE, DRIVE, TRUCK, LOAD, AIRPLANE },
    keywordstyle=[3]\color{orange}\bfseries,
    morekeywords=[4]{t4, t2, p3, l1-0, l0-1, p2, l3-0, p5, p1, l3-1, p7, t1, t0, l2-0, a2, l0-0, p8, a1, t3, l1-1, p0, c2, l2-1, p6, c3, p4, c1, c0, a0 },
    keywordstyle=[4]\color{blue}\bfseries,
}

\begin{figure*}
\footnotesize
\begin{lstlisting}[basicstyle=\footnotesize\ttfamily]
Name: logistics-c4-s2-p9-a3 (logistics_a-3_c-4_s-2_p-9_t-5.pddl)
Objects: 
    a0, a1, a2, c0, c1, c2, c3, l0-0, l0-1, l1-0, l1-1, l2-0, l2-1, l3-0, l3-1, p0
p1, p2, p3, p4, p5, p6, p7, p8, t0, t1, t2, t3, t4
Initial: 
    package(p0), package(p1), package(p2), package(p3), package(p4), package(p5)
package(p6), package(p7), package(p8), truck(t0), truck(t1), truck(t2)
truck(t3), truck(t4), location(l0-0), location(l0-1), location(l1-0)
location(l1-1), location(l2-0), location(l2-1), location(l3-0), location(l3-1)
airplane(a0), airplane(a1), airplane(a2), city(c0), city(c1), city(c2), city(c3)
airport(l0-0), airport(l1-0), airport(l2-0), airport(l3-0), at(t0, l0-0), at(p6
l0-1), at(a0, l1-0), at(a1, l1-0), at(t1, l1-1), at(p3, l1-1), at(a2, l2-0)
at(t2, l2-0), at(t4, l2-0), at(p8, l2-0), at(p2, l3-0), at(p4, l3-0), at(p5
l3-0), at(t3, l3-1), at(p0, l3-1), at(p1, l3-1), at(p7, l3-1), in-city(l0-0, c0)
in-city(l0-1, c0), in-city(l1-0, c1), in-city(l1-1, c1), in-city(l2-0, c2)
in-city(l2-1, c2), in-city(l3-0, c3), in-city(l3-1, c3)
Goal: 
    at(p0, l1-1), at(p1, l2-0), at(p2, l3-0), at(p3, l1-1), at(p4, l1-1), at(p5
l3-0), at(p6, l3-0), at(p7, l1-0), at(p8, l3-0)

Plan has path-cycle: unchecked
Plan has subgoal-cycle: false
Primitive plan: 43
Plan: 5
1 drive-truck(t0, l0-0, l0-1, c0) -> load-truck(p6, t0, l0-1) -> drive-truck(t0, l0-1, l0-0, c0)
   ->unload-truck(p6, t0, l0-0) -> fly-airplane(a0, l1-0, l0-0) -> load-airplane(p6, a0, l0-0)
   ->fly-airplane(a0, l0-0, l3-0) -> unload-airplane(p6, a0, l3-0) -> load-truck(p7, t3, l3-1)
2 load-truck(p0, t3, l3-1) -> drive-truck(t3, l3-1, l3-0, c3) -> unload-truck(p0, t3, l3-0)
   ->load-airplane(p0, a0, l3-0) -> fly-airplane(a0, l3-0, l1-0) -> unload-airplane(p0, a0, l1-0)
   ->drive-truck(t1, l1-1, l1-0, c1) -> load-truck(p0, t1, l1-0) -> drive-truck(t1, l1-0, l1-1, c1)
   ->unload-truck(p0, t1, l1-1) -> drive-truck(t3, l3-0, l3-1, c3) -> load-truck(p1, t3, l3-1)
3 fly-airplane(a0, l1-0, l3-0) -> load-airplane(p4, a0, l3-0) -> fly-airplane(a0, l3-0, l1-0)
   ->unload-airplane(p4, a0, l1-0) -> drive-truck(t1, l1-1, l1-0, c1) -> load-truck(p4, t1, l1-0)
   ->drive-truck(t1, l1-0, l1-1, c1) -> unload-truck(p4, t1, l1-1) -> load-airplane(p8, a2, l2-0)
4 drive-truck(t3, l3-1, l3-0, c3) -> unload-truck(p1, t3, l3-0) -> fly-airplane(a0, l1-0, l3-0)
   ->load-airplane(p1, a0, l3-0) -> fly-airplane(a0, l3-0, l2-0) -> unload-airplane(p1, a0, l2-0)
   ->fly-airplane(a2, l2-0, l3-0) -> unload-airplane(p8, a2, l3-0)
5 unload-truck(p7, t3, l3-0) -> load-airplane(p7, a2, l3-0) -> fly-airplane(a2, l3-0, l1-0)
   ->unload-airplane(p7, a2, l1-0) -> fly-airplane(a0, l2-0, l1-0)
\end{lstlisting}
\end{figure*}

\clearpage

\lstset{
    basicstyle=\footnotesize\ttfamily,
    keywordstyle=\bfseries, % This will apply bold to all keywords
    % Define colors for different groups of keywords
    morekeywords=[1]{Domain},
    keywordstyle=[1]\color{red}\bfseries,
    morekeywords=[2]{Objects, Primitive, Goal, Initial, Plan, plan},
    keywordstyle=[2]\bfseries,
    morekeywords=[3]{UNLOAD, TRUCK, UNLOAD, AIRPLANE, LOAD, TRUCK, FLY, AIRPLANE, DRIVE, TRUCK, LOAD, AIRPLANE },
    keywordstyle=[3]\color{orange}\bfseries,
    morekeywords=[4]{t4, t2, p3, l1-0, l0-1, p2, l3-0, p5, p1, l3-1, p7, t1, t0, l2-0, a2, l0-0, p8, a1, t3, l1-1, p0, c2, l2-1, p6, c3, p4, c1, c0, a0 },
    keywordstyle=[4]\color{blue}\bfseries,
}

\begin{figure*}
\footnotesize
\begin{lstlisting}[basicstyle=\footnotesize\ttfamily]
Name: logistics-c4-s2-p9-a3 (logistics_a-3_c-4_s-2_p-9_t-5.pddl)
Objects: 
    a0, a1, a2, c0, c1, c2, c3, l0-0, l0-1, l1-0, l1-1, l2-0, l2-1, l3-0, l3-1, p0
p1, p2, p3, p4, p5, p6, p7, p8, t0, t1, t2, t3, t4
Initial: 
    package(p0), package(p1), package(p2), package(p3), package(p4), package(p5)
package(p6), package(p7), package(p8), truck(t0), truck(t1), truck(t2)
truck(t3), truck(t4), location(l0-0), location(l0-1), location(l1-0)
location(l1-1), location(l2-0), location(l2-1), location(l3-0), location(l3-1)
airplane(a0), airplane(a1), airplane(a2), city(c0), city(c1), city(c2), city(c3)
airport(l0-0), airport(l1-0), airport(l2-0), airport(l3-0), at(t0, l0-0), at(p6
l0-1), at(a0, l1-0), at(a1, l1-0), at(t1, l1-1), at(p3, l1-1), at(a2, l2-0)
at(t2, l2-0), at(t4, l2-0), at(p8, l2-0), at(p2, l3-0), at(p4, l3-0), at(p5
l3-0), at(t3, l3-1), at(p0, l3-1), at(p1, l3-1), at(p7, l3-1), in-city(l0-0, c0)
in-city(l0-1, c0), in-city(l1-0, c1), in-city(l1-1, c1), in-city(l2-0, c2)
in-city(l2-1, c2), in-city(l3-0, c3), in-city(l3-1, c3)
Goal: 
    at(p0, l1-1), at(p1, l2-0), at(p2, l3-0), at(p3, l1-1), at(p4, l1-1), at(p5
l3-0), at(p6, l3-0), at(p7, l1-0), at(p8, l3-0)

Plan has path-cycle: unchecked
Plan has subgoal-cycle: false
Primitive plan: 43
Plan: 5
1 drive-truck(t0, l0-0, l0-1, c0) -> load-truck(p6, t0, l0-1) -> drive-truck(t0, l0-1, l0-0, c0)
   ->unload-truck(p6, t0, l0-0) -> fly-airplane(a0, l1-0, l0-0) -> load-airplane(p6, a0, l0-0)
   ->fly-airplane(a0, l0-0, l3-0) -> unload-airplane(p6, a0, l3-0) -> load-truck(p7, t3, l3-1)
2 load-truck(p0, t3, l3-1) -> drive-truck(t3, l3-1, l3-0, c3) -> unload-truck(p0, t3, l3-0)
   ->load-airplane(p0, a0, l3-0) -> fly-airplane(a0, l3-0, l1-0) -> unload-airplane(p0, a0, l1-0)
   ->drive-truck(t1, l1-1, l1-0, c1) -> load-truck(p0, t1, l1-0) -> drive-truck(t1, l1-0, l1-1, c1)
   ->unload-truck(p0, t1, l1-1) -> drive-truck(t3, l3-0, l3-1, c3) -> load-truck(p1, t3, l3-1)
3 fly-airplane(a0, l1-0, l3-0) -> load-airplane(p4, a0, l3-0) -> fly-airplane(a0, l3-0, l1-0)
   ->unload-airplane(p4, a0, l1-0) -> drive-truck(t1, l1-1, l1-0, c1) -> load-truck(p4, t1, l1-0)
   ->drive-truck(t1, l1-0, l1-1, c1) -> unload-truck(p4, t1, l1-1) -> load-airplane(p8, a2, l2-0)
4 drive-truck(t3, l3-1, l3-0, c3) -> unload-truck(p1, t3, l3-0) -> fly-airplane(a0, l1-0, l3-0)
   ->load-airplane(p1, a0, l3-0) -> fly-airplane(a0, l3-0, l2-0) -> unload-airplane(p1, a0, l2-0)
   ->fly-airplane(a2, l2-0, l3-0) -> unload-airplane(p8, a2, l3-0)
5 unload-truck(p7, t3, l3-0) -> load-airplane(p7, a2, l3-0) -> fly-airplane(a2, l3-0, l1-0)
   ->unload-airplane(p7, a2, l1-0) -> fly-airplane(a0, l2-0, l1-0)
\end{lstlisting}
\end{figure*}

\clearpage

\lstset{
    basicstyle=\footnotesize\ttfamily,
    keywordstyle=\bfseries, % This will apply bold to all keywords
    % Define colors for different groups of keywords
    morekeywords=[1]{Domain},
    keywordstyle=[1]\color{red}\bfseries,
    morekeywords=[2]{Objects, Primitive, Goal, Initial, Plan, plan},
    keywordstyle=[2]\bfseries,
    morekeywords=[3]{UNLOAD, TRUCK, UNLOAD, AIRPLANE, LOAD, TRUCK, FLY, AIRPLANE, DRIVE, TRUCK, LOAD, AIRPLANE },
    keywordstyle=[3]\color{orange}\bfseries,
    morekeywords=[4]{t4, t2, p3, l1-0, l0-1, p2, l3-0, p5, p1, l3-1, p7, t1, t0, l2-0, a2, l0-0, p8, a1, t3, l1-1, p0, c2, l2-1, p6, c3, p4, c1, c0, a0 },
    keywordstyle=[4]\color{blue}\bfseries,
}

\begin{figure*}
\footnotesize
\begin{lstlisting}[basicstyle=\footnotesize\ttfamily]
Name: logistics-c4-s2-p9-a3 (logistics_a-3_c-4_s-2_p-9_t-5.pddl)
Objects: 
    a0, a1, a2, c0, c1, c2, c3, l0-0, l0-1, l1-0, l1-1, l2-0, l2-1, l3-0, l3-1, p0
p1, p2, p3, p4, p5, p6, p7, p8, t0, t1, t2, t3, t4
Initial: 
    package(p0), package(p1), package(p2), package(p3), package(p4), package(p5)
package(p6), package(p7), package(p8), truck(t0), truck(t1), truck(t2)
truck(t3), truck(t4), location(l0-0), location(l0-1), location(l1-0)
location(l1-1), location(l2-0), location(l2-1), location(l3-0), location(l3-1)
airplane(a0), airplane(a1), airplane(a2), city(c0), city(c1), city(c2), city(c3)
airport(l0-0), airport(l1-0), airport(l2-0), airport(l3-0), at(t0, l0-0), at(p6
l0-1), at(a0, l1-0), at(a1, l1-0), at(t1, l1-1), at(p3, l1-1), at(a2, l2-0)
at(t2, l2-0), at(t4, l2-0), at(p8, l2-0), at(p2, l3-0), at(p4, l3-0), at(p5
l3-0), at(t3, l3-1), at(p0, l3-1), at(p1, l3-1), at(p7, l3-1), in-city(l0-0, c0)
in-city(l0-1, c0), in-city(l1-0, c1), in-city(l1-1, c1), in-city(l2-0, c2)
in-city(l2-1, c2), in-city(l3-0, c3), in-city(l3-1, c3)
Goal: 
    at(p0, l1-1), at(p1, l2-0), at(p2, l3-0), at(p3, l1-1), at(p4, l1-1), at(p5
l3-0), at(p6, l3-0), at(p7, l1-0), at(p8, l3-0)

Plan has path-cycle: unchecked
Plan has subgoal-cycle: false
Primitive plan: 43
Plan: 5
1 drive-truck(t0, l0-0, l0-1, c0) -> load-truck(p6, t0, l0-1) -> drive-truck(t0, l0-1, l0-0, c0)
   ->unload-truck(p6, t0, l0-0) -> fly-airplane(a0, l1-0, l0-0) -> load-airplane(p6, a0, l0-0)
   ->fly-airplane(a0, l0-0, l3-0) -> unload-airplane(p6, a0, l3-0) -> load-truck(p7, t3, l3-1)
2 load-truck(p0, t3, l3-1) -> drive-truck(t3, l3-1, l3-0, c3) -> unload-truck(p0, t3, l3-0)
   ->load-airplane(p0, a0, l3-0) -> fly-airplane(a0, l3-0, l1-0) -> unload-airplane(p0, a0, l1-0)
   ->drive-truck(t1, l1-1, l1-0, c1) -> load-truck(p0, t1, l1-0) -> drive-truck(t1, l1-0, l1-1, c1)
   ->unload-truck(p0, t1, l1-1) -> drive-truck(t3, l3-0, l3-1, c3) -> load-truck(p1, t3, l3-1)
3 fly-airplane(a0, l1-0, l3-0) -> load-airplane(p4, a0, l3-0) -> fly-airplane(a0, l3-0, l1-0)
   ->unload-airplane(p4, a0, l1-0) -> drive-truck(t1, l1-1, l1-0, c1) -> load-truck(p4, t1, l1-0)
   ->drive-truck(t1, l1-0, l1-1, c1) -> unload-truck(p4, t1, l1-1) -> load-airplane(p8, a2, l2-0)
4 drive-truck(t3, l3-1, l3-0, c3) -> unload-truck(p1, t3, l3-0) -> fly-airplane(a0, l1-0, l3-0)
   ->load-airplane(p1, a0, l3-0) -> fly-airplane(a0, l3-0, l2-0) -> unload-airplane(p1, a0, l2-0)
   ->fly-airplane(a2, l2-0, l3-0) -> unload-airplane(p8, a2, l3-0)
5 unload-truck(p7, t3, l3-0) -> load-airplane(p7, a2, l3-0) -> fly-airplane(a2, l3-0, l1-0)
   ->unload-airplane(p7, a2, l1-0) -> fly-airplane(a0, l2-0, l1-0)
\end{lstlisting}
\end{figure*}

\clearpage

\lstset{
    basicstyle=\footnotesize\ttfamily,
    keywordstyle=\bfseries, % This will apply bold to all keywords
    % Define colors for different groups of keywords
    morekeywords=[1]{Domain},
    keywordstyle=[1]\color{red}\bfseries,
    morekeywords=[2]{Objects, Primitive, Goal, Initial, Plan, plan},
    keywordstyle=[2]\bfseries,
    morekeywords=[3]{UNLOAD, TRUCK, UNLOAD, AIRPLANE, LOAD, TRUCK, FLY, AIRPLANE, DRIVE, TRUCK, LOAD, AIRPLANE },
    keywordstyle=[3]\color{orange}\bfseries,
    morekeywords=[4]{t4, t2, p3, l1-0, l0-1, p2, l3-0, p5, p1, l3-1, p7, t1, t0, l2-0, a2, l0-0, p8, a1, t3, l1-1, p0, c2, l2-1, p6, c3, p4, c1, c0, a0 },
    keywordstyle=[4]\color{blue}\bfseries,
}

\begin{figure*}
\footnotesize
\begin{lstlisting}[basicstyle=\footnotesize\ttfamily]
Name: logistics-c4-s2-p9-a3 (logistics_a-3_c-4_s-2_p-9_t-5.pddl)
Objects: 
    a0, a1, a2, c0, c1, c2, c3, l0-0, l0-1, l1-0, l1-1, l2-0, l2-1, l3-0, l3-1, p0
p1, p2, p3, p4, p5, p6, p7, p8, t0, t1, t2, t3, t4
Initial: 
    package(p0), package(p1), package(p2), package(p3), package(p4), package(p5)
package(p6), package(p7), package(p8), truck(t0), truck(t1), truck(t2)
truck(t3), truck(t4), location(l0-0), location(l0-1), location(l1-0)
location(l1-1), location(l2-0), location(l2-1), location(l3-0), location(l3-1)
airplane(a0), airplane(a1), airplane(a2), city(c0), city(c1), city(c2), city(c3)
airport(l0-0), airport(l1-0), airport(l2-0), airport(l3-0), at(t0, l0-0), at(p6
l0-1), at(a0, l1-0), at(a1, l1-0), at(t1, l1-1), at(p3, l1-1), at(a2, l2-0)
at(t2, l2-0), at(t4, l2-0), at(p8, l2-0), at(p2, l3-0), at(p4, l3-0), at(p5
l3-0), at(t3, l3-1), at(p0, l3-1), at(p1, l3-1), at(p7, l3-1), in-city(l0-0, c0)
in-city(l0-1, c0), in-city(l1-0, c1), in-city(l1-1, c1), in-city(l2-0, c2)
in-city(l2-1, c2), in-city(l3-0, c3), in-city(l3-1, c3)
Goal: 
    at(p0, l1-1), at(p1, l2-0), at(p2, l3-0), at(p3, l1-1), at(p4, l1-1), at(p5
l3-0), at(p6, l3-0), at(p7, l1-0), at(p8, l3-0)

Plan has path-cycle: unchecked
Plan has subgoal-cycle: false
Primitive plan: 43
Plan: 5
1 drive-truck(t0, l0-0, l0-1, c0) -> load-truck(p6, t0, l0-1) -> drive-truck(t0, l0-1, l0-0, c0)
   ->unload-truck(p6, t0, l0-0) -> fly-airplane(a0, l1-0, l0-0) -> load-airplane(p6, a0, l0-0)
   ->fly-airplane(a0, l0-0, l3-0) -> unload-airplane(p6, a0, l3-0) -> load-truck(p7, t3, l3-1)
2 load-truck(p0, t3, l3-1) -> drive-truck(t3, l3-1, l3-0, c3) -> unload-truck(p0, t3, l3-0)
   ->load-airplane(p0, a0, l3-0) -> fly-airplane(a0, l3-0, l1-0) -> unload-airplane(p0, a0, l1-0)
   ->drive-truck(t1, l1-1, l1-0, c1) -> load-truck(p0, t1, l1-0) -> drive-truck(t1, l1-0, l1-1, c1)
   ->unload-truck(p0, t1, l1-1) -> drive-truck(t3, l3-0, l3-1, c3) -> load-truck(p1, t3, l3-1)
3 fly-airplane(a0, l1-0, l3-0) -> load-airplane(p4, a0, l3-0) -> fly-airplane(a0, l3-0, l1-0)
   ->unload-airplane(p4, a0, l1-0) -> drive-truck(t1, l1-1, l1-0, c1) -> load-truck(p4, t1, l1-0)
   ->drive-truck(t1, l1-0, l1-1, c1) -> unload-truck(p4, t1, l1-1) -> load-airplane(p8, a2, l2-0)
4 drive-truck(t3, l3-1, l3-0, c3) -> unload-truck(p1, t3, l3-0) -> fly-airplane(a0, l1-0, l3-0)
   ->load-airplane(p1, a0, l3-0) -> fly-airplane(a0, l3-0, l2-0) -> unload-airplane(p1, a0, l2-0)
   ->fly-airplane(a2, l2-0, l3-0) -> unload-airplane(p8, a2, l3-0)
5 unload-truck(p7, t3, l3-0) -> load-airplane(p7, a2, l3-0) -> fly-airplane(a2, l3-0, l1-0)
   ->unload-airplane(p7, a2, l1-0) -> fly-airplane(a0, l2-0, l1-0)
\end{lstlisting}
\end{figure*}

\clearpage
